# Supplementary material for: Communicating Inferred Goals with Passive Augmented Reality and Active Haptic Feedback
Source: arXiv:2109.01747 source file (2021-09-03)
Supplement: Supplementary file 1 [file interaction_time.pdf]

```
NEW FILE.
DATASET NAME DataSet1 WINDOW=FRONT.
GLM A1 B1 C1 D1
  /WSFACTOR=method 4 Polynomial
  /MEASURE=interaction_time
  /METHOD=SSTYPE(3)
  /PLOT=PROFILE(method) TYPE=BAR ERRORBAR=CI MEANREFERENCE=NO
  /EMMEANS=TABLES(method) COMPARE ADJ(LSD)
  /PRINT=DESCRIPTIVE
  /CRITERIA=ALPHA(.05)
  /WSDESIGN=method.
```

## General Linear Model

[DataSet1]

### Within-Subjects Factors

Measure: interaction_time

| method | Dependent Variable |
|---|---|
| 1 | A1 |
| 2 | B1 |
| 3 | C1 |
| 4 | D1 |

### Descriptive Statistics

| | Mean | Std. Deviation | N |
|---|---|---|---|
| A1 | 8.6800 | 1.81769 | 10 |
| B1 | 6.7600 | .74714 | 10 |
| C1 | 8.8700 | 2.56301 | 10 |
| D1 | 7.2800 | 1.52956 | 10 |

## Multivariate Tests[a]

| Effect | | Value | F | Hypothesis df | Error df | Sig. |
|---|---|---|---|---|---|---|
| method | Pillai's Trace | .705 | 5.580[b] | 3.000 | 7.000 | .028 |
| | Wilks' Lambda | .295 | 5.580[b] | 3.000 | 7.000 | .028 |
| | Hotelling's Trace | 2.391 | 5.580[b] | 3.000 | 7.000 | .028 |
| | Roy's Largest Root | 2.391 | 5.580[b] | 3.000 | 7.000 | .028 |

a. Design: Intercept
Within Subjects Design: method

b. Exact statistic

## Mauchly's Test of Sphericity[a]

Measure: interaction_time

| Within Subjects Effect | Mauchly's W | Approx. Chi-Square | df | Sig. | Epsilon[b] Greenhouse-Geisser |
|---|---|---|---|---|---|
| method | .152 | 14.556 | 5 | .013 | .573 |

## Mauchly's Test of Sphericity[a]

Measure: interaction_time

| Within Subjects Effect | Epsilon[b] Huynh-Feldt | Lower-bound |
|---|---|---|
| method | .696 | .333 |

Tests the null hypothesis that the error covariance matrix of the orthonormalized transformed dependent variables is proportional to an identity matrix.

a. Design: Intercept
Within Subjects Design: method

b. May be used to adjust the degrees of freedom for the averaged tests of significance. Corrected tests are displayed in the Tests of Within-Subjects Effects table.

## Tests of Within-Subjects Effects

Measure: interaction_time

| Source | | Type III Sum of Squares | df | Mean Square | F |
|---|---|---|---|---|---|
| method | Sphericity Assumed | 32.333 | 3 | 10.778 | 3.765 |
| | Greenhouse-Geisser | 32.333 | 1.720 | 18.794 | 3.765 |
| | Huynh-Feldt | 32.333 | 2.089 | 15.481 | 3.765 |
| | Lower-bound | 32.333 | 1.000 | 32.333 | 3.765 |
| Error(method) | Sphericity Assumed | 77.280 | 27 | 2.862 | |
| | Greenhouse-Geisser | 77.280 | 15.483 | 4.991 | |
| | Huynh-Feldt | 77.280 | 18.797 | 4.111 | |
| | Lower-bound | 77.280 | 9.000 | 8.587 | |

## Tests of Within-Subjects Effects

Measure: interaction_time

| Source | | Sig. |
|---|---|---|
| method | Sphericity Assumed | .022 |
| | Greenhouse-Geisser | .052 |
| | Huynh-Feldt | .041 |
| | Lower-bound | .084 |
| Error(method) | Sphericity Assumed | |
| | Greenhouse-Geisser | |
| | Huynh-Feldt | |
| | Lower-bound | |

## Tests of Within-Subjects Contrasts

Measure: interaction_time

| Source | method | Type III Sum of Squares | df | Mean Square | F | Sig. |
|---|---|---|---|---|---|---|
| method | Linear | 2.184 | 1 | 2.184 | 4.170 | .072 |
| | Quadratic | .272 | 1 | .272 | .060 | .812 |
| | Cubic | 29.876 | 1 | 29.876 | 8.520 | .017 |
| Error(method) | Linear | 4.713 | 9 | .524 | | |
| | Quadratic | 41.005 | 9 | 4.556 | | |
| | Cubic | 31.561 | 9 | 3.507 | | |

### Tests of Between-Subjects Effects

Measure: interaction_time

Transformed Variable: Average

| Source | Type III Sum of Squares | df | Mean Square | F | Sig. |
|---|---|---|---|---|---|
| Intercept | 2494.820 | 1 | 2494.820 | 596.257 | .000 |
| Error | 37.657 | 9 | 4.184 | | |

## Estimated Marginal Means

## method

### Estimates

Measure: interaction_time

| method | Mean | Std. Error | 95% Confidence Interval Lower Bound | 95% Confidence Interval Upper Bound |
|---|---|---|---|---|
| 1 | 8.680 | .575 | 7.380 | 9.980 |
| 2 | 6.760 | .236 | 6.226 | 7.294 |
| 3 | 8.870 | .810 | 7.037 | 10.703 |
| 4 | 7.280 | .484 | 6.186 | 8.374 |

### Pairwise Comparisons

Measure: interaction_time

| (I) method | (J) method | Mean Difference (I-J) | Std. Error | Sig.[b] | 95% Confidence Interval for Difference[b] Lower Bound | Upper Bound |
|---|---|---|---|---|---|---|
| 1 | 2 | 1.920* | .682 | .020 | .378 | 3.462 |
| | 3 | -.190 | .981 | .851 | -2.408 | 2.028 |
| | 4 | 1.400* | .311 | .001 | .697 | 2.103 |
| 2 | 1 | -1.920* | .682 | .020 | -3.462 | -.378 |
| | 3 | -2.110* | .842 | .034 | -4.015 | -.205 |
| | 4 | -.520 | .514 | .338 | -1.682 | .642 |
| 3 | 1 | .190 | .981 | .851 | -2.028 | 2.408 |
| | 2 | 2.110* | .842 | .034 | .205 | 4.015 |
| | 4 | 1.590 | .969 | .135 | -.601 | 3.781 |
| 4 | 1 | -1.400* | .311 | .001 | -2.103 | -.697 |
| | 2 | .520 | .514 | .338 | -.642 | 1.682 |
| | 3 | -1.590 | .969 | .135 | -3.781 | .601 |

Based on estimated marginal means

*. The mean difference is significant at the .05 level.

b. Adjustment for multiple comparisons: Least Significant Difference (equivalent to no adjustments).

### Multivariate Tests

| | Value | F | Hypothesis df | Error df | Sig. |
|---|---|---|---|---|---|
| Pillai's trace | .705 | 5.580[a] | 3.000 | 7.000 | .028 |
| Wilks' lambda | .295 | 5.580[a] | 3.000 | 7.000 | .028 |
| Hotelling's trace | 2.391 | 5.580[a] | 3.000 | 7.000 | .028 |
| Roy's largest root | 2.391 | 5.580[a] | 3.000 | 7.000 | .028 |

Each F tests the multivariate effect of method. These tests are based on the linearly independent pairwise comparisons among the estimated marginal means.

a. Exact statistic

## Profile Plots

Estimated Marginal Means of interaction_time

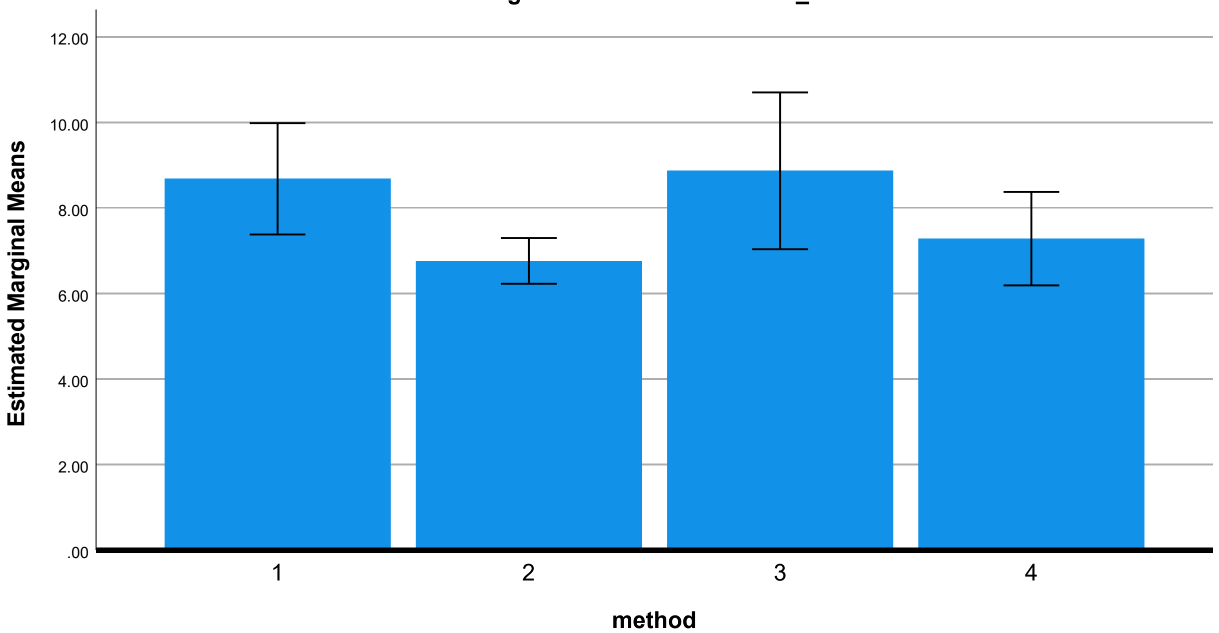


Error bars: 95% CI

```
GLM A2 B2 C2 D2
  /WSFACTOR=method 4 Polynomial
  /MEASURE=interaction_time
  /METHOD=SSTYPE(3)
  /PLOT=PROFILE(method) TYPE=BAR ERRORBAR=CI MEANREFERENCE=NO
  /EMMEANS=TABLES(method) COMPARE ADJ(LSD)
  /PRINT=DESCRIPTIVE
  /CRITERIA=ALPHA(.05)
  /WSDESIGN=method.
```

## General Linear Model

### Within-Subjects Factors

Measure: interaction_time

| method | Dependent Variable |
|---|---|
| 1 | A2 |
| 2 | B2 |
| 3 | C2 |
| 4 | D2 |

### Descriptive Statistics

| | Mean | Std. Deviation | N |
|---|---|---|---|
| A2 | 4.4300 | 1.70493 | 10 |
| B2 | 3.6600 | 1.21947 | 10 |
| C2 | 2.8700 | .62548 | 10 |
| D2 | 2.6100 | .67239 | 10 |

### Multivariate Tests[a]

| Effect | | Value | F | Hypothesis df | Error df | Sig. |
|---|---|---|---|---|---|---|
| method | Pillai's Trace | .624 | 3.878[b] | 3.000 | 7.000 | .064 |
| | Wilks' Lambda | .376 | 3.878[b] | 3.000 | 7.000 | .064 |
| | Hotelling's Trace | 1.662 | 3.878[b] | 3.000 | 7.000 | .064 |
| | Roy's Largest Root | 1.662 | 3.878[b] | 3.000 | 7.000 | .064 |

a. Design: Intercept
Within Subjects Design: method

b. Exact statistic

### Mauchly's Test of Sphericity[a]

Measure: interaction_time

| | | | | | Epsilon[b] |
|---|---|---|---|---|---|
| Within Subjects Effect | Mauchly's W | Approx. Chi-Square | df | Sig. | Greenhouse-Geisser |
| method | .378 | 7.506 | 5 | .189 | .726 |

### Mauchly's Test of Sphericity[a]

Measure: interaction_time

| | Epsilon[b] | |
|---|---|---|
| Within Subjects Effect | Huynh-Feldt | Lower-bound |
| method | .966 | .333 |

Tests the null hypothesis that the error covariance matrix of the orthonormalized transformed dependent variables is proportional to an identity matrix.

a. Design: Intercept
Within Subjects Design: method

b. May be used to adjust the degrees of freedom for the averaged tests of significance. Corrected tests are displayed in the Tests of Within-Subjects Effects table.

## Tests of Within-Subjects Effects

Measure: interaction_time

| Source | | Type III Sum of Squares | df | Mean Square | F |
|---|---|---|---|---|---|
| method | Sphericity Assumed | 20.333 | 3 | 6.778 | 5.422 |
| | Greenhouse-Geisser | 20.333 | 2.177 | 9.340 | 5.422 |
| | Huynh-Feldt | 20.333 | 2.898 | 7.017 | 5.422 |
| | Lower-bound | 20.333 | 1.000 | 20.333 | 5.422 |
| Error(method) | Sphericity Assumed | 33.750 | 27 | 1.250 | |
| | Greenhouse-Geisser | 33.750 | 19.593 | 1.723 | |
| | Huynh-Feldt | 33.750 | 26.078 | 1.294 | |
| | Lower-bound | 33.750 | 9.000 | 3.750 | |

## Tests of Within-Subjects Effects

Measure: interaction_time

| Source | | Sig. |
|---|---|---|
| method | Sphericity Assumed | .005 |
| | Greenhouse-Geisser | .012 |
| | Huynh-Feldt | .005 |
| | Lower-bound | .045 |
| Error(method) | Sphericity Assumed | |
| | Greenhouse-Geisser | |
| | Huynh-Feldt | |
| | Lower-bound | |

## Tests of Within-Subjects Contrasts

Measure: interaction_time

| Source | method | Type III Sum of Squares | df | Mean Square | F | Sig. |
|---|---|---|---|---|---|---|
| method | Linear | 19.531 | 1 | 19.531 | 13.262 | .005 |
| | Quadratic | .650 | 1 | .650 | .926 | .361 |
| | Cubic | .151 | 1 | .151 | .096 | .764 |
| Error(method) | Linear | 13.254 | 9 | 1.473 | | |
| | Quadratic | 6.317 | 9 | .702 | | |
| | Cubic | 14.178 | 9 | 1.575 | | |

## Tests of Between-Subjects Effects

Measure: interaction_time

Transformed Variable: Average

| Source | Type III Sum of Squares | df | Mean Square | F | Sig. |
|---|---|---|---|---|---|
| Intercept | 460.362 | 1 | 460.362 | 309.539 | .000 |
| Error | 13.385 | 9 | 1.487 | | |

## Estimated Marginal Means

### method

## Estimates

Measure: interaction_time

| method | Mean | Std. Error | 95% Confidence Interval | |
|---|---|---|---|---|
| | | | Lower Bound | Upper Bound |
| 1 | 4.430 | .539 | 3.210 | 5.650 |
| 2 | 3.660 | .386 | 2.788 | 4.532 |
| 3 | 2.870 | .198 | 2.423 | 3.317 |
| 4 | 2.610 | .213 | 2.129 | 3.091 |

## Pairwise Comparisons

Measure: interaction_time

| (I) method | (J) method | Mean Difference (I-J) | Std. Error | Sig.[b] | 95% Confidence Interval for Difference[b] Lower Bound | Upper Bound |
|---|---|---|---|---|---|---|
| 1 | 2 | .770 | .623 | .248 | -.640 | 2.180 |
| | 3 | 1.560* | .509 | .014 | .408 | 2.712 |
| | 4 | 1.820* | .561 | .010 | .551 | 3.089 |
| 2 | 1 | -.770 | .623 | .248 | -2.180 | .640 |
| | 3 | .790 | .543 | .180 | -.439 | 2.019 |
| | 4 | 1.050* | .394 | .026 | .158 | 1.942 |
| 3 | 1 | -1.560* | .509 | .014 | -2.712 | -.408 |
| | 2 | -.790 | .543 | .180 | -2.019 | .439 |
| | 4 | .260 | .295 | .401 | -.407 | .927 |
| 4 | 1 | -1.820* | .561 | .010 | -3.089 | -.551 |
| | 2 | -1.050* | .394 | .026 | -1.942 | -.158 |
| | 3 | -.260 | .295 | .401 | -.927 | .407 |

Based on estimated marginal means

*. The mean difference is significant at the .05 level.

b. Adjustment for multiple comparisons: Least Significant Difference (equivalent to no adjustments).

## Multivariate Tests

| | Value | F | Hypothesis df | Error df | Sig. |
|---|---|---|---|---|---|
| Pillai's trace | .624 | 3.878[a] | 3.000 | 7.000 | .064 |
| Wilks' lambda | .376 | 3.878[a] | 3.000 | 7.000 | .064 |
| Hotelling's trace | 1.662 | 3.878[a] | 3.000 | 7.000 | .064 |
| Roy's largest root | 1.662 | 3.878[a] | 3.000 | 7.000 | .064 |

Each F tests the multivariate effect of method. These tests are based on the linearly independent pairwise comparisons among the estimated marginal means.

a. Exact statistic

## Profile Plots

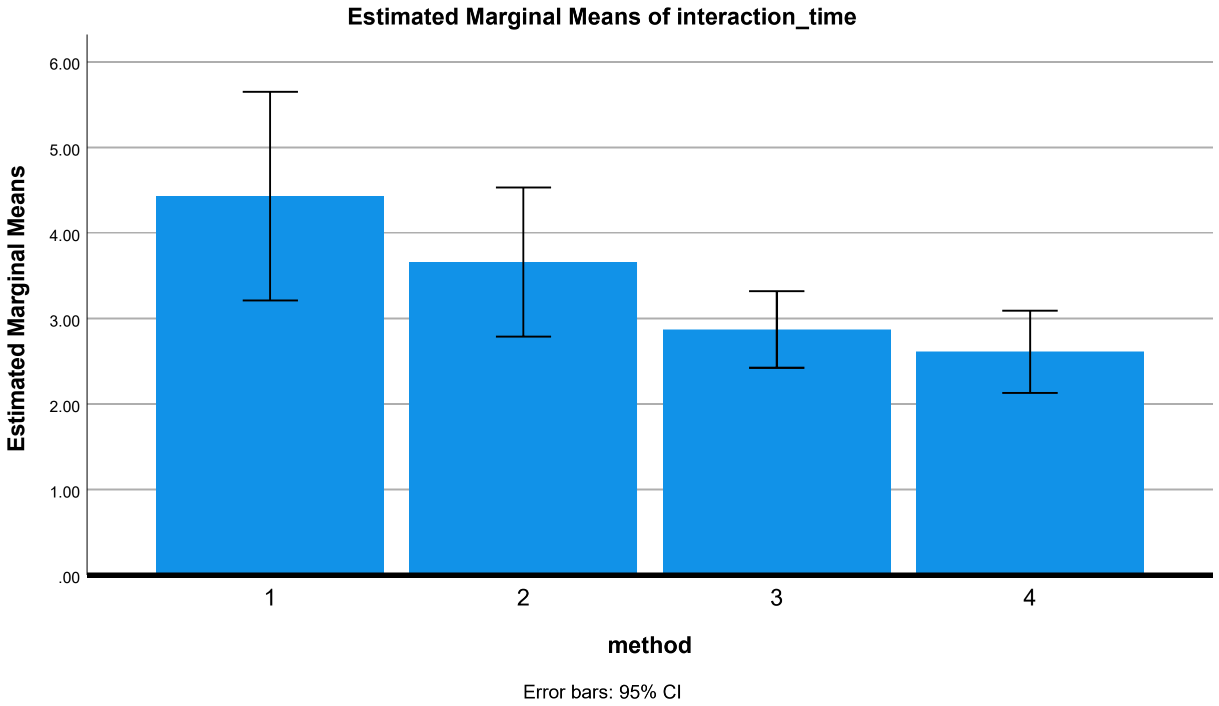


```
GLM A3 B3 C3 D3
  /WSFACTOR=method 4 Polynomial
  /MEASURE=interaction_time
  /METHOD=SSTYPE(3)
  /PLOT=PROFILE(method) TYPE=BAR ERRORBAR=CI MEANREFERENCE=NO
  /EMMEANS=TABLES(method) COMPARE ADJ(LSD)
  /PRINT=DESCRIPTIVE
  /CRITERIA=ALPHA(.05)
  /WSDESIGN=method.
```

## General Linear Model

### Within-Subjects Factors

Measure: interaction_time

| method | Dependent Variable |
|---|---|
| 1 | A3 |
| 2 | B3 |
| 3 | C3 |
| 4 | D3 |

### Descriptive Statistics

| | Mean | Std. Deviation | N |
|---|---|---|---|
| A3 | 2.5300 | .96845 | 10 |
| B3 | 3.0000 | 1.02956 | 10 |
| C3 | 2.5800 | 1.27436 | 10 |
| D3 | 1.7300 | .73492 | 10 |

### Multivariate Tests[a]

| Effect | | Value | F | Hypothesis df | Error df | Sig. |
|---|---|---|---|---|---|---|
| method | Pillai's Trace | .736 | 6.506[b] | 3.000 | 7.000 | .020 |
| | Wilks' Lambda | .264 | 6.506[b] | 3.000 | 7.000 | .020 |
| | Hotelling's Trace | 2.788 | 6.506[b] | 3.000 | 7.000 | .020 |
| | Roy's Largest Root | 2.788 | 6.506[b] | 3.000 | 7.000 | .020 |

a. Design: Intercept
Within Subjects Design: method

b. Exact statistic

### Mauchly's Test of Sphericity[a]

Measure: interaction_time

| Within Subjects Effect | Mauchly's W | Approx. Chi-Square | df | Sig. | Epsilon[b] Greenhouse-Geisser |
|---|---|---|---|---|---|
| method | .236 | 11.135 | 5 | .050 | .532 |

### Mauchly's Test of Sphericity[a]

Measure: interaction_time

| Within Subjects Effect | Epsilon[b] Huynh-Feldt | Lower-bound |
|---|---|---|
| method | .628 | .333 |

Tests the null hypothesis that the error covariance matrix of the orthonormalized transformed dependent variables is proportional to an identity matrix.

a. Design: Intercept
Within Subjects Design: method

b. May be used to adjust the degrees of freedom for the averaged tests of significance. Corrected tests are displayed in the Tests of Within-Subjects Effects table.

**Tests of Within-Subjects Effects**

Measure: interaction_time

| Source | | Type III Sum of Squares | df | Mean Square | F |
|---|---|---|---|---|---|
| method | Sphericity Assumed | 8.438 | 3 | 2.813 | 2.649 |
| | Greenhouse-Geisser | 8.438 | 1.595 | 5.289 | 2.649 |
| | Huynh-Feldt | 8.438 | 1.885 | 4.477 | 2.649 |
| | Lower-bound | 8.438 | 1.000 | 8.438 | 2.649 |
| Error(method) | Sphericity Assumed | 28.672 | 27 | 1.062 | |
| | Greenhouse-Geisser | 28.672 | 14.359 | 1.997 | |
| | Huynh-Feldt | 28.672 | 16.961 | 1.690 | |
| | Lower-bound | 28.672 | 9.000 | 3.186 | |

**Tests of Within-Subjects Effects**

Measure: interaction_time

| Source | | Sig. |
|---|---|---|
| method | Sphericity Assumed | .069 |
| | Greenhouse-Geisser | .113 |
| | Huynh-Feldt | .102 |
| | Lower-bound | .138 |
| Error(method) | Sphericity Assumed | |
| | Greenhouse-Geisser | |
| | Huynh-Feldt | |
| | Lower-bound | |

**Tests of Within-Subjects Contrasts**

Measure: interaction_time

| Source | method | Type III Sum of Squares | df | Mean Square | F | Sig. |
|---|---|---|---|---|---|---|
| method | Linear | 3.976 | 1 | 3.976 | 3.236 | .106 |
| | Quadratic | 4.356 | 1 | 4.356 | 6.731 | .029 |
| | Cubic | .106 | 1 | .106 | .081 | .783 |
| Error(method) | Linear | 11.058 | 9 | 1.229 | | |
| | Quadratic | 5.824 | 9 | .647 | | |
| | Cubic | 11.790 | 9 | 1.310 | | |

## Tests of Between-Subjects Effects

Measure: interaction_time

Transformed Variable: Average

| Source | Type III Sum of Squares | df | Mean Square | F | Sig. |
|---|---|---|---|---|---|
| Intercept | 242.064 | 1 | 242.064 | 247.960 | .000 |
| Error | 8.786 | 9 | .976 | | |

# Estimated Marginal Means

## method

## Estimates

Measure: interaction_time

| method | Mean | Std. Error | 95% Confidence Interval | |
|---|---|---|---|---|
| | | | Lower Bound | Upper Bound |
| 1 | 2.530 | .306 | 1.837 | 3.223 |
| 2 | 3.000 | .326 | 2.263 | 3.737 |
| 3 | 2.580 | .403 | 1.668 | 3.492 |
| 4 | 1.730 | .232 | 1.204 | 2.256 |

## Pairwise Comparisons

Measure: interaction_time

| (I) method | (J) method | Mean Difference (I-J) | Std. Error | Sig.[b] | 95% Confidence Interval for Difference[b] Lower Bound | Upper Bound |
|---|---|---|---|---|---|---|
| 1 | 2 | -.470 | .302 | .154 | -1.154 | .214 |
| | 3 | -.050 | .623 | .938 | -1.458 | 1.358 |
| | 4 | .800 | .357 | .052 | -.009 | 1.609 |
| 2 | 1 | .470 | .302 | .154 | -.214 | 1.154 |
| | 3 | .420 | .616 | .513 | -.974 | 1.814 |
| | 4 | 1.270* | .388 | .010 | .393 | 2.147 |
| 3 | 1 | .050 | .623 | .938 | -1.358 | 1.458 |
| | 2 | -.420 | .616 | .513 | -1.814 | .974 |
| | 4 | .850* | .371 | .048 | .012 | 1.688 |
| 4 | 1 | -.800 | .357 | .052 | -1.609 | .009 |
| | 2 | -1.270* | .388 | .010 | -2.147 | -.393 |
| | 3 | -.850* | .371 | .048 | -1.688 | -.012 |

Based on estimated marginal means

*. The mean difference is significant at the .05 level.

b. Adjustment for multiple comparisons: Least Significant Difference (equivalent to no adjustments).

## Multivariate Tests

| | Value | F | Hypothesis df | Error df | Sig. |
|---|---|---|---|---|---|
| Pillai's trace | .736 | 6.506[a] | 3.000 | 7.000 | .020 |
| Wilks' lambda | .264 | 6.506[a] | 3.000 | 7.000 | .020 |
| Hotelling's trace | 2.788 | 6.506[a] | 3.000 | 7.000 | .020 |
| Roy's largest root | 2.788 | 6.506[a] | 3.000 | 7.000 | .020 |

Each F tests the multivariate effect of method. These tests are based on the linearly independent pairwise comparisons among the estimated marginal means.

a. Exact statistic

## Profile Plots

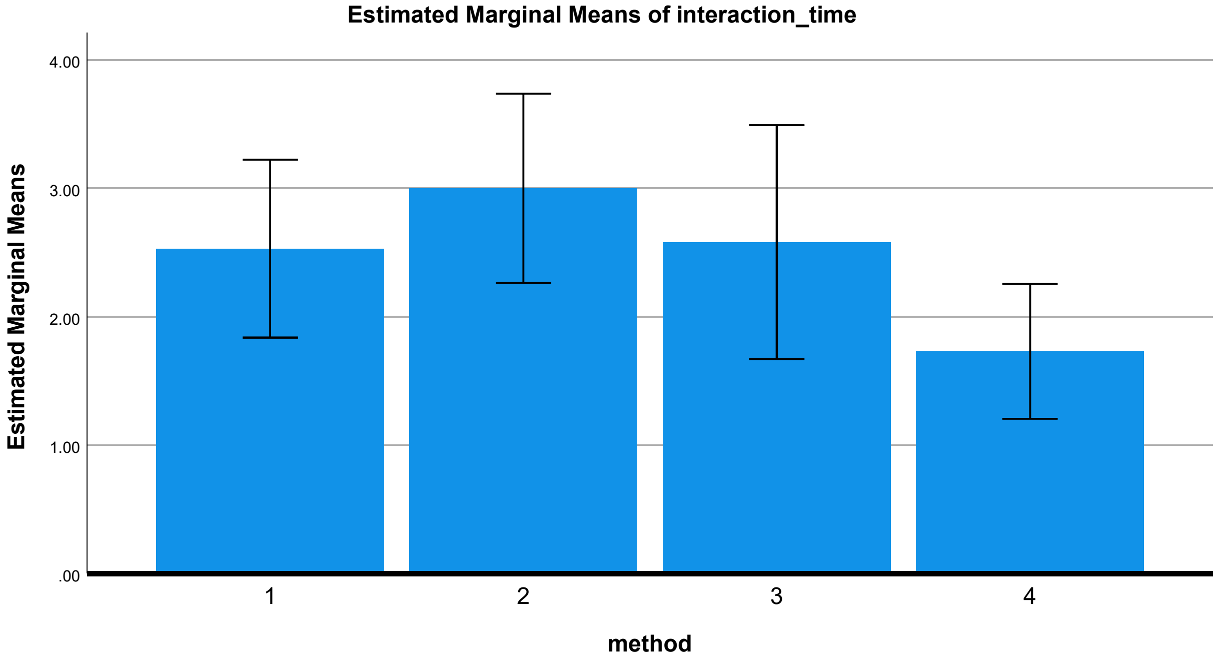

Error bars: 95% CI

```
GLM A4 B4 C4 D4
  /WSFACTOR=method 4 Polynomial
  /MEASURE=interaction_time
  /METHOD=SSTYPE(3)
  /PLOT=PROFILE(method) TYPE=BAR ERRORBAR=CI MEANREFERENCE=NO
  /EMMEANS=TABLES(method) COMPARE ADJ(LSD)
  /PRINT=DESCRIPTIVE
  /CRITERIA=ALPHA(.05)
  /WSDESIGN=method.
```

## General Linear Model

### Within-Subjects Factors

Measure: interaction_time

| method | Dependent Variable |
|---|---|
| 1 | A4 |
| 2 | B4 |
| 3 | C4 |
| 4 | D4 |

### Descriptive Statistics

| | Mean | Std. Deviation | N |
|---|---|---|---|
| A4 | 3.3100 | 1.74193 | 10 |
| B4 | 3.9000 | .92014 | 10 |
| C4 | 3.1200 | .58841 | 10 |
| D4 | 3.3100 | .67404 | 10 |

### Multivariate Tests[a]

| Effect | | Value | F | Hypothesis df | Error df | Sig. |
|---|---|---|---|---|---|---|
| method | Pillai's Trace | .643 | 4.194[b] | 3.000 | 7.000 | .054 |
| | Wilks' Lambda | .357 | 4.194[b] | 3.000 | 7.000 | .054 |
| | Hotelling's Trace | 1.798 | 4.194[b] | 3.000 | 7.000 | .054 |
| | Roy's Largest Root | 1.798 | 4.194[b] | 3.000 | 7.000 | .054 |

a. Design: Intercept
Within Subjects Design: method

b. Exact statistic

### Mauchly's Test of Sphericity[a]

Measure: interaction_time

| Within Subjects Effect | Mauchly's W | Approx. Chi-Square | df | Sig. | Epsilon[b] Greenhouse-Geisser |
|---|---|---|---|---|---|
| method | .057 | 22.092 | 5 | .001 | .435 |

### Mauchly's Test of Sphericity[a]

Measure: interaction_time

| Within Subjects Effect | Epsilon[b] Huynh-Feldt | Lower-bound |
|---|---|---|
| method | .479 | .333 |

Tests the null hypothesis that the error covariance matrix of the orthonormalized transformed dependent variables is proportional to an identity matrix.

a. Design: Intercept
Within Subjects Design: method

b. May be used to adjust the degrees of freedom for the averaged tests of significance. Corrected tests are displayed in the Tests of Within-Subjects Effects table.

## Tests of Within-Subjects Effects

Measure: interaction_time

| Source | | Type III Sum of Squares | df | Mean Square | F |
|---|---|---|---|---|---|
| method | Sphericity Assumed | 3.442 | 3 | 1.147 | 1.373 |
| | Greenhouse-Geisser | 3.442 | 1.306 | 2.635 | 1.373 |
| | Huynh-Feldt | 3.442 | 1.438 | 2.393 | 1.373 |
| | Lower-bound | 3.442 | 1.000 | 3.442 | 1.373 |
| Error(method) | Sphericity Assumed | 22.568 | 27 | .836 | |
| | Greenhouse-Geisser | 22.568 | 11.758 | 1.919 | |
| | Huynh-Feldt | 22.568 | 12.943 | 1.744 | |
| | Lower-bound | 22.568 | 9.000 | 2.508 | |

## Tests of Within-Subjects Effects

Measure: interaction_time

| Source | | Sig. |
|---|---|---|
| method | Sphericity Assumed | .272 |
| | Greenhouse-Geisser | .277 |
| | Huynh-Feldt | .278 |
| | Lower-bound | .271 |
| Error(method) | Sphericity Assumed | |
| | Greenhouse-Geisser | |
| | Huynh-Feldt | |
| | Lower-bound | |

## Tests of Within-Subjects Contrasts

Measure: interaction_time

| Source | method | Type III Sum of Squares | df | Mean Square | F | Sig. |
|---|---|---|---|---|---|---|
| method | Linear | .304 | 1 | .304 | .262 | .621 |
| | Quadratic | .400 | 1 | .400 | .371 | .558 |
| | Cubic | 2.738 | 1 | 2.738 | 10.292 | .011 |
| Error(method) | Linear | 10.464 | 9 | 1.163 | | |
| | Quadratic | 9.710 | 9 | 1.079 | | |
| | Cubic | 2.394 | 9 | .266 | | |

### Tests of Between-Subjects Effects

Measure: interaction_time

Transformed Variable: Average

| Source | Type III Sum of Squares | df | Mean Square | F | Sig. |
|---|---|---|---|---|---|
| Intercept | 465.124 | 1 | 465.124 | 213.948 | .000 |
| Error | 19.566 | 9 | 2.174 | | |

## Estimated Marginal Means

## method

### Estimates

Measure: interaction_time

| method | Mean | Std. Error | 95% Confidence Interval | |
|---|---|---|---|---|
| | | | Lower Bound | Upper Bound |
| 1 | 3.310 | .551 | 2.064 | 4.556 |
| 2 | 3.900 | .291 | 3.242 | 4.558 |
| 3 | 3.120 | .186 | 2.699 | 3.541 |
| 4 | 3.310 | .213 | 2.828 | 3.792 |

## Pairwise Comparisons

Measure: interaction_time

| (I) method | (J) method | Mean Difference (I-J) | Std. Error | Sig.[b] | 95% Confidence Interval for Difference[b] | |
|---|---|---|---|---|---|---|
| | | | | | Lower Bound | Upper Bound |
| 1 | 2 | -.590 | .570 | .328 | -1.880 | .700 |
| | 3 | .190 | .569 | .746 | -1.097 | 1.477 |
| | 4 | .000 | .493 | 1.000 | -1.115 | 1.115 |
| 2 | 1 | .590 | .570 | .328 | -.700 | 1.880 |
| | 3 | .780* | .206 | .004 | .313 | 1.247 |
| | 4 | .590* | .226 | .028 | .079 | 1.101 |
| 3 | 1 | -.190 | .569 | .746 | -1.477 | 1.097 |
| | 2 | -.780* | .206 | .004 | -1.247 | -.313 |
| | 4 | -.190 | .132 | .184 | -.489 | .109 |
| 4 | 1 | .000 | .493 | 1.000 | -1.115 | 1.115 |
| | 2 | -.590* | .226 | .028 | -1.101 | -.079 |
| | 3 | .190 | .132 | .184 | -.109 | .489 |

Based on estimated marginal means

*. The mean difference is significant at the .05 level.

b. Adjustment for multiple comparisons: Least Significant Difference (equivalent to no adjustments).

## Multivariate Tests

| | Value | F | Hypothesis df | Error df | Sig. |
|---|---|---|---|---|---|
| Pillai's trace | .643 | 4.194[a] | 3.000 | 7.000 | .054 |
| Wilks' lambda | .357 | 4.194[a] | 3.000 | 7.000 | .054 |
| Hotelling's trace | 1.798 | 4.194[a] | 3.000 | 7.000 | .054 |
| Roy's largest root | 1.798 | 4.194[a] | 3.000 | 7.000 | .054 |

Each F tests the multivariate effect of method. These tests are based on the linearly independent pairwise comparisons among the estimated marginal means.

a. Exact statistic

## Profile Plots

Estimated Marginal Means of interaction_time

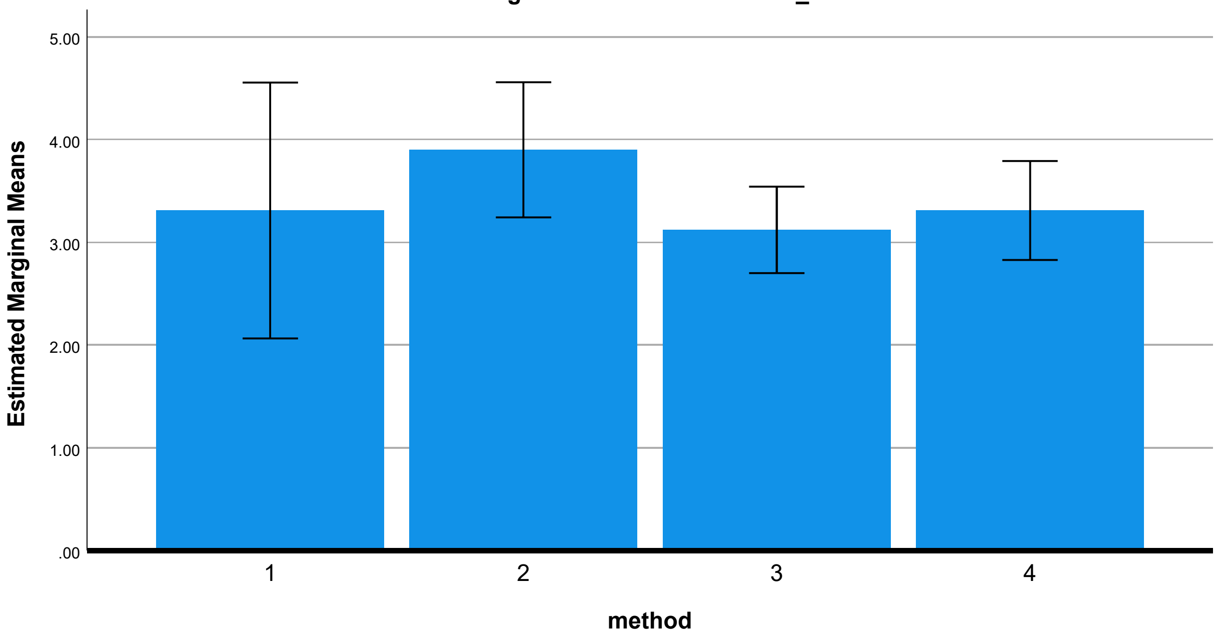


Error bars: 95% CI

```
GLM A5 B5 C5 D5
  /WSFACTOR=method 4 Polynomial
  /MEASURE=interaction_time
  /METHOD=SSTYPE(3)
  /PLOT=PROFILE(method) TYPE=BAR ERRORBAR=CI MEANREFERENCE=NO
  /EMMEANS=TABLES(method) COMPARE ADJ(LSD)
  /PRINT=DESCRIPTIVE
  /CRITERIA=ALPHA(.05)
  /WSDESIGN=method.
```

## General Linear Model

### Within-Subjects Factors

Measure: interaction_time

| method | Dependent Variable |
|---|---|
| 1 | A5 |
| 2 | B5 |
| 3 | C5 |
| 4 | D5 |

## Descriptive Statistics

| | Mean | Std. Deviation | N |
|---|---|---|---|
| A5 | 4.8200 | 1.02068 | 10 |
| B5 | 4.4900 | 1.18364 | 10 |
| C5 | 5.2000 | 3.91805 | 10 |
| D5 | 2.9300 | .97531 | 10 |

## Multivariate Tests[a]

| Effect | | Value | F | Hypothesis df | Error df | Sig. |
|---|---|---|---|---|---|---|
| method | Pillai's Trace | .780 | 8.267[b] | 3.000 | 7.000 | .011 |
| | Wilks' Lambda | .220 | 8.267[b] | 3.000 | 7.000 | .011 |
| | Hotelling's Trace | 3.543 | 8.267[b] | 3.000 | 7.000 | .011 |
| | Roy's Largest Root | 3.543 | 8.267[b] | 3.000 | 7.000 | .011 |

a. Design: Intercept
Within Subjects Design: method

b. Exact statistic

## Mauchly's Test of Sphericity[a]

Measure: interaction_time

| | | | | | Epsilon[b] |
|---|---|---|---|---|---|
| Within Subjects Effect | Mauchly's W | Approx. Chi-Square | df | Sig. | Greenhouse-Geisser |
| method | .030 | 27.004 | 5 | .000 | .385 |

## Mauchly's Test of Sphericity[a]

Measure: interaction_time

| | Epsilon[b] | |
|---|---|---|
| Within Subjects Effect | Huynh-Feldt | Lower-bound |
| method | .406 | .333 |

Tests the null hypothesis that the error covariance matrix of the orthonormalized transformed dependent variables is proportional to an identity matrix.

a. Design: Intercept
Within Subjects Design: method

b. May be used to adjust the degrees of freedom for the averaged tests of significance. Corrected tests are displayed in the Tests of Within-Subjects Effects table.

## Tests of Within-Subjects Effects

Measure: interaction_time

| Source | | Type III Sum of Squares | df | Mean Square | F |
|---|---|---|---|---|---|
| method | Sphericity Assumed | 29.790 | 3 | 9.930 | 1.791 |
| | Greenhouse-Geisser | 29.790 | 1.155 | 25.790 | 1.791 |
| | Huynh-Feldt | 29.790 | 1.217 | 24.468 | 1.791 |
| | Lower-bound | 29.790 | 1.000 | 29.790 | 1.791 |
| Error(method) | Sphericity Assumed | 149.670 | 27 | 5.543 | |
| | Greenhouse-Geisser | 149.670 | 10.396 | 14.397 | |
| | Huynh-Feldt | 149.670 | 10.957 | 13.659 | |
| | Lower-bound | 149.670 | 9.000 | 16.630 | |

## Tests of Within-Subjects Effects

Measure: interaction_time

| Source | | Sig. |
|---|---|---|
| method | Sphericity Assumed | .173 |
| | Greenhouse-Geisser | .212 |
| | Huynh-Feldt | .211 |
| | Lower-bound | .214 |
| Error(method) | Sphericity Assumed | |
| | Greenhouse-Geisser | |
| | Huynh-Feldt | |
| | Lower-bound | |

## Tests of Within-Subjects Contrasts

Measure: interaction_time

| Source | method | Type III Sum of Squares | df | Mean Square | F | Sig. |
|---|---|---|---|---|---|---|
| method | Linear | 12.301 | 1 | 12.301 | 6.009 | .037 |
| | Quadratic | 9.409 | 1 | 9.409 | 1.906 | .201 |
| | Cubic | 8.080 | 1 | 8.080 | .838 | .384 |
| Error(method) | Linear | 18.423 | 9 | 2.047 | | |
| | Quadratic | 44.421 | 9 | 4.936 | | |
| | Cubic | 86.826 | 9 | 9.647 | | |

## Tests of Between-Subjects Effects

Measure: interaction_time

Transformed Variable: Average

| Source | Type III Sum of Squares | df | Mean Square | F | Sig. |
|---|---|---|---|---|---|
| Intercept | 760.384 | 1 | 760.384 | 359.501 | .000 |
| Error | 19.036 | 9 | 2.115 | | |

## Estimated Marginal Means

## method

## Estimates

Measure: interaction_time

| method | Mean | Std. Error | 95% Confidence Interval | |
|---|---|---|---|---|
| | | | Lower Bound | Upper Bound |
| 1 | 4.820 | .323 | 4.090 | 5.550 |
| 2 | 4.490 | .374 | 3.643 | 5.337 |
| 3 | 5.200 | 1.239 | 2.397 | 8.003 |
| 4 | 2.930 | .308 | 2.232 | 3.628 |

## Pairwise Comparisons

Measure: interaction_time

| (I) method | (J) method | Mean Difference (I-J) | Std. Error | Sig.[b] | 95% Confidence Interval for Difference[b] Lower Bound | Upper Bound |
|---|---|---|---|---|---|---|
| 1 | 2 | .330 | .308 | .312 | -.367 | 1.027 |
| | 3 | -.380 | 1.460 | .800 | -3.682 | 2.922 |
| | 4 | 1.890* | .365 | .001 | 1.065 | 2.715 |
| 2 | 1 | -.330 | .308 | .312 | -1.027 | .367 |
| | 3 | -.710 | 1.485 | .644 | -4.070 | 2.650 |
| | 4 | 1.560* | .376 | .002 | .709 | 2.411 |
| 3 | 1 | .380 | 1.460 | .800 | -2.922 | 3.682 |
| | 2 | .710 | 1.485 | .644 | -2.650 | 4.070 |
| | 4 | 2.270 | 1.395 | .138 | -.886 | 5.426 |
| 4 | 1 | -1.890* | .365 | .001 | -2.715 | -1.065 |
| | 2 | -1.560* | .376 | .002 | -2.411 | -.709 |
| | 3 | -2.270 | 1.395 | .138 | -5.426 | .886 |

Based on estimated marginal means

*. The mean difference is significant at the .05 level.

b. Adjustment for multiple comparisons: Least Significant Difference (equivalent to no adjustments).

## Multivariate Tests

| | Value | F | Hypothesis df | Error df | Sig. |
|---|---|---|---|---|---|
| Pillai's trace | .780 | 8.267[a] | 3.000 | 7.000 | .011 |
| Wilks' lambda | .220 | 8.267[a] | 3.000 | 7.000 | .011 |
| Hotelling's trace | 3.543 | 8.267[a] | 3.000 | 7.000 | .011 |
| Roy's largest root | 3.543 | 8.267[a] | 3.000 | 7.000 | .011 |

Each F tests the multivariate effect of method. These tests are based on the linearly independent pairwise comparisons among the estimated marginal means.

a. Exact statistic

## Profile Plots

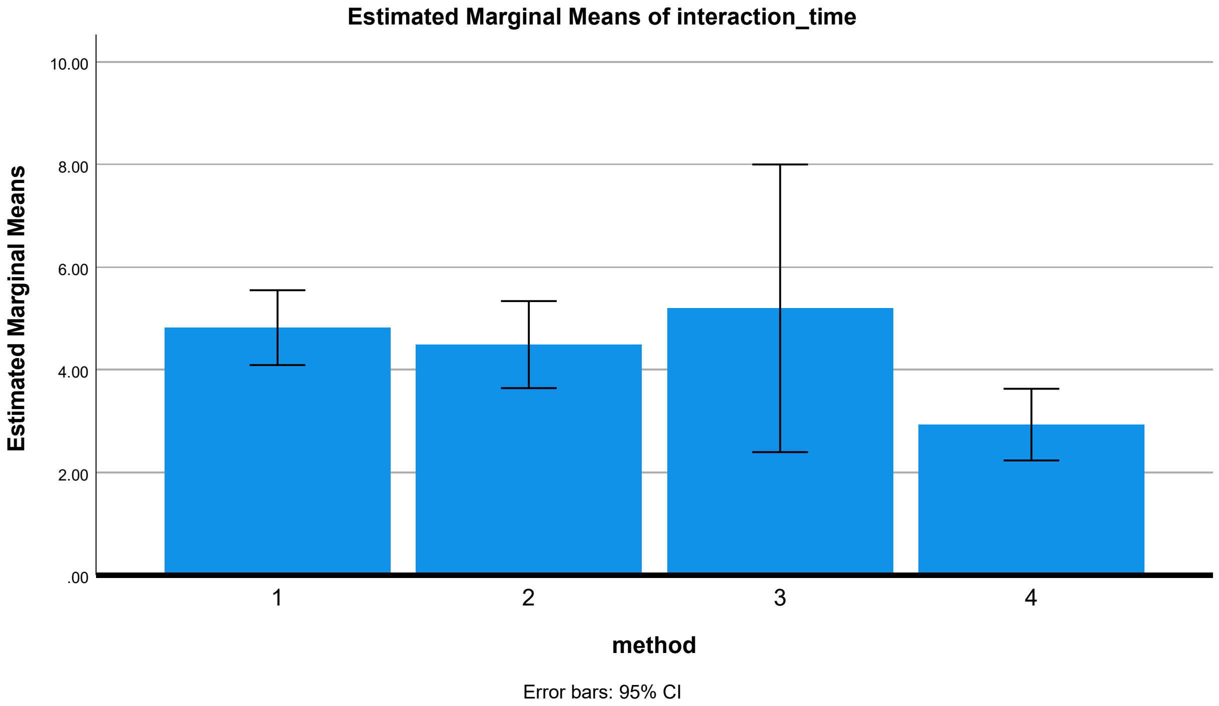
Estimated Marginal Means of interaction_time
Estimated Marginal Means
10.00
8.00
6.00
4.00
2.00
.00
1
2
3
4
method
Error bars: 95% CI
