# Supplementary material for: Communicating Inferred Goals with Passive Augmented Reality and Active Haptic Feedback
Source: arXiv:2109.01747 source file (2021-09-03)

```

GLM A B C D
  /WSFACTOR=method 4 Polynomial
  /MEASURE=score
  /METHOD=SSTYPE(3)
  /PLOT=PROFILE(method) TYPE=BAR ERRORBAR=CI MEANREFERENCE=NO
  /EMMEANS=TABLES(method) COMPARE ADJ(LSD)
  /PRINT=DESCRIPTIVE
  /CRITERIA=ALPHA(.05)
  /WSDESIGN=method.

```

## General Linear Model

### Within-Subjects Factors

Measure: score

| method | Dependent<br>Variable |
|--------|-----------------------|
| 1      | A                     |
| 2      | B                     |
| 3      | C                     |
| 4      | D                     |

### Descriptive Statistics

|   | Mean    | Std. Deviation | N  |
|---|---------|----------------|----|
| A | 19.5536 | 3.58165        | 10 |
| B | 23.0863 | 2.73387        | 10 |
| C | 19.7239 | 2.85398        | 10 |
| D | 22.9412 | 3.62776        | 10 |

### Multivariate Tests<sup>a</sup>

| Effect |                    | Value | F                   | Hypothesis df | Error df | Sig. |
|--------|--------------------|-------|---------------------|---------------|----------|------|
| method | Pillai's Trace     | .866  | 15.029 <sup>b</sup> | 3.000         | 7.000    | .002 |
|        | Wilks' Lambda      | .134  | 15.029 <sup>b</sup> | 3.000         | 7.000    | .002 |
|        | Hotelling's Trace  | 6.441 | 15.029 <sup>b</sup> | 3.000         | 7.000    | .002 |
|        | Roy's Largest Root | 6.441 | 15.029 <sup>b</sup> | 3.000         | 7.000    | .002 |

a. Design: Intercept  
Within Subjects Design: method

b. Exact statistic

### Mauchly's Test of Sphericity<sup>a</sup>

Measure: score

| Within Subjects Effect | Mauchly's W | Approx. Chi-Square | df | Sig. | Epsilon <sup>b</sup><br>Greenhouse-Geisser |
|------------------------|-------------|--------------------|----|------|--------------------------------------------|
| method                 | .350        | 8.117              | 5  | .153 | .630                                       |

### Mauchly's Test of Sphericity<sup>a</sup>

Measure: score

| Within Subjects Effect | Epsilon <sup>b</sup> |             |
|------------------------|----------------------|-------------|
|                        | Huynh-Feldt          | Lower-bound |
| method                 | .793                 | .333        |

Tests the null hypothesis that the error covariance matrix of the orthonormalized transformed dependent variables is proportional to an identity matrix.

a. Design: Intercept

Within Subjects Design: method

b. May be used to adjust the degrees of freedom for the averaged tests of significance. Corrected tests are displayed in the Tests of Within-Subjects Effects table.

### Tests of Within-Subjects Effects

Measure: score

| Source        |                    | Type III Sum of Squares | df     | Mean Square | F     |
|---------------|--------------------|-------------------------|--------|-------------|-------|
| method        | Sphericity Assumed | 114.157                 | 3      | 38.052      | 4.693 |
|               | Greenhouse-Geisser | 114.157                 | 1.891  | 60.354      | 4.693 |
|               | Huynh-Feldt        | 114.157                 | 2.379  | 47.976      | 4.693 |
|               | Lower-bound        | 114.157                 | 1.000  | 114.157     | 4.693 |
| Error(method) | Sphericity Assumed | 218.908                 | 27     | 8.108       |       |
|               | Greenhouse-Geisser | 218.908                 | 17.023 | 12.859      |       |
|               | Huynh-Feldt        | 218.908                 | 21.415 | 10.222      |       |
|               | Lower-bound        | 218.908                 | 9.000  | 24.323      |       |

### Tests of Within-Subjects Effects

Measure: score

| Source        |                    | Sig. |
|---------------|--------------------|------|
| method        | Sphericity Assumed | .009 |
|               | Greenhouse-Geisser | .025 |
|               | Huynh-Feldt        | .016 |
|               | Lower-bound        | .058 |
| Error(method) | Sphericity Assumed |      |
|               | Greenhouse-Geisser |      |
|               | Huynh-Feldt        |      |
|               | Lower-bound        |      |

### Tests of Within-Subjects Contrasts

Measure: score

| Source        | method    | Type III Sum of Squares | df | Mean Square | F      | Sig. |
|---------------|-----------|-------------------------|----|-------------|--------|------|
| method        | Linear    | 23.122                  | 1  | 23.122      | 1.587  | .239 |
|               | Quadratic | .249                    | 1  | .249        | .044   | .839 |
|               | Cubic     | 90.786                  | 1  | 90.786      | 22.468 | .001 |
| Error(method) | Linear    | 131.132                 | 9  | 14.570      |        |      |
|               | Quadratic | 51.410                  | 9  | 5.712       |        |      |
|               | Cubic     | 36.366                  | 9  | 4.041       |        |      |

### Tests of Between-Subjects Effects

Measure: score

Transformed Variable: Average

| Source    | Type III Sum of Squares | df | Mean Square | F        | Sig. |
|-----------|-------------------------|----|-------------|----------|------|
| Intercept | 18192.367               | 1  | 18192.367   | 1052.494 | .000 |
| Error     | 155.565                 | 9  | 17.285      |          |      |

### Estimated Marginal Means

method

## Estimates

Measure: score

| method | Mean   | Std. Error | 95% Confidence Interval |             |
|--------|--------|------------|-------------------------|-------------|
|        |        |            | Lower Bound             | Upper Bound |
| 1      | 19.554 | 1.133      | 16.991                  | 22.116      |
| 2      | 23.086 | .865       | 21.131                  | 25.042      |
| 3      | 19.724 | .903       | 17.682                  | 21.766      |
| 4      | 22.941 | 1.147      | 20.346                  | 25.536      |

## Pairwise Comparisons

Measure: score

| (I) method | (J) method | Mean Difference (I-J) | Std. Error | Sig. <sup>b</sup> | 95% Confidence Interval for Difference <sup>b</sup> |             |
|------------|------------|-----------------------|------------|-------------------|-----------------------------------------------------|-------------|
|            |            |                       |            |                   | Lower Bound                                         | Upper Bound |
| 1          | 2          | -3.533 <sup>*</sup>   | .823       | .002              | -5.395                                              | -1.671      |
|            | 3          | -.170                 | 1.523      | .913              | -3.615                                              | 3.274       |
|            | 4          | -3.388 <sup>*</sup>   | 1.449      | .044              | -6.666                                              | -.109       |
| 2          | 1          | 3.533 <sup>*</sup>    | .823       | .002              | 1.671                                               | 5.395       |
|            | 3          | 3.362 <sup>*</sup>    | 1.273      | .027              | .482                                                | 6.243       |
|            | 4          | .145                  | 1.456      | .923              | -3.149                                              | 3.439       |
| 3          | 1          | .170                  | 1.523      | .913              | -3.274                                              | 3.615       |
|            | 2          | -3.362 <sup>*</sup>   | 1.273      | .027              | -6.243                                              | -.482       |
|            | 4          | -3.217 <sup>*</sup>   | .944       | .008              | -5.352                                              | -1.082      |
| 4          | 1          | 3.388 <sup>*</sup>    | 1.449      | .044              | .109                                                | 6.666       |
|            | 2          | -.145                 | 1.456      | .923              | -3.439                                              | 3.149       |
|            | 3          | 3.217 <sup>*</sup>    | .944       | .008              | 1.082                                               | 5.352       |

Based on estimated marginal means

\*. The mean difference is significant at the .05 level.

b. Adjustment for multiple comparisons: Least Significant Difference (equivalent to no adjustments).

### Multivariate Tests

|                    | Value | F                   | Hypothesis df | Error df | Sig. |
|--------------------|-------|---------------------|---------------|----------|------|
| Pillai's trace     | .866  | 15.029 <sup>a</sup> | 3.000         | 7.000    | .002 |
| Wilks' lambda      | .134  | 15.029 <sup>a</sup> | 3.000         | 7.000    | .002 |
| Hotelling's trace  | 6.441 | 15.029 <sup>a</sup> | 3.000         | 7.000    | .002 |
| Roy's largest root | 6.441 | 15.029 <sup>a</sup> | 3.000         | 7.000    | .002 |

Each F tests the multivariate effect of method. These tests are based on the linearly independent pairwise comparisons among the estimated marginal means.

a. Exact statistic

### Profile Plots

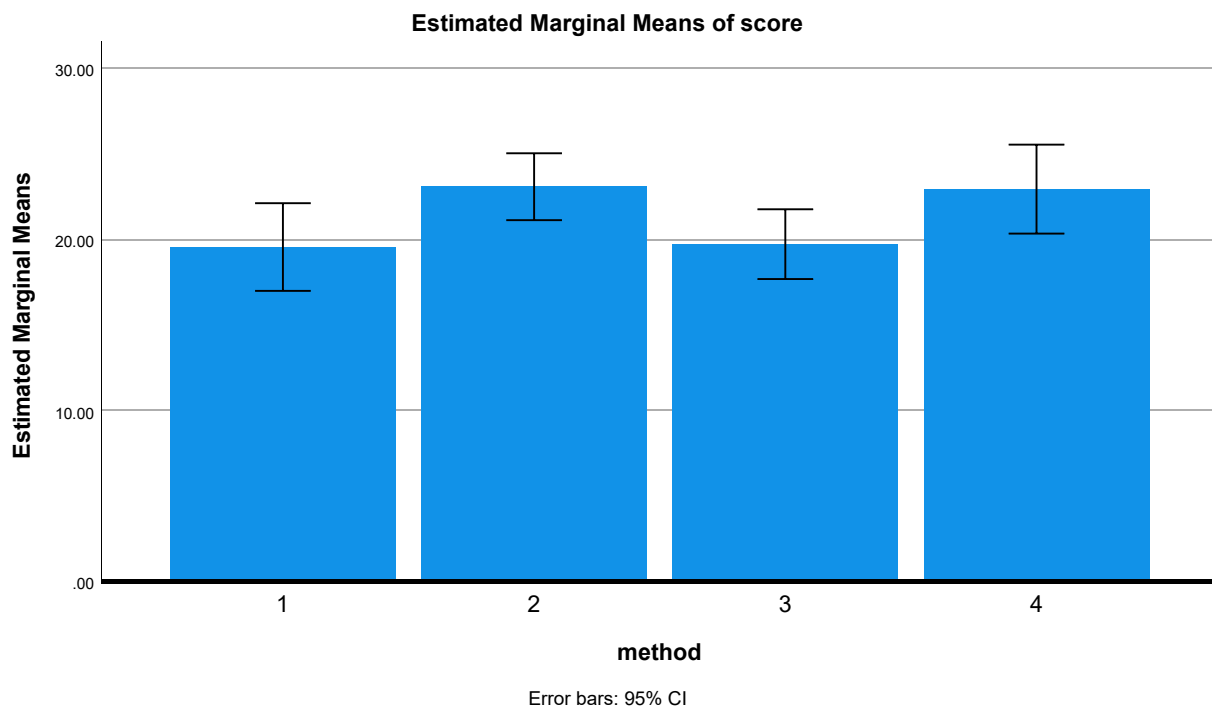

Supplement: Supplementary file 2 [file distractor_all.pdf]
