# Supplementary material for: Communicating Inferred Goals with Passive Augmented Reality and Active Haptic Feedback
Source: arXiv:2109.01747 source file (2021-09-03)

```

GLM A1 B1 C1 D1
  /WSFACTOR=method 4 Polynomial
  /MEASURE=distractor_score
  /METHOD=SSTYPE(3)
  /PLOT=PROFILE(method) TYPE=BAR ERRORBAR=CI MEANREFERENCE=NO
  /EMMEANS=TABLES(method) COMPARE ADJ(LSD)
  /PRINT=DESCRIPTIVE
  /CRITERIA=ALPHA(.05)
  /WSDSIGN=method.

```

## General Linear Model

### Within-Subjects Factors

Measure: distractor\_score

| method | Dependent<br>Variable |
|--------|-----------------------|
| 1      | A1                    |
| 2      | B1                    |
| 3      | C1                    |
| 4      | D1                    |

### Descriptive Statistics

|    | Mean    | Std. Deviation | N  |
|----|---------|----------------|----|
| A1 | 15.0357 | 7.07103        | 10 |
| B1 | 19.8924 | 3.81986        | 10 |
| C1 | 15.1201 | 2.55973        | 10 |
| D1 | 17.5404 | 5.70374        | 10 |

### Multivariate Tests<sup>a</sup>

| Effect |                    | Value | F                  | Hypothesis df | Error df | Sig. |
|--------|--------------------|-------|--------------------|---------------|----------|------|
| method | Pillai's Trace     | .659  | 4.509 <sup>b</sup> | 3.000         | 7.000    | .046 |
|        | Wilks' Lambda      | .341  | 4.509 <sup>b</sup> | 3.000         | 7.000    | .046 |
|        | Hotelling's Trace  | 1.932 | 4.509 <sup>b</sup> | 3.000         | 7.000    | .046 |
|        | Roy's Largest Root | 1.932 | 4.509 <sup>b</sup> | 3.000         | 7.000    | .046 |

a. Design: Intercept  
Within Subjects Design: method

b. Exact statistic

### Mauchly's Test of Sphericity<sup>a</sup>

Measure: distractor\_score

| Within Subjects Effect | Mauchly's W | Approx. Chi-Square | df | Sig. | Epsilon <sup>b</sup><br>Greenhouse-Geisser |
|------------------------|-------------|--------------------|----|------|--------------------------------------------|
| method                 | .589        | 4.094              | 5  | .539 | .808                                       |

### Mauchly's Test of Sphericity<sup>a</sup>

Measure: distractor\_score

| Within Subjects Effect | Epsilon <sup>b</sup> |             |
|------------------------|----------------------|-------------|
|                        | Huynh-Feldt          | Lower-bound |
| method                 | 1.000                | .333        |

Tests the null hypothesis that the error covariance matrix of the orthonormalized transformed dependent variables is proportional to an identity matrix.

a. Design: Intercept

Within Subjects Design: method

b. May be used to adjust the degrees of freedom for the averaged tests of significance. Corrected tests are displayed in the Tests of Within-Subjects Effects table.

### Tests of Within-Subjects Effects

Measure: distractor\_score

| Source        |                    | Type III Sum of Squares | df     | Mean Square | F     |
|---------------|--------------------|-------------------------|--------|-------------|-------|
| method        | Sphericity Assumed | 160.082                 | 3      | 53.361      | 2.039 |
|               | Greenhouse-Geisser | 160.082                 | 2.423  | 66.066      | 2.039 |
|               | Huynh-Feldt        | 160.082                 | 3.000  | 53.361      | 2.039 |
|               | Lower-bound        | 160.082                 | 1.000  | 160.082     | 2.039 |
| Error(method) | Sphericity Assumed | 706.673                 | 27     | 26.173      |       |
|               | Greenhouse-Geisser | 706.673                 | 21.807 | 32.405      |       |
|               | Huynh-Feldt        | 706.673                 | 27.000 | 26.173      |       |
|               | Lower-bound        | 706.673                 | 9.000  | 78.519      |       |

### Tests of Within-Subjects Effects

Measure: distractor\_score

| Source        |                    | Sig. |
|---------------|--------------------|------|
| method        | Sphericity Assumed | .132 |
|               | Greenhouse-Geisser | .147 |
|               | Huynh-Feldt        | .132 |
|               | Lower-bound        | .187 |
| Error(method) | Sphericity Assumed |      |
|               | Greenhouse-Geisser |      |
|               | Huynh-Feldt        |      |
|               | Lower-bound        |      |

### Tests of Within-Subjects Contrasts

Measure: distractor\_score

| Source        | method    | Type III Sum of Squares | df | Mean Square | F      | Sig. |
|---------------|-----------|-------------------------|----|-------------|--------|------|
| method        | Linear    | 3.759                   | 1  | 3.759       | .114   | .743 |
|               | Quadratic | 14.840                  | 1  | 14.840      | .421   | .533 |
|               | Cubic     | 141.483                 | 1  | 141.483     | 13.618 | .005 |
| Error(method) | Linear    | 295.814                 | 9  | 32.868      |        |      |
|               | Quadratic | 317.356                 | 9  | 35.262      |        |      |
|               | Cubic     | 93.502                  | 9  | 10.389      |        |      |

### Tests of Between-Subjects Effects

Measure: distractor\_score

Transformed Variable: Average

| Source    | Type III Sum of Squares | df | Mean Square | F       | Sig. |
|-----------|-------------------------|----|-------------|---------|------|
| Intercept | 11420.585               | 1  | 11420.585   | 453.984 | .000 |
| Error     | 226.407                 | 9  | 25.156      |         |      |

### Estimated Marginal Means

method

## Estimates

Measure: distractor\_score

| method | Mean   | Std. Error | 95% Confidence Interval |             |
|--------|--------|------------|-------------------------|-------------|
|        |        |            | Lower Bound             | Upper Bound |
| 1      | 15.036 | 2.236      | 9.977                   | 20.094      |
| 2      | 19.892 | 1.208      | 17.160                  | 22.625      |
| 3      | 15.120 | .809       | 13.289                  | 16.951      |
| 4      | 17.540 | 1.804      | 13.460                  | 21.621      |

## Pairwise Comparisons

Measure: distractor\_score

| (I) method | (J) method | Mean Difference (I-J) | Std. Error | Sig. <sup>b</sup> | 95% Confidence Interval for Difference <sup>b</sup> |             |
|------------|------------|-----------------------|------------|-------------------|-----------------------------------------------------|-------------|
|            |            |                       |            |                   | Lower Bound                                         | Upper Bound |
| 1          | 2          | -4.857 <sup>*</sup>   | 2.086      | .045              | -9.575                                              | -.138       |
|            | 3          | -.084                 | 2.786      | .976              | -6.387                                              | 6.218       |
|            | 4          | -2.505                | 2.330      | .310              | -7.776                                              | 2.767       |
| 2          | 1          | 4.857 <sup>*</sup>    | 2.086      | .045              | .138                                                | 9.575       |
|            | 3          | 4.772 <sup>*</sup>    | 1.795      | .026              | .712                                                | 8.832       |
|            | 4          | 2.352                 | 2.427      | .358              | -3.138                                              | 7.842       |
| 3          | 1          | .084                  | 2.786      | .976              | -6.218                                              | 6.387       |
|            | 2          | -4.772 <sup>*</sup>   | 1.795      | .026              | -8.832                                              | -.712       |
|            | 4          | -2.420                | 2.180      | .296              | -7.352                                              | 2.512       |
| 4          | 1          | 2.505                 | 2.330      | .310              | -2.767                                              | 7.776       |
|            | 2          | -2.352                | 2.427      | .358              | -7.842                                              | 3.138       |
|            | 3          | 2.420                 | 2.180      | .296              | -2.512                                              | 7.352       |

Based on estimated marginal means

\*. The mean difference is significant at the .05 level.

b. Adjustment for multiple comparisons: Least Significant Difference (equivalent to no adjustments).

### Multivariate Tests

|                    | Value | F                  | Hypothesis df | Error df | Sig. |
|--------------------|-------|--------------------|---------------|----------|------|
| Pillai's trace     | .659  | 4.509 <sup>a</sup> | 3.000         | 7.000    | .046 |
| Wilks' lambda      | .341  | 4.509 <sup>a</sup> | 3.000         | 7.000    | .046 |
| Hotelling's trace  | 1.932 | 4.509 <sup>a</sup> | 3.000         | 7.000    | .046 |
| Roy's largest root | 1.932 | 4.509 <sup>a</sup> | 3.000         | 7.000    | .046 |

Each F tests the multivariate effect of method. These tests are based on the linearly independent pairwise comparisons among the estimated marginal means.

a. Exact statistic

### Profile Plots

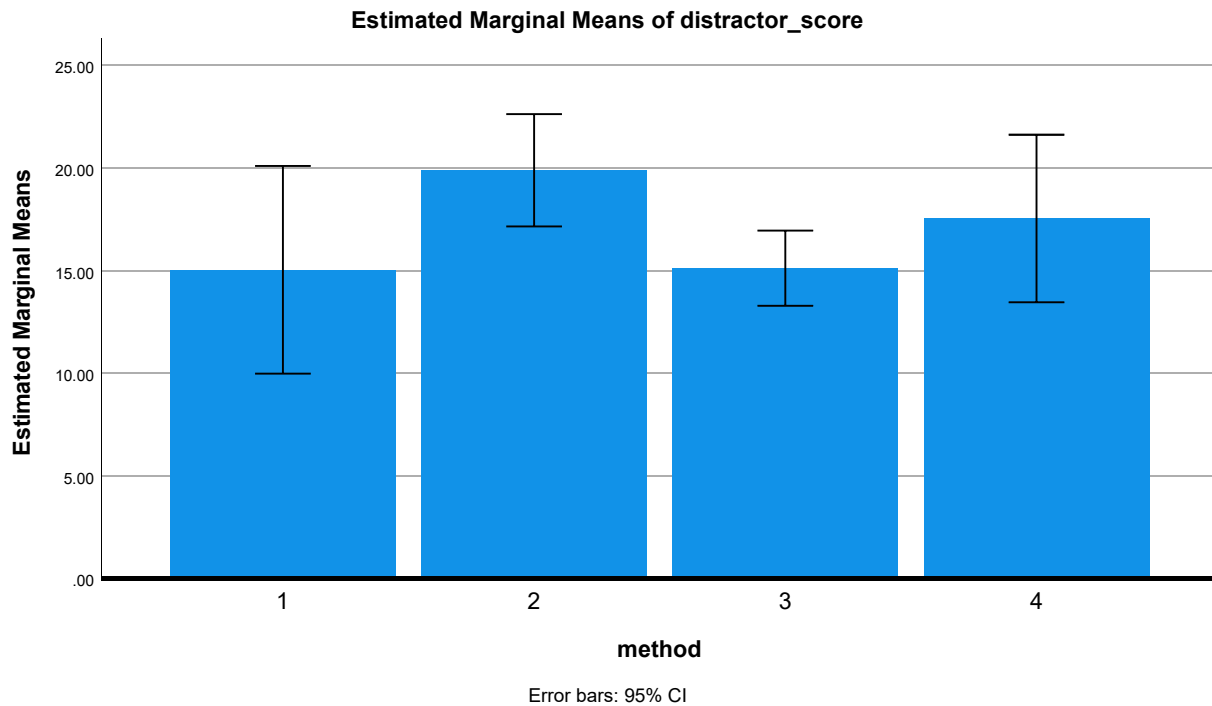

```
GLM A2 B2 C2 D2
  /WSFACTOR=method 4 Polynomial
  /MEASURE=distractor_score
  /METHOD=SSTYPE(3)
  /PLOT=PROFILE(method) TYPE=BAR ERRORBAR=CI MEANREFERENCE=NO
  /EMMEANS=TABLES(method) COMPARE ADJ(LSD)
  /PRINT=DESCRIPTIVE
  /CRITERIA=ALPHA(.05)
  /WSDESIGN=method.
```

### General Linear Model

## Within-Subjects Factors

Measure: distractor\_score

| method | Dependent<br>Variable |
|--------|-----------------------|
| 1      | A2                    |
| 2      | B2                    |
| 3      | C2                    |
| 4      | D2                    |

## Descriptive Statistics

|    | Mean    | Std. Deviation | N  |
|----|---------|----------------|----|
| A2 | 23.4658 | 5.02408        | 10 |
| B2 | 24.6478 | 4.81376        | 10 |
| C2 | 21.5003 | 6.92093        | 10 |
| D2 | 26.4732 | 5.51247        | 10 |

## Multivariate Tests<sup>a</sup>

| Effect |                    | Value | F                  | Hypothesis df | Error df | Sig. |
|--------|--------------------|-------|--------------------|---------------|----------|------|
| method | Pillai's Trace     | .705  | 5.583 <sup>b</sup> | 3.000         | 7.000    | .028 |
|        | Wilks' Lambda      | .295  | 5.583 <sup>b</sup> | 3.000         | 7.000    | .028 |
|        | Hotelling's Trace  | 2.393 | 5.583 <sup>b</sup> | 3.000         | 7.000    | .028 |
|        | Roy's Largest Root | 2.393 | 5.583 <sup>b</sup> | 3.000         | 7.000    | .028 |

a. Design: Intercept  
Within Subjects Design: method

b. Exact statistic

### Mauchly's Test of Sphericity<sup>a</sup>

Measure: distractor\_score

| Within Subjects Effect | Mauchly's W | Approx. Chi-Square | df | Sig. | Epsilon <sup>b</sup><br>Greenhouse-Geisser |
|------------------------|-------------|--------------------|----|------|--------------------------------------------|
| method                 | .297        | 9.386              | 5  | .097 | .563                                       |

### Mauchly's Test of Sphericity<sup>a</sup>

Measure: distractor\_score

| Within Subjects Effect | Epsilon <sup>b</sup> |             |
|------------------------|----------------------|-------------|
|                        | Huynh-Feldt          | Lower-bound |
| method                 | .679                 | .333        |

Tests the null hypothesis that the error covariance matrix of the orthonormalized transformed dependent variables is proportional to an identity matrix.

a. Design: Intercept

Within Subjects Design: method

b. May be used to adjust the degrees of freedom for the averaged tests of significance. Corrected tests are displayed in the Tests of Within-Subjects Effects table.

### Tests of Within-Subjects Effects

Measure: distractor\_score

| Source        |                    | Type III Sum of Squares | df     | Mean Square | F     |
|---------------|--------------------|-------------------------|--------|-------------|-------|
| method        | Sphericity Assumed | 130.681                 | 3      | 43.560      | 3.453 |
|               | Greenhouse-Geisser | 130.681                 | 1.689  | 77.365      | 3.453 |
|               | Huynh-Feldt        | 130.681                 | 2.037  | 64.156      | 3.453 |
|               | Lower-bound        | 130.681                 | 1.000  | 130.681     | 3.453 |
| Error(method) | Sphericity Assumed | 340.653                 | 27     | 12.617      |       |
|               | Greenhouse-Geisser | 340.653                 | 15.202 | 22.408      |       |
|               | Huynh-Feldt        | 340.653                 | 18.332 | 18.582      |       |
|               | Lower-bound        | 340.653                 | 9.000  | 37.850      |       |

### Tests of Within-Subjects Effects

Measure: distractor\_score

| Source        |                    | Sig. |
|---------------|--------------------|------|
| method        | Sphericity Assumed | .030 |
|               | Greenhouse-Geisser | .064 |
|               | Huynh-Feldt        | .053 |
|               | Lower-bound        | .096 |
| Error(method) | Sphericity Assumed |      |
|               | Greenhouse-Geisser |      |
|               | Huynh-Feldt        |      |
|               | Lower-bound        |      |

### Tests of Within-Subjects Contrasts

Measure: distractor\_score

| Source        | method    | Type III Sum of Squares | df | Mean Square | F      | Sig. |
|---------------|-----------|-------------------------|----|-------------|--------|------|
| method        | Linear    | 17.256                  | 1  | 17.256      | 1.469  | .256 |
|               | Quadratic | 35.927                  | 1  | 35.927      | 10.288 | .011 |
|               | Cubic     | 77.497                  | 1  | 77.497      | 3.428  | .097 |
| Error(method) | Linear    | 105.739                 | 9  | 11.749      |        |      |
|               | Quadratic | 31.429                  | 9  | 3.492       |        |      |
|               | Cubic     | 203.486                 | 9  | 22.610      |        |      |

### Tests of Between-Subjects Effects

Measure: distractor\_score

Transformed Variable: Average

| Source    | Type III Sum of Squares | df | Mean Square | F       | Sig. |
|-----------|-------------------------|----|-------------|---------|------|
| Intercept | 23081.790               | 1  | 23081.790   | 259.784 | .000 |
| Error     | 799.649                 | 9  | 88.850      |         |      |

### Estimated Marginal Means

method



## Estimates

Measure: distractor\_score

| method | Mean   | Std. Error | 95% Confidence Interval |             |
|--------|--------|------------|-------------------------|-------------|
|        |        |            | Lower Bound             | Upper Bound |
| 1      | 23.466 | 1.589      | 19.872                  | 27.060      |
| 2      | 24.648 | 1.522      | 21.204                  | 28.091      |
| 3      | 21.500 | 2.189      | 16.549                  | 26.451      |
| 4      | 26.473 | 1.743      | 22.530                  | 30.417      |

## Pairwise Comparisons

Measure: distractor\_score

| (I) method | (J) method | Mean Difference (I-J) | Std. Error | Sig. <sup>b</sup> | 95% Confidence Interval for Difference <sup>b</sup> |             |
|------------|------------|-----------------------|------------|-------------------|-----------------------------------------------------|-------------|
|            |            |                       |            |                   | Lower Bound                                         | Upper Bound |
| 1          | 2          | -1.182                | 1.308      | .390              | -4.142                                              | 1.778       |
|            | 3          | 1.965                 | 1.508      | .225              | -1.445                                              | 5.376       |
|            | 4          | -3.007 <sup>*</sup>   | 1.190      | .032              | -5.700                                              | -.314       |
| 2          | 1          | 1.182                 | 1.308      | .390              | -1.778                                              | 4.142       |
|            | 3          | 3.147                 | 2.335      | .211              | -2.136                                              | 8.431       |
|            | 4          | -1.825                | 1.656      | .299              | -5.572                                              | 1.921       |
| 3          | 1          | -1.965                | 1.508      | .225              | -5.376                                              | 1.445       |
|            | 2          | -3.147                | 2.335      | .211              | -8.431                                              | 2.136       |
|            | 4          | -4.973 <sup>*</sup>   | 1.241      | .003              | -7.781                                              | -2.165      |
| 4          | 1          | 3.007 <sup>*</sup>    | 1.190      | .032              | .314                                                | 5.700       |
|            | 2          | 1.825                 | 1.656      | .299              | -1.921                                              | 5.572       |
|            | 3          | 4.973 <sup>*</sup>    | 1.241      | .003              | 2.165                                               | 7.781       |

Based on estimated marginal means

\*. The mean difference is significant at the .05 level.

b. Adjustment for multiple comparisons: Least Significant Difference (equivalent to no adjustments).

### Multivariate Tests

|                    | Value | F                  | Hypothesis df | Error df | Sig. |
|--------------------|-------|--------------------|---------------|----------|------|
| Pillai's trace     | .705  | 5.583 <sup>a</sup> | 3.000         | 7.000    | .028 |
| Wilks' lambda      | .295  | 5.583 <sup>a</sup> | 3.000         | 7.000    | .028 |
| Hotelling's trace  | 2.393 | 5.583 <sup>a</sup> | 3.000         | 7.000    | .028 |
| Roy's largest root | 2.393 | 5.583 <sup>a</sup> | 3.000         | 7.000    | .028 |

Each F tests the multivariate effect of method. These tests are based on the linearly independent pairwise comparisons among the estimated marginal means.

a. Exact statistic

### Profile Plots

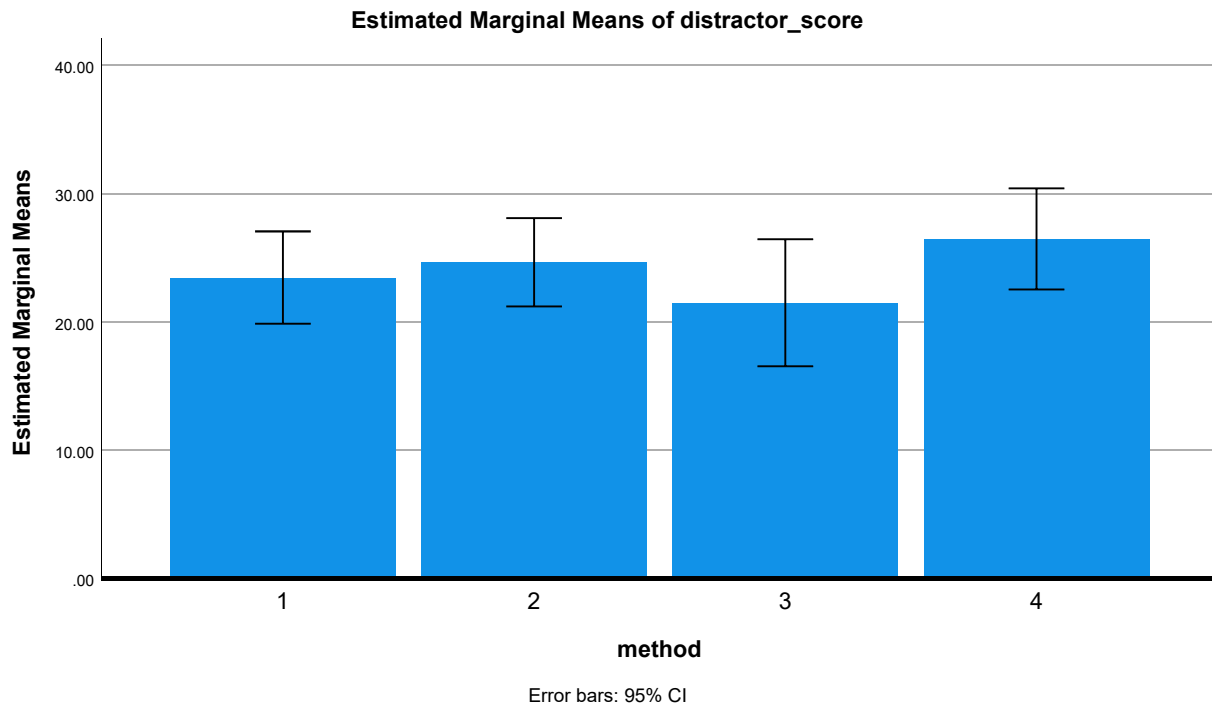

```
GLM A3 B3 C3 D3
  /WSFACTOR=method 4 Polynomial
  /MEASURE=distractor_score
  /METHOD=SSTYPE(3)
  /PLOT=PROFILE(method) TYPE=BAR ERRORBAR=CI MEANREFERENCE=NO
  /EMMEANS=TABLES(method) COMPARE ADJ(LSD)
  /PRINT=DESCRIPTIVE
  /CRITERIA=ALPHA(.05)
  /WSDESIGN=method.
```

### General Linear Model

## Within-Subjects Factors

Measure: distractor\_score

| method | Dependent<br>Variable |
|--------|-----------------------|
| 1      | A3                    |
| 2      | B3                    |
| 3      | C3                    |
| 4      | D3                    |

## Descriptive Statistics

|    | Mean    | Std. Deviation | N  |
|----|---------|----------------|----|
| A3 | 22.6360 | 5.15275        | 10 |
| B3 | 26.8980 | 4.80307        | 10 |
| C3 | 20.8349 | 4.36574        | 10 |
| D3 | 24.8463 | 3.43571        | 10 |

## Multivariate Tests<sup>a</sup>

| Effect |                    | Value | F                  | Hypothesis df | Error df | Sig. |
|--------|--------------------|-------|--------------------|---------------|----------|------|
| method | Pillai's Trace     | .705  | 5.567 <sup>b</sup> | 3.000         | 7.000    | .029 |
|        | Wilks' Lambda      | .295  | 5.567 <sup>b</sup> | 3.000         | 7.000    | .029 |
|        | Hotelling's Trace  | 2.386 | 5.567 <sup>b</sup> | 3.000         | 7.000    | .029 |
|        | Roy's Largest Root | 2.386 | 5.567 <sup>b</sup> | 3.000         | 7.000    | .029 |

a. Design: Intercept  
Within Subjects Design: method

b. Exact statistic

### Mauchly's Test of Sphericity<sup>a</sup>

Measure: distractor\_score

| Within Subjects Effect | Mauchly's W | Approx. Chi-Square | df | Sig. | Epsilon <sup>b</sup><br>Greenhouse-Geisser |
|------------------------|-------------|--------------------|----|------|--------------------------------------------|
| method                 | .769        | 2.025              | 5  | .847 | .851                                       |

### Mauchly's Test of Sphericity<sup>a</sup>

Measure: distractor\_score

| Within Subjects Effect | Huynh-Feldt | Epsilon <sup>b</sup><br>Lower-bound |
|------------------------|-------------|-------------------------------------|
| method                 | 1.000       | .333                                |

Tests the null hypothesis that the error covariance matrix of the orthonormalized transformed dependent variables is proportional to an identity matrix.

a. Design: Intercept

Within Subjects Design: method

b. May be used to adjust the degrees of freedom for the averaged tests of significance. Corrected tests are displayed in the Tests of Within-Subjects Effects table.

### Tests of Within-Subjects Effects

Measure: distractor\_score

| Source        |                    | Type III Sum of Squares | df     | Mean Square | F     |
|---------------|--------------------|-------------------------|--------|-------------|-------|
| method        | Sphericity Assumed | 208.387                 | 3      | 69.462      | 5.848 |
|               | Greenhouse-Geisser | 208.387                 | 2.553  | 81.626      | 5.848 |
|               | Huynh-Feldt        | 208.387                 | 3.000  | 69.462      | 5.848 |
|               | Lower-bound        | 208.387                 | 1.000  | 208.387     | 5.848 |
| Error(method) | Sphericity Assumed | 320.700                 | 27     | 11.878      |       |
|               | Greenhouse-Geisser | 320.700                 | 22.976 | 13.958      |       |
|               | Huynh-Feldt        | 320.700                 | 27.000 | 11.878      |       |
|               | Lower-bound        | 320.700                 | 9.000  | 35.633      |       |

### Tests of Within-Subjects Effects

Measure: distractor\_score

| Source        |                    | Sig. |
|---------------|--------------------|------|
| method        | Sphericity Assumed | .003 |
|               | Greenhouse-Geisser | .006 |
|               | Huynh-Feldt        | .003 |
|               | Lower-bound        | .039 |
| Error(method) | Sphericity Assumed |      |
|               | Greenhouse-Geisser |      |
|               | Huynh-Feldt        |      |
|               | Lower-bound        |      |

### Tests of Within-Subjects Contrasts

Measure: distractor\_score

| Source        | method    | Type III Sum of Squares | df | Mean Square | F      | Sig. |
|---------------|-----------|-------------------------|----|-------------|--------|------|
| method        | Linear    | .161                    | 1  | .161        | .009   | .926 |
|               | Quadratic | .157                    | 1  | .157        | .021   | .888 |
|               | Cubic     | 208.068                 | 1  | 208.068     | 20.293 | .001 |
| Error(method) | Linear    | 160.507                 | 9  | 17.834      |        |      |
|               | Quadratic | 67.916                  | 9  | 7.546       |        |      |
|               | Cubic     | 92.277                  | 9  | 10.253      |        |      |

### Tests of Between-Subjects Effects

Measure: distractor\_score

Transformed Variable: Average

| Source    | Type III Sum of Squares | df | Mean Square | F       | Sig. |
|-----------|-------------------------|----|-------------|---------|------|
| Intercept | 22664.829               | 1  | 22664.829   | 505.338 | .000 |
| Error     | 403.657                 | 9  | 44.851      |         |      |

### Estimated Marginal Means

method

## Estimates

Measure: distractor\_score

| method | Mean   | Std. Error | 95% Confidence Interval |             |
|--------|--------|------------|-------------------------|-------------|
|        |        |            | Lower Bound             | Upper Bound |
| 1      | 22.636 | 1.629      | 18.950                  | 26.322      |
| 2      | 26.898 | 1.519      | 23.462                  | 30.334      |
| 3      | 20.835 | 1.381      | 17.712                  | 23.958      |
| 4      | 24.846 | 1.086      | 22.389                  | 27.304      |

## Pairwise Comparisons

Measure: distractor\_score

| (I) method | (J) method | Mean Difference (I-J) | Std. Error | Sig. <sup>b</sup> | 95% Confidence Interval for Difference <sup>b</sup> |             |
|------------|------------|-----------------------|------------|-------------------|-----------------------------------------------------|-------------|
|            |            |                       |            |                   | Lower Bound                                         | Upper Bound |
| 1          | 2          | -4.262 <sup>*</sup>   | 1.436      | .016              | -7.510                                              | -1.014      |
|            | 3          | 1.801                 | 1.639      | .300              | -1.907                                              | 5.509       |
|            | 4          | -2.210                | 1.769      | .243              | -6.211                                              | 1.790       |
| 2          | 1          | 4.262 <sup>*</sup>    | 1.436      | .016              | 1.014                                               | 7.510       |
|            | 3          | 6.063 <sup>*</sup>    | 1.578      | .004              | 2.494                                               | 9.632       |
|            | 4          | 2.052                 | 1.571      | .224              | -1.503                                              | 5.606       |
| 3          | 1          | -1.801                | 1.639      | .300              | -5.509                                              | 1.907       |
|            | 2          | -6.063 <sup>*</sup>   | 1.578      | .004              | -9.632                                              | -2.494      |
|            | 4          | -4.011 <sup>*</sup>   | 1.191      | .008              | -6.705                                              | -1.317      |
| 4          | 1          | 2.210                 | 1.769      | .243              | -1.790                                              | 6.211       |
|            | 2          | -2.052                | 1.571      | .224              | -5.606                                              | 1.503       |
|            | 3          | 4.011 <sup>*</sup>    | 1.191      | .008              | 1.317                                               | 6.705       |

Based on estimated marginal means

\*. The mean difference is significant at the .05 level.

b. Adjustment for multiple comparisons: Least Significant Difference (equivalent to no adjustments).

### Multivariate Tests

|                    | Value | F                  | Hypothesis df | Error df | Sig. |
|--------------------|-------|--------------------|---------------|----------|------|
| Pillai's trace     | .705  | 5.567 <sup>a</sup> | 3.000         | 7.000    | .029 |
| Wilks' lambda      | .295  | 5.567 <sup>a</sup> | 3.000         | 7.000    | .029 |
| Hotelling's trace  | 2.386 | 5.567 <sup>a</sup> | 3.000         | 7.000    | .029 |
| Roy's largest root | 2.386 | 5.567 <sup>a</sup> | 3.000         | 7.000    | .029 |

Each F tests the multivariate effect of method. These tests are based on the linearly independent pairwise comparisons among the estimated marginal means.

a. Exact statistic

### Profile Plots

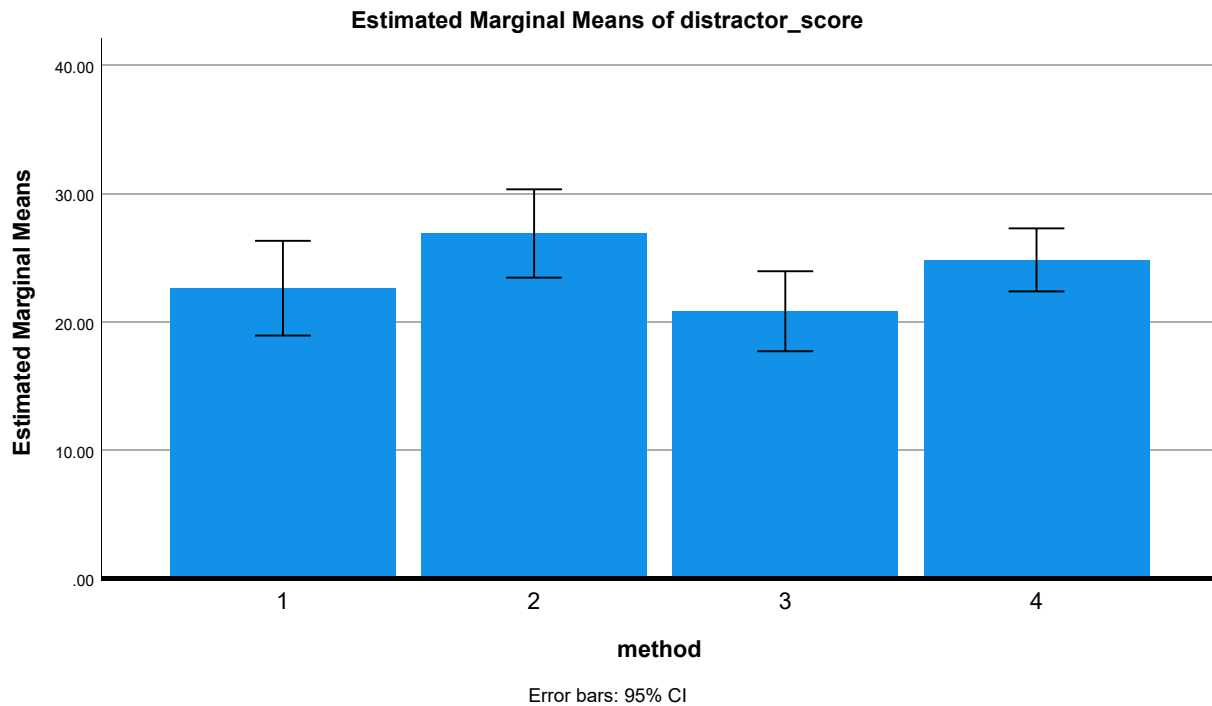

```
GLM A4 B4 C4 D4
  /WSFACTOR=method 4 Polynomial
  /MEASURE=distractor_score
  /METHOD=SSTYPE(3)
  /PLOT=PROFILE(method) TYPE=BAR ERRORBAR=CI MEANREFERENCE=NO
  /EMMEANS=TABLES(method) COMPARE ADJ(LSD)
  /PRINT=DESCRIPTIVE
  /CRITERIA=ALPHA(.05)
  /WSDESIGN=method.
```

### General Linear Model

## Within-Subjects Factors

Measure: distractor\_score

| method | Dependent<br>Variable |
|--------|-----------------------|
| 1      | A4                    |
| 2      | B4                    |
| 3      | C4                    |
| 4      | D4                    |

## Descriptive Statistics

|    | Mean    | Std. Deviation | N  |
|----|---------|----------------|----|
| A4 | 21.3553 | 1.97045        | 10 |
| B4 | 24.0310 | 4.22302        | 10 |
| C4 | 22.8986 | 6.55278        | 10 |
| D4 | 23.4426 | 4.18556        | 10 |

## Multivariate Tests<sup>a</sup>

| Effect |                    | Value | F                  | Hypothesis df | Error df | Sig. |
|--------|--------------------|-------|--------------------|---------------|----------|------|
| method | Pillai's Trace     | .380  | 1.428 <sup>b</sup> | 3.000         | 7.000    | .313 |
|        | Wilks' Lambda      | .620  | 1.428 <sup>b</sup> | 3.000         | 7.000    | .313 |
|        | Hotelling's Trace  | .612  | 1.428 <sup>b</sup> | 3.000         | 7.000    | .313 |
|        | Roy's Largest Root | .612  | 1.428 <sup>b</sup> | 3.000         | 7.000    | .313 |

a. Design: Intercept  
Within Subjects Design: method

b. Exact statistic



### Mauchly's Test of Sphericity<sup>a</sup>

Measure: distractor\_score

| Within Subjects Effect | Mauchly's W | Approx. Chi-Square | df | Sig. | Epsilon <sup>b</sup><br>Greenhouse-Geisser |
|------------------------|-------------|--------------------|----|------|--------------------------------------------|
| method                 | .321        | 8.764              | 5  | .121 | .572                                       |

### Mauchly's Test of Sphericity<sup>a</sup>

Measure: distractor\_score

| Within Subjects Effect | Epsilon <sup>b</sup> |             |
|------------------------|----------------------|-------------|
|                        | Huynh-Feldt          | Lower-bound |
| method                 | .693                 | .333        |

Tests the null hypothesis that the error covariance matrix of the orthonormalized transformed dependent variables is proportional to an identity matrix.

a. Design: Intercept

Within Subjects Design: method

b. May be used to adjust the degrees of freedom for the averaged tests of significance. Corrected tests are displayed in the Tests of Within-Subjects Effects table.

### Tests of Within-Subjects Effects

Measure: distractor\_score

| Source        |                    | Type III Sum of Squares | df     | Mean Square | F    |
|---------------|--------------------|-------------------------|--------|-------------|------|
| method        | Sphericity Assumed | 39.555                  | 3      | 13.185      | .588 |
|               | Greenhouse-Geisser | 39.555                  | 1.715  | 23.064      | .588 |
|               | Huynh-Feldt        | 39.555                  | 2.080  | 19.021      | .588 |
|               | Lower-bound        | 39.555                  | 1.000  | 39.555      | .588 |
| Error(method) | Sphericity Assumed | 605.746                 | 27     | 22.435      |      |
|               | Greenhouse-Geisser | 605.746                 | 15.435 | 39.245      |      |
|               | Huynh-Feldt        | 605.746                 | 18.716 | 32.364      |      |
|               | Lower-bound        | 605.746                 | 9.000  | 67.305      |      |

### Tests of Within-Subjects Effects

Measure: distractor\_score

| Source        |                    | Sig. |
|---------------|--------------------|------|
| method        | Sphericity Assumed | .628 |
|               | Greenhouse-Geisser | .543 |
|               | Huynh-Feldt        | .572 |
|               | Lower-bound        | .463 |
| Error(method) | Sphericity Assumed |      |
|               | Greenhouse-Geisser |      |
|               | Huynh-Feldt        |      |
|               | Lower-bound        |      |

### Tests of Within-Subjects Contrasts

Measure: distractor\_score

| Source        | method    | Type III Sum of Squares | df | Mean Square | F    | Sig. |
|---------------|-----------|-------------------------|----|-------------|------|------|
| method        | Linear    | 13.156                  | 1  | 13.156      | .719 | .418 |
|               | Quadratic | 11.360                  | 1  | 11.360      | .935 | .359 |
|               | Cubic     | 15.040                  | 1  | 15.040      | .408 | .539 |
| Error(method) | Linear    | 164.626                 | 9  | 18.292      |      |      |
|               | Quadratic | 109.317                 | 9  | 12.146      |      |      |
|               | Cubic     | 331.803                 | 9  | 36.867      |      |      |

### Tests of Between-Subjects Effects

Measure: distractor\_score

Transformed Variable: Average

| Source    | Type III Sum of Squares | df | Mean Square | F        | Sig. |
|-----------|-------------------------|----|-------------|----------|------|
| Intercept | 21034.884               | 1  | 21034.884   | 1414.649 | .000 |
| Error     | 133.824                 | 9  | 14.869      |          |      |

### Estimated Marginal Means

method

## Estimates

Measure: distractor\_score

| method | Mean   | Std. Error | 95% Confidence Interval |             |
|--------|--------|------------|-------------------------|-------------|
|        |        |            | Lower Bound             | Upper Bound |
| 1      | 21.355 | .623       | 19.946                  | 22.765      |
| 2      | 24.031 | 1.335      | 21.010                  | 27.052      |
| 3      | 22.899 | 2.072      | 18.211                  | 27.586      |
| 4      | 23.443 | 1.324      | 20.448                  | 26.437      |

## Pairwise Comparisons

Measure: distractor\_score

| (I) method | (J) method | Mean Difference (I-J) | Std. Error | Sig. <sup>a</sup> | 95% Confidence Interval for Difference <sup>a</sup> |             |
|------------|------------|-----------------------|------------|-------------------|-----------------------------------------------------|-------------|
|            |            |                       |            |                   | Lower Bound                                         | Upper Bound |
| 1          | 2          | -2.676                | 1.424      | .093              | -5.896                                              | .545        |
|            | 3          | -1.543                | 2.481      | .549              | -7.155                                              | 4.069       |
|            | 4          | -2.087                | 1.358      | .159              | -5.160                                              | .985        |
| 2          | 1          | 2.676                 | 1.424      | .093              | -.545                                               | 5.896       |
|            | 3          | 1.132                 | 3.031      | .717              | -5.724                                              | 7.989       |
|            | 4          | .588                  | 1.895      | .763              | -3.698                                              | 4.874       |
| 3          | 1          | 1.543                 | 2.481      | .549              | -4.069                                              | 7.155       |
|            | 2          | -1.132                | 3.031      | .717              | -7.989                                              | 5.724       |
|            | 4          | -.544                 | 2.030      | .795              | -5.135                                              | 4.047       |
| 4          | 1          | 2.087                 | 1.358      | .159              | -.985                                               | 5.160       |
|            | 2          | -.588                 | 1.895      | .763              | -4.874                                              | 3.698       |
|            | 3          | .544                  | 2.030      | .795              | -4.047                                              | 5.135       |

Based on estimated marginal means

a. Adjustment for multiple comparisons: Least Significant Difference (equivalent to no adjustments).

### Multivariate Tests

|                    | Value | F                  | Hypothesis df | Error df | Sig. |
|--------------------|-------|--------------------|---------------|----------|------|
| Pillai's trace     | .380  | 1.428 <sup>a</sup> | 3.000         | 7.000    | .313 |
| Wilks' lambda      | .620  | 1.428 <sup>a</sup> | 3.000         | 7.000    | .313 |
| Hotelling's trace  | .612  | 1.428 <sup>a</sup> | 3.000         | 7.000    | .313 |
| Roy's largest root | .612  | 1.428 <sup>a</sup> | 3.000         | 7.000    | .313 |

Each F tests the multivariate effect of method. These tests are based on the linearly independent pairwise comparisons among the estimated marginal means.

a. Exact statistic

### Profile Plots

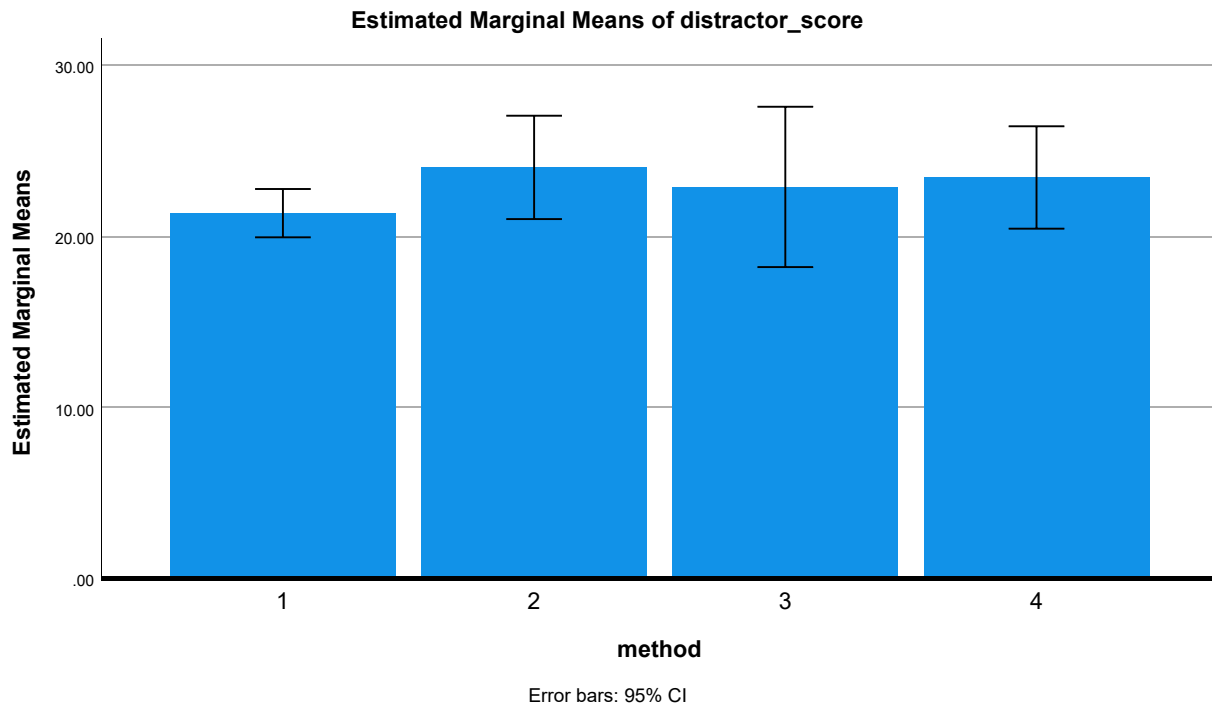

```
GLM A5 B5 C5 D5
  /WSFACTOR=method 4 Polynomial
  /MEASURE=distractor_score
  /METHOD=SSTYPE(3)
  /PLOT=PROFILE(method) TYPE=BAR ERRORBAR=CI MEANREFERENCE=NO
  /EMMEANS=TABLES(method) COMPARE ADJ(LSD)
  /PRINT=DESCRIPTIVE
  /CRITERIA=ALPHA(.05)
  /WSDESIGN=method.
```

### General Linear Model

## Within-Subjects Factors

Measure: distractor\_score

| method | Dependent<br>Variable |
|--------|-----------------------|
| 1      | A5                    |
| 2      | B5                    |
| 3      | C5                    |
| 4      | D5                    |

## Descriptive Statistics

|    | Mean    | Std. Deviation | N  |
|----|---------|----------------|----|
| A5 | 19.1492 | 5.04016        | 10 |
| B5 | 20.9072 | 3.41930        | 10 |
| C5 | 21.4403 | 4.88888        | 10 |
| D5 | 22.9048 | 4.47075        | 10 |

## Multivariate Tests<sup>a</sup>

| Effect |                    | Value | F                  | Hypothesis df | Error df | Sig. |
|--------|--------------------|-------|--------------------|---------------|----------|------|
| method | Pillai's Trace     | .347  | 1.240 <sup>b</sup> | 3.000         | 7.000    | .365 |
|        | Wilks' Lambda      | .653  | 1.240 <sup>b</sup> | 3.000         | 7.000    | .365 |
|        | Hotelling's Trace  | .532  | 1.240 <sup>b</sup> | 3.000         | 7.000    | .365 |
|        | Roy's Largest Root | .532  | 1.240 <sup>b</sup> | 3.000         | 7.000    | .365 |

a. Design: Intercept  
Within Subjects Design: method

b. Exact statistic

### Mauchly's Test of Sphericity<sup>a</sup>

Measure: distractor\_score

| Within Subjects Effect | Mauchly's W | Approx. Chi-Square | df | Sig. | Epsilon <sup>b</sup><br>Greenhouse-Geisser |
|------------------------|-------------|--------------------|----|------|--------------------------------------------|
| method                 | .524        | 4.998              | 5  | .419 | .684                                       |

### Mauchly's Test of Sphericity<sup>a</sup>

Measure: distractor\_score

| Within Subjects Effect | Epsilon <sup>b</sup> |             |
|------------------------|----------------------|-------------|
|                        | Huynh-Feldt          | Lower-bound |
| method                 | .889                 | .333        |

Tests the null hypothesis that the error covariance matrix of the orthonormalized transformed dependent variables is proportional to an identity matrix.

a. Design: Intercept

Within Subjects Design: method

b. May be used to adjust the degrees of freedom for the averaged tests of significance. Corrected tests are displayed in the Tests of Within-Subjects Effects table.

### Tests of Within-Subjects Effects

Measure: distractor\_score

| Source        |                    | Type III Sum of Squares | df     | Mean Square | F     |
|---------------|--------------------|-------------------------|--------|-------------|-------|
| method        | Sphericity Assumed | 72.158                  | 3      | 24.053      | 1.287 |
|               | Greenhouse-Geisser | 72.158                  | 2.053  | 35.143      | 1.287 |
|               | Huynh-Feldt        | 72.158                  | 2.668  | 27.048      | 1.287 |
|               | Lower-bound        | 72.158                  | 1.000  | 72.158      | 1.287 |
| Error(method) | Sphericity Assumed | 504.720                 | 27     | 18.693      |       |
|               | Greenhouse-Geisser | 504.720                 | 18.479 | 27.313      |       |
|               | Huynh-Feldt        | 504.720                 | 24.010 | 21.021      |       |
|               | Lower-bound        | 504.720                 | 9.000  | 56.080      |       |

### Tests of Within-Subjects Effects

Measure: distractor\_score

| Source        |                    | Sig. |
|---------------|--------------------|------|
| method        | Sphericity Assumed | .299 |
|               | Greenhouse-Geisser | .301 |
|               | Huynh-Feldt        | .300 |
|               | Lower-bound        | .286 |
| Error(method) | Sphericity Assumed |      |
|               | Greenhouse-Geisser |      |
|               | Huynh-Feldt        |      |
|               | Lower-bound        |      |

### Tests of Within-Subjects Contrasts

Measure: distractor\_score

| Source        | method    | Type III Sum of Squares | df | Mean Square | F     | Sig. |
|---------------|-----------|-------------------------|----|-------------|-------|------|
| method        | Linear    | 69.617                  | 1  | 69.617      | 3.362 | .100 |
|               | Quadratic | .215                    | 1  | .215        | .008  | .930 |
|               | Cubic     | 2.325                   | 1  | 2.325       | .251  | .628 |
| Error(method) | Linear    | 186.383                 | 9  | 20.709      |       |      |
|               | Quadratic | 234.997                 | 9  | 26.111      |       |      |
|               | Cubic     | 83.340                  | 9  | 9.260       |       |      |

### Tests of Between-Subjects Effects

Measure: distractor\_score

Transformed Variable: Average

| Source    | Type III Sum of Squares | df | Mean Square | F       | Sig. |
|-----------|-------------------------|----|-------------|---------|------|
| Intercept | 17809.032               | 1  | 17809.032   | 715.121 | .000 |
| Error     | 224.132                 | 9  | 24.904      |         |      |

### Estimated Marginal Means

method

## Estimates

Measure: distractor\_score

| method | Mean   | Std. Error | 95% Confidence Interval |             |
|--------|--------|------------|-------------------------|-------------|
|        |        |            | Lower Bound             | Upper Bound |
| 1      | 19.149 | 1.594      | 15.544                  | 22.755      |
| 2      | 20.907 | 1.081      | 18.461                  | 23.353      |
| 3      | 21.440 | 1.546      | 17.943                  | 24.938      |
| 4      | 22.905 | 1.414      | 19.707                  | 26.103      |

## Pairwise Comparisons

Measure: distractor\_score

| (I) method | (J) method | Mean Difference (I-J) | Std. Error | Sig. <sup>a</sup> | 95% Confidence Interval for Difference <sup>a</sup> |             |
|------------|------------|-----------------------|------------|-------------------|-----------------------------------------------------|-------------|
|            |            |                       |            |                   | Lower Bound                                         | Upper Bound |
| 1          | 2          | -1.758                | 2.027      | .408              | -6.343                                              | 2.827       |
|            | 3          | -2.291                | 2.668      | .413              | -8.326                                              | 3.744       |
|            | 4          | -3.756                | 1.920      | .082              | -8.100                                              | .589        |
| 2          | 1          | 1.758                 | 2.027      | .408              | -2.827                                              | 6.343       |
|            | 3          | -.533                 | 1.518      | .734              | -3.968                                              | 2.902       |
|            | 4          | -1.998                | 1.445      | .200              | -5.266                                              | 1.271       |
| 3          | 1          | 2.291                 | 2.668      | .413              | -3.744                                              | 8.326       |
|            | 2          | .533                  | 1.518      | .734              | -2.902                                              | 3.968       |
|            | 4          | -1.465                | 1.768      | .429              | -5.463                                              | 2.534       |
| 4          | 1          | 3.756                 | 1.920      | .082              | -.589                                               | 8.100       |
|            | 2          | 1.998                 | 1.445      | .200              | -1.271                                              | 5.266       |
|            | 3          | 1.465                 | 1.768      | .429              | -2.534                                              | 5.463       |

Based on estimated marginal means

a. Adjustment for multiple comparisons: Least Significant Difference (equivalent to no adjustments).



### Multivariate Tests

|                    | Value | F                  | Hypothesis df | Error df | Sig. |
|--------------------|-------|--------------------|---------------|----------|------|
| Pillai's trace     | .347  | 1.240 <sup>a</sup> | 3.000         | 7.000    | .365 |
| Wilks' lambda      | .653  | 1.240 <sup>a</sup> | 3.000         | 7.000    | .365 |
| Hotelling's trace  | .532  | 1.240 <sup>a</sup> | 3.000         | 7.000    | .365 |
| Roy's largest root | .532  | 1.240 <sup>a</sup> | 3.000         | 7.000    | .365 |

Each F tests the multivariate effect of method. These tests are based on the linearly independent pairwise comparisons among the estimated marginal means.

a. Exact statistic

### Profile Plots

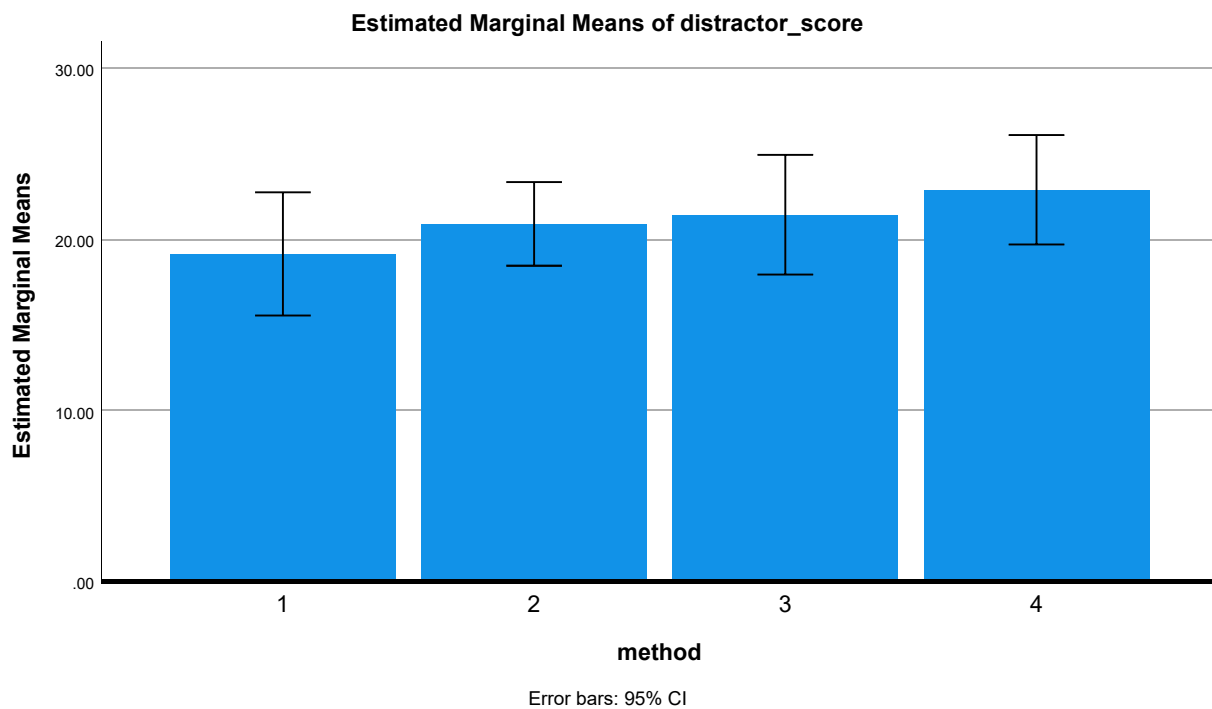

Supplement: Supplementary file 3 [file distractor_task.pdf]
