# Supplementary material for: Communicating Inferred Goals with Passive Augmented Reality and Active Haptic Feedback
Source: arXiv:2109.01747 source file (2021-09-03)

```

GLM A1 B1 C1 D1
  /WSFACTOR=method 4 Polynomial
  /MEASURE=rating
  /METHOD=SSTYPE(3)
  /PLOT=PROFILE(method) TYPE=BAR ERRORBAR=CI MEANREFERENCE=NO
  /EMMEANS=TABLES(method) COMPARE ADJ(LSD)
  /PRINT=DESCRIPTIVE
  /CRITERIA=ALPHA(.05)
  /WSDESIGN=method.

```

## General Linear Model

### Within-Subjects Factors

Measure: rating

| method | Dependent<br>Variable |
|--------|-----------------------|
| 1      | A1                    |
| 2      | B1                    |
| 3      | C1                    |
| 4      | D1                    |

### Descriptive Statistics

|    | Mean   | Std. Deviation | N  |
|----|--------|----------------|----|
| A1 | 5.9500 | .98460         | 10 |
| B1 | 4.2000 | 2.11082        | 10 |
| C1 | 6.4000 | .69921         | 10 |
| D1 | 6.7000 | .42164         | 10 |

### Multivariate Tests<sup>a</sup>

| Effect |                    | Value | F                  | Hypothesis df | Error df | Sig. |
|--------|--------------------|-------|--------------------|---------------|----------|------|
| method | Pillai's Trace     | .655  | 4.433 <sup>b</sup> | 3.000         | 7.000    | .048 |
|        | Wilks' Lambda      | .345  | 4.433 <sup>b</sup> | 3.000         | 7.000    | .048 |
|        | Hotelling's Trace  | 1.900 | 4.433 <sup>b</sup> | 3.000         | 7.000    | .048 |
|        | Roy's Largest Root | 1.900 | 4.433 <sup>b</sup> | 3.000         | 7.000    | .048 |

a. Design: Intercept  
Within Subjects Design: method

b. Exact statistic

### Mauchly's Test of Sphericity<sup>a</sup>

Measure: rating

| Within Subjects Effect | Mauchly's W | Approx. Chi-Square | df | Sig. | Epsilon <sup>b</sup><br>Greenhouse-Geisser |
|------------------------|-------------|--------------------|----|------|--------------------------------------------|
| method                 | .137        | 15.372             | 5  | .009 | .511                                       |

### Mauchly's Test of Sphericity<sup>a</sup>

Measure: rating

| Within Subjects Effect | Epsilon <sup>b</sup> |             |
|------------------------|----------------------|-------------|
|                        | Huynh-Feldt          | Lower-bound |
| method                 | .596                 | .333        |

Tests the null hypothesis that the error covariance matrix of the orthonormalized transformed dependent variables is proportional to an identity matrix.

a. Design: Intercept

Within Subjects Design: method

b. May be used to adjust the degrees of freedom for the averaged tests of significance. Corrected tests are displayed in the Tests of Within-Subjects Effects table.

### Tests of Within-Subjects Effects

Measure: rating

| Source        |                    | Type III Sum of Squares | df     | Mean Square | F     |
|---------------|--------------------|-------------------------|--------|-------------|-------|
| method        | Sphericity Assumed | 37.519                  | 3      | 12.506      | 8.539 |
|               | Greenhouse-Geisser | 37.519                  | 1.534  | 24.454      | 8.539 |
|               | Huynh-Feldt        | 37.519                  | 1.787  | 20.993      | 8.539 |
|               | Lower-bound        | 37.519                  | 1.000  | 37.519      | 8.539 |
| Error(method) | Sphericity Assumed | 39.544                  | 27     | 1.465       |       |
|               | Greenhouse-Geisser | 39.544                  | 13.808 | 2.864       |       |
|               | Huynh-Feldt        | 39.544                  | 16.085 | 2.458       |       |
|               | Lower-bound        | 39.544                  | 9.000  | 4.394       |       |

### Tests of Within-Subjects Effects

Measure: rating

| Source        |                    | Sig. |
|---------------|--------------------|------|
| method        | Sphericity Assumed | .000 |
|               | Greenhouse-Geisser | .006 |
|               | Huynh-Feldt        | .004 |
|               | Lower-bound        | .017 |
| Error(method) | Sphericity Assumed |      |
|               | Greenhouse-Geisser |      |
|               | Huynh-Feldt        |      |
|               | Lower-bound        |      |

### Tests of Within-Subjects Contrasts

Measure: rating

| Source        | method    | Type III Sum of Squares | df | Mean Square | F      | Sig. |
|---------------|-----------|-------------------------|----|-------------|--------|------|
| method        | Linear    | 9.901                   | 1  | 9.901       | 11.020 | .009 |
|               | Quadratic | 10.506                  | 1  | 10.506      | 8.650  | .016 |
|               | Cubic     | 17.111                  | 1  | 17.111      | 7.503  | .023 |
| Error(method) | Linear    | 8.086                   | 9  | .898        |        |      |
|               | Quadratic | 10.931                  | 9  | 1.215       |        |      |
|               | Cubic     | 20.526                  | 9  | 2.281       |        |      |

### Tests of Between-Subjects Effects

Measure: rating

Transformed Variable: Average

| Source    | Type III Sum of Squares | df | Mean Square | F       | Sig. |
|-----------|-------------------------|----|-------------|---------|------|
| Intercept | 1351.406                | 1  | 1351.406    | 795.920 | .000 |
| Error     | 15.281                  | 9  | 1.698       |         |      |

### Estimated Marginal Means

method

## Estimates

Measure: rating

| method | Mean  | Std. Error | 95% Confidence Interval |             |
|--------|-------|------------|-------------------------|-------------|
|        |       |            | Lower Bound             | Upper Bound |
| 1      | 5.950 | .311       | 5.246                   | 6.654       |
| 2      | 4.200 | .667       | 2.690                   | 5.710       |
| 3      | 6.400 | .221       | 5.900                   | 6.900       |
| 4      | 6.700 | .133       | 6.398                   | 7.002       |

## Pairwise Comparisons

Measure: rating

| (I) method | (J) method | Mean Difference (I-J) | Std. Error | Sig. <sup>b</sup> | 95% Confidence Interval for Difference <sup>b</sup> |             |
|------------|------------|-----------------------|------------|-------------------|-----------------------------------------------------|-------------|
|            |            |                       |            |                   | Lower Bound                                         | Upper Bound |
| 1          | 2          | 1.750 <sup>*</sup>    | .716       | .037              | .131                                                | 3.369       |
|            | 3          | -.450                 | .337       | .215              | -1.212                                              | .312        |
|            | 4          | -.750                 | .367       | .071              | -1.580                                              | .080        |
| 2          | 1          | -1.750 <sup>*</sup>   | .716       | .037              | -3.369                                              | -.131       |
|            | 3          | -2.200 <sup>*</sup>   | .708       | .013              | -3.801                                              | -.599       |
|            | 4          | -2.500 <sup>*</sup>   | .679       | .005              | -4.036                                              | -.964       |
| 3          | 1          | .450                  | .337       | .215              | -.312                                               | 1.212       |
|            | 2          | 2.200 <sup>*</sup>    | .708       | .013              | .599                                                | 3.801       |
|            | 4          | -.300                 | .186       | .140              | -.720                                               | .120        |
| 4          | 1          | .750                  | .367       | .071              | -.080                                               | 1.580       |
|            | 2          | 2.500 <sup>*</sup>    | .679       | .005              | .964                                                | 4.036       |
|            | 3          | .300                  | .186       | .140              | -.120                                               | .720        |

Based on estimated marginal means

\*. The mean difference is significant at the .05 level.

b. Adjustment for multiple comparisons: Least Significant Difference (equivalent to no adjustments).

### Multivariate Tests

|                    | Value | F                  | Hypothesis df | Error df | Sig. |
|--------------------|-------|--------------------|---------------|----------|------|
| Pillai's trace     | .655  | 4.433 <sup>a</sup> | 3.000         | 7.000    | .048 |
| Wilks' lambda      | .345  | 4.433 <sup>a</sup> | 3.000         | 7.000    | .048 |
| Hotelling's trace  | 1.900 | 4.433 <sup>a</sup> | 3.000         | 7.000    | .048 |
| Roy's largest root | 1.900 | 4.433 <sup>a</sup> | 3.000         | 7.000    | .048 |

Each F tests the multivariate effect of method. These tests are based on the linearly independent pairwise comparisons among the estimated marginal means.

a. Exact statistic

### Profile Plots

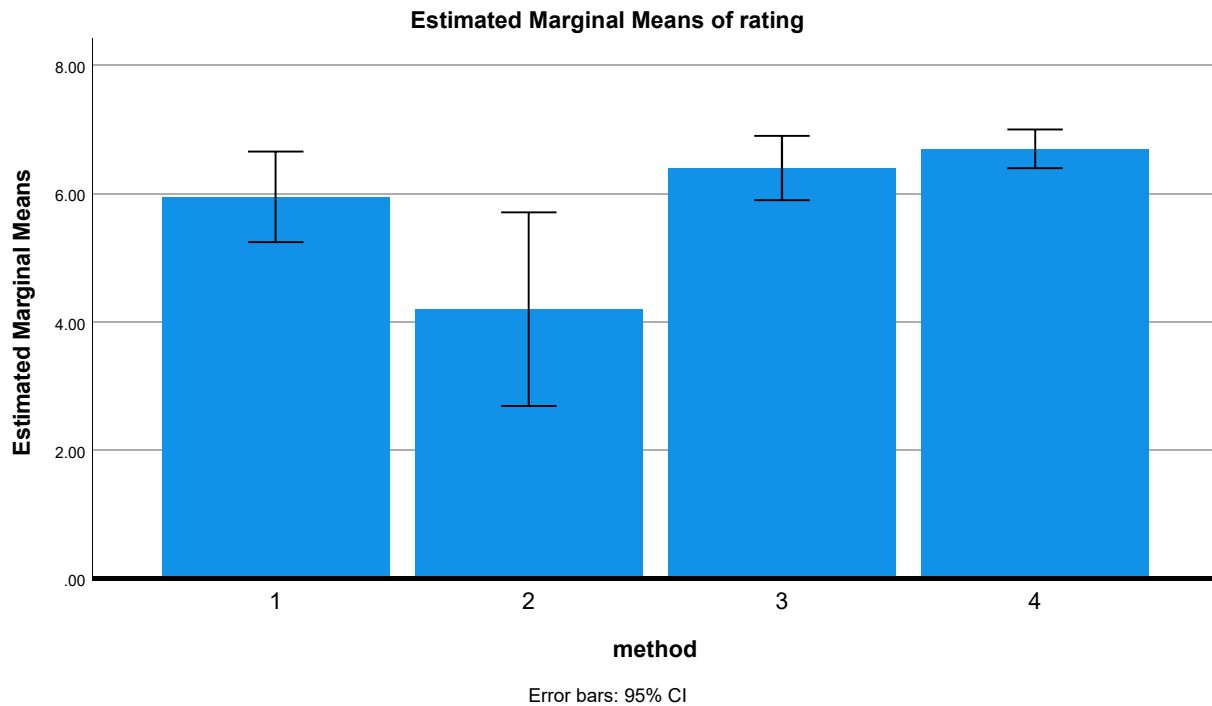

```
GLM A2 B2 C2 D2
  /WSFACTOR=method 4 Polynomial
  /MEASURE=rating
  /METHOD=SSTYPE(3)
  /PLOT=PROFILE(method) TYPE=BAR ERRORBAR=CI MEANREFERENCE=NO
  /EMMEANS=TABLES(method) COMPARE ADJ(LSD)
  /PRINT=DESCRIPTIVE
  /CRITERIA=ALPHA(.05)
  /WSDESIGN=method.
```

### General Linear Model

## Within-Subjects Factors

Measure: rating

| method | Dependent<br>Variable |
|--------|-----------------------|
| 1      | A2                    |
| 2      | B2                    |
| 3      | C2                    |
| 4      | D2                    |

## Descriptive Statistics

|    | Mean   | Std. Deviation | N  |
|----|--------|----------------|----|
| A2 | 4.2500 | 1.82954        | 10 |
| B2 | 6.5500 | .59861         | 10 |
| C2 | 2.3500 | 1.17969        | 10 |
| D2 | 6.9000 | .21082         | 10 |

## Multivariate Tests<sup>a</sup>

| Effect |                    | Value  | F                   | Hypothesis df | Error df | Sig. |
|--------|--------------------|--------|---------------------|---------------|----------|------|
| method | Pillai's Trace     | .957   | 52.093 <sup>b</sup> | 3.000         | 7.000    | .000 |
|        | Wilks' Lambda      | .043   | 52.093 <sup>b</sup> | 3.000         | 7.000    | .000 |
|        | Hotelling's Trace  | 22.325 | 52.093 <sup>b</sup> | 3.000         | 7.000    | .000 |
|        | Roy's Largest Root | 22.325 | 52.093 <sup>b</sup> | 3.000         | 7.000    | .000 |

a. Design: Intercept  
Within Subjects Design: method

b. Exact statistic

### Mauchly's Test of Sphericity<sup>a</sup>

Measure: rating

| Within Subjects Effect | Mauchly's W | Approx. Chi-Square | df | Sig. | Epsilon <sup>b</sup><br>Greenhouse-Geisser |
|------------------------|-------------|--------------------|----|------|--------------------------------------------|
| method                 | .192        | 12.751             | 5  | .027 | .630                                       |

### Mauchly's Test of Sphericity<sup>a</sup>

Measure: rating

| Within Subjects Effect | Epsilon <sup>b</sup> |             |
|------------------------|----------------------|-------------|
|                        | Huynh-Feldt          | Lower-bound |
| method                 | .791                 | .333        |

Tests the null hypothesis that the error covariance matrix of the orthonormalized transformed dependent variables is proportional to an identity matrix.

a. Design: Intercept

Within Subjects Design: method

b. May be used to adjust the degrees of freedom for the averaged tests of significance. Corrected tests are displayed in the Tests of Within-Subjects Effects table.

### Tests of Within-Subjects Effects

Measure: rating

| Source        |                    | Type III Sum of Squares | df     | Mean Square | F      |
|---------------|--------------------|-------------------------|--------|-------------|--------|
| method        | Sphericity Assumed | 135.969                 | 3      | 45.323      | 32.769 |
|               | Greenhouse-Geisser | 135.969                 | 1.889  | 71.997      | 32.769 |
|               | Huynh-Feldt        | 135.969                 | 2.374  | 57.265      | 32.769 |
|               | Lower-bound        | 135.969                 | 1.000  | 135.969     | 32.769 |
| Error(method) | Sphericity Assumed | 37.344                  | 27     | 1.383       |        |
|               | Greenhouse-Geisser | 37.344                  | 16.997 | 2.197       |        |
|               | Huynh-Feldt        | 37.344                  | 21.369 | 1.748       |        |
|               | Lower-bound        | 37.344                  | 9.000  | 4.149       |        |

### Tests of Within-Subjects Effects

Measure: rating

| Source        |                    | Sig. |
|---------------|--------------------|------|
| method        | Sphericity Assumed | .000 |
|               | Greenhouse-Geisser | .000 |
|               | Huynh-Feldt        | .000 |
|               | Lower-bound        | .000 |
| Error(method) | Sphericity Assumed |      |
|               | Greenhouse-Geisser |      |
|               | Huynh-Feldt        |      |
|               | Lower-bound        |      |

### Tests of Within-Subjects Contrasts

Measure: rating

| Source        | method    | Type III Sum of Squares | df | Mean Square | F      | Sig. |
|---------------|-----------|-------------------------|----|-------------|--------|------|
| method        | Linear    | 7.031                   | 1  | 7.031       | 4.774  | .057 |
|               | Quadratic | 12.656                  | 1  | 12.656      | 9.878  | .012 |
|               | Cubic     | 116.281                 | 1  | 116.281     | 83.347 | .000 |
| Error(method) | Linear    | 13.256                  | 9  | 1.473       |        |      |
|               | Quadratic | 11.531                  | 9  | 1.281       |        |      |
|               | Cubic     | 12.556                  | 9  | 1.395       |        |      |

### Tests of Between-Subjects Effects

Measure: rating

Transformed Variable: Average

| Source    | Type III Sum of Squares | df | Mean Square | F        | Sig. |
|-----------|-------------------------|----|-------------|----------|------|
| Intercept | 1005.006                | 1  | 1005.006    | 1012.742 | .000 |
| Error     | 8.931                   | 9  | .992        |          |      |

### Estimated Marginal Means

method



## Estimates

Measure: rating

| method | Mean  | Std. Error | 95% Confidence Interval |             |
|--------|-------|------------|-------------------------|-------------|
|        |       |            | Lower Bound             | Upper Bound |
| 1      | 4.250 | .579       | 2.941                   | 5.559       |
| 2      | 6.550 | .189       | 6.122                   | 6.978       |
| 3      | 2.350 | .373       | 1.506                   | 3.194       |
| 4      | 6.900 | .067       | 6.749                   | 7.051       |

## Pairwise Comparisons

Measure: rating

| (I) method | (J) method | Mean Difference (I-J) | Std. Error | Sig. <sup>b</sup> | 95% Confidence Interval for Difference <sup>b</sup> |             |
|------------|------------|-----------------------|------------|-------------------|-----------------------------------------------------|-------------|
|            |            |                       |            |                   | Lower Bound                                         | Upper Bound |
| 1          | 2          | -2.300 <sup>*</sup>   | .672       | .008              | -3.819                                              | -.781       |
|            | 3          | 1.900 <sup>*</sup>    | .666       | .019              | .394                                                | 3.406       |
|            | 4          | -2.650 <sup>*</sup>   | .578       | .001              | -3.957                                              | -1.343      |
| 2          | 1          | 2.300 <sup>*</sup>    | .672       | .008              | .781                                                | 3.819       |
|            | 3          | 4.200 <sup>*</sup>    | .490       | .000              | 3.092                                               | 5.308       |
|            | 4          | -.350                 | .224       | .153              | -.857                                               | .157        |
| 3          | 1          | -1.900 <sup>*</sup>   | .666       | .019              | -3.406                                              | -.394       |
|            | 2          | -4.200 <sup>*</sup>   | .490       | .000              | -5.308                                              | -3.092      |
|            | 4          | -4.550 <sup>*</sup>   | .376       | .000              | -5.401                                              | -3.699      |
| 4          | 1          | 2.650 <sup>*</sup>    | .578       | .001              | 1.343                                               | 3.957       |
|            | 2          | .350                  | .224       | .153              | -.157                                               | .857        |
|            | 3          | 4.550 <sup>*</sup>    | .376       | .000              | 3.699                                               | 5.401       |

Based on estimated marginal means

\*. The mean difference is significant at the .05 level.

b. Adjustment for multiple comparisons: Least Significant Difference (equivalent to no adjustments).

### Multivariate Tests

|                    | Value  | F                   | Hypothesis df | Error df | Sig. |
|--------------------|--------|---------------------|---------------|----------|------|
| Pillai's trace     | .957   | 52.093 <sup>a</sup> | 3.000         | 7.000    | .000 |
| Wilks' lambda      | .043   | 52.093 <sup>a</sup> | 3.000         | 7.000    | .000 |
| Hotelling's trace  | 22.325 | 52.093 <sup>a</sup> | 3.000         | 7.000    | .000 |
| Roy's largest root | 22.325 | 52.093 <sup>a</sup> | 3.000         | 7.000    | .000 |

Each F tests the multivariate effect of method. These tests are based on the linearly independent pairwise comparisons among the estimated marginal means.

a. Exact statistic

### Profile Plots

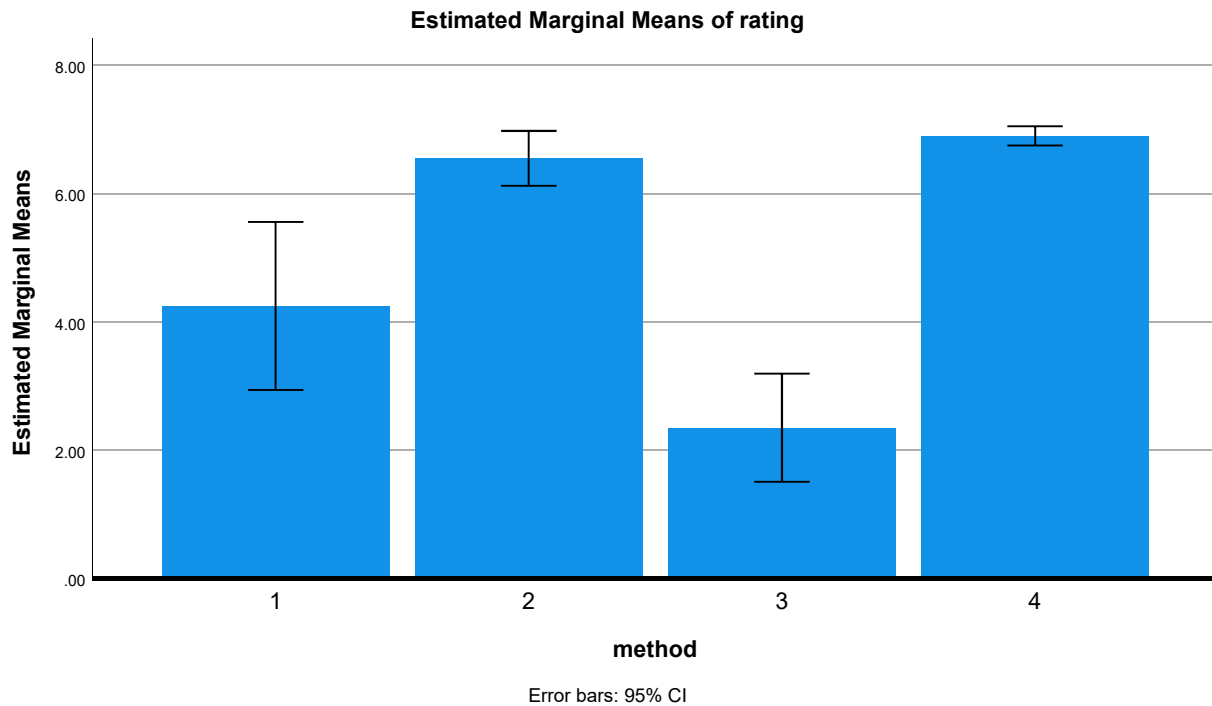

```
GLM A3 B3 C3 D3
  /WSFACTOR=method 4 Polynomial
  /MEASURE=rating
  /METHOD=SSTYPE(3)
  /PLOT=PROFILE(method) TYPE=BAR ERRORBAR=CI MEANREFERENCE=NO
  /EMMEANS=TABLES(method) COMPARE ADJ(LSD)
  /PRINT=DESCRIPTIVE
  /CRITERIA=ALPHA(.05)
  /WSDESIGN=method.
```

### General Linear Model

## Within-Subjects Factors

Measure: rating

| method | Dependent<br>Variable |
|--------|-----------------------|
| 1      | A3                    |
| 2      | B3                    |
| 3      | C3                    |
| 4      | D3                    |

## Descriptive Statistics

|    | Mean   | Std. Deviation | N  |
|----|--------|----------------|----|
| A3 | 5.4500 | 1.48043        | 10 |
| B3 | 5.3500 | 1.00139        | 10 |
| C3 | 5.7000 | .82327         | 10 |
| D3 | 6.5500 | .55025         | 10 |

## Multivariate Tests<sup>a</sup>

| Effect |                    | Value | F                  | Hypothesis df | Error df | Sig. |
|--------|--------------------|-------|--------------------|---------------|----------|------|
| method | Pillai's Trace     | .677  | 4.887 <sup>b</sup> | 3.000         | 7.000    | .039 |
|        | Wilks' Lambda      | .323  | 4.887 <sup>b</sup> | 3.000         | 7.000    | .039 |
|        | Hotelling's Trace  | 2.095 | 4.887 <sup>b</sup> | 3.000         | 7.000    | .039 |
|        | Roy's Largest Root | 2.095 | 4.887 <sup>b</sup> | 3.000         | 7.000    | .039 |

a. Design: Intercept  
Within Subjects Design: method

b. Exact statistic

### Mauchly's Test of Sphericity<sup>a</sup>

Measure: rating

| Within Subjects Effect | Mauchly's W | Approx. Chi-Square | df | Sig. | Epsilon <sup>b</sup><br>Greenhouse-Geisser |
|------------------------|-------------|--------------------|----|------|--------------------------------------------|
| method                 | .532        | 4.875              | 5  | .435 | .693                                       |

### Mauchly's Test of Sphericity<sup>a</sup>

Measure: rating

| Within Subjects Effect | Epsilon <sup>b</sup> |             |
|------------------------|----------------------|-------------|
|                        | Huynh-Feldt          | Lower-bound |
| method                 | .905                 | .333        |

Tests the null hypothesis that the error covariance matrix of the orthonormalized transformed dependent variables is proportional to an identity matrix.

a. Design: Intercept

Within Subjects Design: method

b. May be used to adjust the degrees of freedom for the averaged tests of significance. Corrected tests are displayed in the Tests of Within-Subjects Effects table.

### Tests of Within-Subjects Effects

Measure: rating

| Source        |                    | Type III Sum of Squares | df     | Mean Square | F     |
|---------------|--------------------|-------------------------|--------|-------------|-------|
| method        | Sphericity Assumed | 8.919                   | 3      | 2.973       | 3.274 |
|               | Greenhouse-Geisser | 8.919                   | 2.080  | 4.288       | 3.274 |
|               | Huynh-Feldt        | 8.919                   | 2.716  | 3.283       | 3.274 |
|               | Lower-bound        | 8.919                   | 1.000  | 8.919       | 3.274 |
| Error(method) | Sphericity Assumed | 24.519                  | 27     | .908        |       |
|               | Greenhouse-Geisser | 24.519                  | 18.719 | 1.310       |       |
|               | Huynh-Feldt        | 24.519                  | 24.448 | 1.003       |       |
|               | Lower-bound        | 24.519                  | 9.000  | 2.724       |       |

### Tests of Within-Subjects Effects

Measure: rating

| Source        |                    | Sig. |
|---------------|--------------------|------|
| method        | Sphericity Assumed | .036 |
|               | Greenhouse-Geisser | .059 |
|               | Huynh-Feldt        | .042 |
|               | Lower-bound        | .104 |
| Error(method) | Sphericity Assumed |      |
|               | Greenhouse-Geisser |      |
|               | Huynh-Feldt        |      |
|               | Lower-bound        |      |

### Tests of Within-Subjects Contrasts

Measure: rating

| Source        | method    | Type III Sum of Squares | df | Mean Square | F     | Sig. |
|---------------|-----------|-------------------------|----|-------------|-------|------|
| method        | Linear    | 6.661                   | 1  | 6.661       | 5.965 | .037 |
|               | Quadratic | 2.256                   | 1  | 2.256       | 3.220 | .106 |
|               | Cubic     | .001                    | 1  | .001        | .001  | .971 |
| Error(method) | Linear    | 10.051                  | 9  | 1.117       |       |      |
|               | Quadratic | 6.306                   | 9  | .701        |       |      |
|               | Cubic     | 8.161                   | 9  | .907        |       |      |

### Tests of Between-Subjects Effects

Measure: rating

Transformed Variable: Average

| Source    | Type III Sum of Squares | df | Mean Square | F       | Sig. |
|-----------|-------------------------|----|-------------|---------|------|
| Intercept | 1328.256                | 1  | 1328.256    | 915.600 | .000 |
| Error     | 13.056                  | 9  | 1.451       |         |      |

### Estimated Marginal Means

method

## Estimates

Measure: rating

| method | Mean  | Std. Error | 95% Confidence Interval |             |
|--------|-------|------------|-------------------------|-------------|
|        |       |            | Lower Bound             | Upper Bound |
| 1      | 5.450 | .468       | 4.391                   | 6.509       |
| 2      | 5.350 | .317       | 4.634                   | 6.066       |
| 3      | 5.700 | .260       | 5.111                   | 6.289       |
| 4      | 6.550 | .174       | 6.156                   | 6.944       |

## Pairwise Comparisons

Measure: rating

| (I) method | (J) method | Mean Difference (I-J) | Std. Error | Sig. <sup>b</sup> | 95% Confidence Interval for Difference <sup>b</sup> |             |
|------------|------------|-----------------------|------------|-------------------|-----------------------------------------------------|-------------|
|            |            |                       |            |                   | Lower Bound                                         | Upper Bound |
| 1          | 2          | .100                  | .547       | .859              | -1.137                                              | 1.337       |
|            | 3          | -.250                 | .443       | .586              | -1.251                                              | .751        |
|            | 4          | -1.100                | .521       | .064              | -2.278                                              | .078        |
| 2          | 1          | -.100                 | .547       | .859              | -1.337                                              | 1.137       |
|            | 3          | -.350                 | .366       | .363              | -1.177                                              | .477        |
|            | 4          | -1.200 <sup>*</sup>   | .300       | .003              | -1.879                                              | -.521       |
| 3          | 1          | .250                  | .443       | .586              | -.751                                               | 1.251       |
|            | 2          | .350                  | .366       | .363              | -.477                                               | 1.177       |
|            | 4          | -.850 <sup>*</sup>    | .317       | .025              | -1.566                                              | -.134       |
| 4          | 1          | 1.100                 | .521       | .064              | -.078                                               | 2.278       |
|            | 2          | 1.200 <sup>*</sup>    | .300       | .003              | .521                                                | 1.879       |
|            | 3          | .850 <sup>*</sup>     | .317       | .025              | .134                                                | 1.566       |

Based on estimated marginal means

\*. The mean difference is significant at the .05 level.

b. Adjustment for multiple comparisons: Least Significant Difference (equivalent to no adjustments).

### Multivariate Tests

|                    | Value | F                  | Hypothesis df | Error df | Sig. |
|--------------------|-------|--------------------|---------------|----------|------|
| Pillai's trace     | .677  | 4.887 <sup>a</sup> | 3.000         | 7.000    | .039 |
| Wilks' lambda      | .323  | 4.887 <sup>a</sup> | 3.000         | 7.000    | .039 |
| Hotelling's trace  | 2.095 | 4.887 <sup>a</sup> | 3.000         | 7.000    | .039 |
| Roy's largest root | 2.095 | 4.887 <sup>a</sup> | 3.000         | 7.000    | .039 |

Each F tests the multivariate effect of method. These tests are based on the linearly independent pairwise comparisons among the estimated marginal means.

a. Exact statistic

### Profile Plots

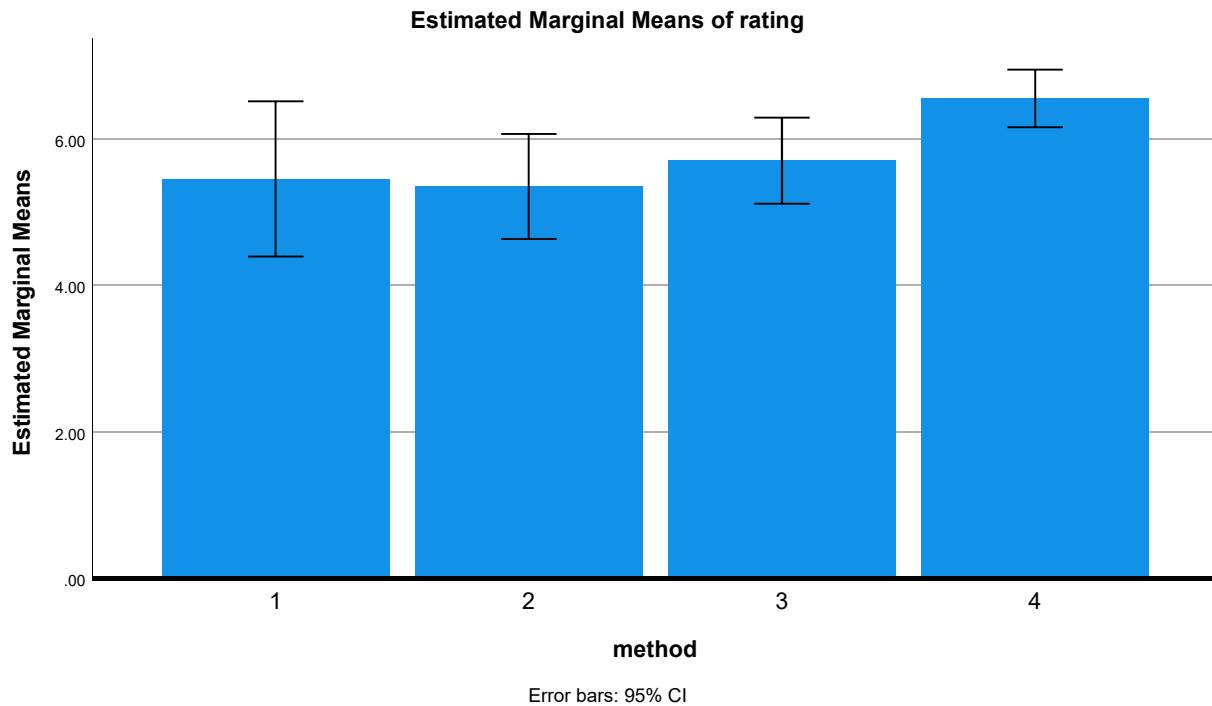

```
GLM A4 B4 C4 D4
  /WSFACTOR=method 4 Polynomial
  /MEASURE=rating
  /METHOD=SSTYPE(3)
  /PLOT=PROFILE(method) TYPE=BAR ERRORBAR=CI MEANREFERENCE=NO
  /EMMEANS=TABLES(method) COMPARE ADJ(LSD)
  /PRINT=DESCRIPTIVE
  /CRITERIA=ALPHA(.05)
  /WSDESIGN=method.
```

### General Linear Model

## Within-Subjects Factors

Measure: rating

| method | Dependent<br>Variable |
|--------|-----------------------|
| 1      | A4                    |
| 2      | B4                    |
| 3      | C4                    |
| 4      | D4                    |

## Descriptive Statistics

|    | Mean   | Std. Deviation | N  |
|----|--------|----------------|----|
| A4 | 5.6500 | 1.35503        | 10 |
| B4 | 5.3000 | .88819         | 10 |
| C4 | 5.5000 | 1.31233        | 10 |
| D4 | 6.2000 | 1.20646        | 10 |

## Multivariate Tests<sup>a</sup>

| Effect |                    | Value | F                  | Hypothesis df | Error df | Sig. |
|--------|--------------------|-------|--------------------|---------------|----------|------|
| method | Pillai's Trace     | .325  | 1.124 <sup>b</sup> | 3.000         | 7.000    | .402 |
|        | Wilks' Lambda      | .675  | 1.124 <sup>b</sup> | 3.000         | 7.000    | .402 |
|        | Hotelling's Trace  | .482  | 1.124 <sup>b</sup> | 3.000         | 7.000    | .402 |
|        | Roy's Largest Root | .482  | 1.124 <sup>b</sup> | 3.000         | 7.000    | .402 |

a. Design: Intercept  
Within Subjects Design: method

b. Exact statistic



### Mauchly's Test of Sphericity<sup>a</sup>

Measure: rating

| Within Subjects Effect | Mauchly's W | Approx. Chi-Square | df | Sig. | Epsilon <sup>b</sup><br>Greenhouse-Geisser |
|------------------------|-------------|--------------------|----|------|--------------------------------------------|
| method                 | .633        | 3.532              | 5  | .621 | .769                                       |

### Mauchly's Test of Sphericity<sup>a</sup>

Measure: rating

| Within Subjects Effect | Epsilon <sup>b</sup> |             |
|------------------------|----------------------|-------------|
|                        | Huynh-Feldt          | Lower-bound |
| method                 | 1.000                | .333        |

Tests the null hypothesis that the error covariance matrix of the orthonormalized transformed dependent variables is proportional to an identity matrix.

a. Design: Intercept

Within Subjects Design: method

b. May be used to adjust the degrees of freedom for the averaged tests of significance. Corrected tests are displayed in the Tests of Within-Subjects Effects table.

### Tests of Within-Subjects Effects

Measure: rating

| Source        |                    | Type III Sum of Squares | df     | Mean Square | F     |
|---------------|--------------------|-------------------------|--------|-------------|-------|
| method        | Sphericity Assumed | 4.469                   | 3      | 1.490       | 1.211 |
|               | Greenhouse-Geisser | 4.469                   | 2.308  | 1.936       | 1.211 |
|               | Huynh-Feldt        | 4.469                   | 3.000  | 1.490       | 1.211 |
|               | Lower-bound        | 4.469                   | 1.000  | 4.469       | 1.211 |
| Error(method) | Sphericity Assumed | 33.219                  | 27     | 1.230       |       |
|               | Greenhouse-Geisser | 33.219                  | 20.775 | 1.599       |       |
|               | Huynh-Feldt        | 33.219                  | 27.000 | 1.230       |       |
|               | Lower-bound        | 33.219                  | 9.000  | 3.691       |       |

### Tests of Within-Subjects Effects

Measure: rating

| Source        |                    | Sig. |
|---------------|--------------------|------|
| method        | Sphericity Assumed | .325 |
|               | Greenhouse-Geisser | .323 |
|               | Huynh-Feldt        | .325 |
|               | Lower-bound        | .300 |
| Error(method) | Sphericity Assumed |      |
|               | Greenhouse-Geisser |      |
|               | Huynh-Feldt        |      |
|               | Lower-bound        |      |

### Tests of Within-Subjects Contrasts

Measure: rating

| Source        | method    | Type III Sum of Squares | df | Mean Square | F     | Sig. |
|---------------|-----------|-------------------------|----|-------------|-------|------|
| method        | Linear    | 1.711                   | 1  | 1.711       | .804  | .393 |
|               | Quadratic | 2.756                   | 1  | 2.756       | 3.645 | .089 |
|               | Cubic     | .001                    | 1  | .001        | .002  | .969 |
| Error(method) | Linear    | 19.151                  | 9  | 2.128       |       |      |
|               | Quadratic | 6.806                   | 9  | .756        |       |      |
|               | Cubic     | 7.261                   | 9  | .807        |       |      |

### Tests of Between-Subjects Effects

Measure: rating

Transformed Variable: Average

| Source    | Type III Sum of Squares | df | Mean Square | F       | Sig. |
|-----------|-------------------------|----|-------------|---------|------|
| Intercept | 1282.556                | 1  | 1282.556    | 607.327 | .000 |
| Error     | 19.006                  | 9  | 2.112       |         |      |

### Estimated Marginal Means

method

## Estimates

Measure: rating

| method | Mean  | Std. Error | 95% Confidence Interval |             |
|--------|-------|------------|-------------------------|-------------|
|        |       |            | Lower Bound             | Upper Bound |
| 1      | 5.650 | .428       | 4.681                   | 6.619       |
| 2      | 5.300 | .281       | 4.665                   | 5.935       |
| 3      | 5.500 | .415       | 4.561                   | 6.439       |
| 4      | 6.200 | .382       | 5.337                   | 7.063       |

## Pairwise Comparisons

Measure: rating

| (I) method | (J) method | Mean Difference (I-J) | Std. Error | Sig. <sup>a</sup> | 95% Confidence Interval for Difference <sup>a</sup> |             |
|------------|------------|-----------------------|------------|-------------------|-----------------------------------------------------|-------------|
|            |            |                       |            |                   | Lower Bound                                         | Upper Bound |
| 1          | 2          | .350                  | .358       | .354              | -.460                                               | 1.160       |
|            | 3          | .150                  | .500       | .771              | -.982                                               | 1.282       |
|            | 4          | -.550                 | .630       | .405              | -1.975                                              | .875        |
| 2          | 1          | -.350                 | .358       | .354              | -1.160                                              | .460        |
|            | 3          | -.200                 | .436       | .657              | -1.186                                              | .786        |
|            | 4          | -.900                 | .526       | .121              | -2.090                                              | .290        |
| 3          | 1          | -.150                 | .500       | .771              | -1.282                                              | .982        |
|            | 2          | .200                  | .436       | .657              | -.786                                               | 1.186       |
|            | 4          | -.700                 | .484       | .182              | -1.795                                              | .395        |
| 4          | 1          | .550                  | .630       | .405              | -.875                                               | 1.975       |
|            | 2          | .900                  | .526       | .121              | -.290                                               | 2.090       |
|            | 3          | .700                  | .484       | .182              | -.395                                               | 1.795       |

Based on estimated marginal means

a. Adjustment for multiple comparisons: Least Significant Difference (equivalent to no adjustments).

### Multivariate Tests

|                    | Value | F                  | Hypothesis df | Error df | Sig. |
|--------------------|-------|--------------------|---------------|----------|------|
| Pillai's trace     | .325  | 1.124 <sup>a</sup> | 3.000         | 7.000    | .402 |
| Wilks' lambda      | .675  | 1.124 <sup>a</sup> | 3.000         | 7.000    | .402 |
| Hotelling's trace  | .482  | 1.124 <sup>a</sup> | 3.000         | 7.000    | .402 |
| Roy's largest root | .482  | 1.124 <sup>a</sup> | 3.000         | 7.000    | .402 |

Each F tests the multivariate effect of method. These tests are based on the linearly independent pairwise comparisons among the estimated marginal means.

a. Exact statistic

### Profile Plots

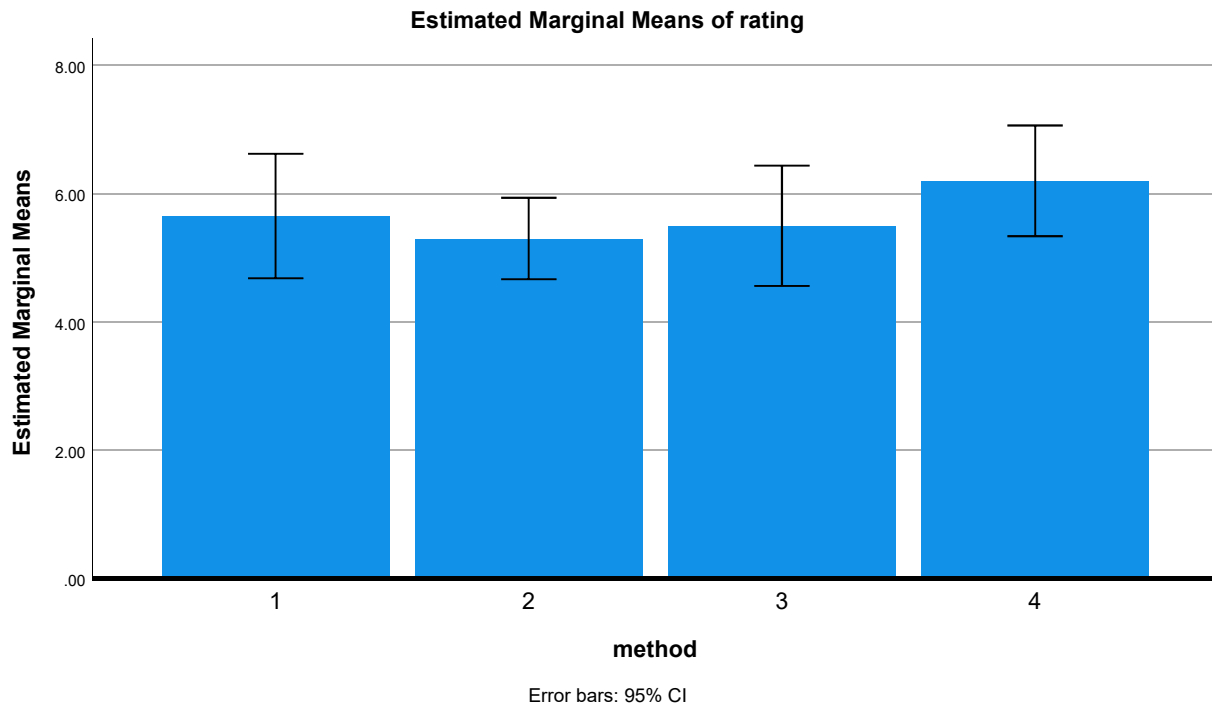

```
GLM A5 B5 C5 D5
  /WSFACTOR=method 4 Polynomial
  /MEASURE=rating
  /METHOD=SSTYPE(3)
  /PLOT=PROFILE(method) TYPE=BAR ERRORBAR=CI MEANREFERENCE=NO
  /EMMEANS=TABLES(method) COMPARE ADJ(LSD)
  /PRINT=DESCRIPTIVE
  /CRITERIA=ALPHA(.05)
  /WSDESIGN=method.
```

### General Linear Model

## Within-Subjects Factors

Measure: rating

| method | Dependent<br>Variable |
|--------|-----------------------|
| 1      | A5                    |
| 2      | B5                    |
| 3      | C5                    |
| 4      | D5                    |

## Descriptive Statistics

|    | Mean   | Std. Deviation | N  |
|----|--------|----------------|----|
| A5 | 4.9000 | 1.59513        | 10 |
| B5 | 5.6000 | 1.34990        | 10 |
| C5 | 4.7000 | 1.49443        | 10 |
| D5 | 6.7000 | .48305         | 10 |

## Multivariate Tests<sup>a</sup>

| Effect |                    | Value | F                   | Hypothesis df | Error df | Sig. |
|--------|--------------------|-------|---------------------|---------------|----------|------|
| method | Pillai's Trace     | .877  | 16.639 <sup>b</sup> | 3.000         | 7.000    | .001 |
|        | Wilks' Lambda      | .123  | 16.639 <sup>b</sup> | 3.000         | 7.000    | .001 |
|        | Hotelling's Trace  | 7.131 | 16.639 <sup>b</sup> | 3.000         | 7.000    | .001 |
|        | Roy's Largest Root | 7.131 | 16.639 <sup>b</sup> | 3.000         | 7.000    | .001 |

a. Design: Intercept  
Within Subjects Design: method

b. Exact statistic

### Mauchly's Test of Sphericity<sup>a</sup>

Measure: rating

| Within Subjects Effect | Mauchly's W | Approx. Chi-Square | df | Sig. | Epsilon <sup>b</sup><br>Greenhouse-Geisser |
|------------------------|-------------|--------------------|----|------|--------------------------------------------|
| method                 | .256        | 10.515             | 5  | .064 | .687                                       |

### Mauchly's Test of Sphericity<sup>a</sup>

Measure: rating

| Within Subjects Effect | Epsilon <sup>b</sup> |             |
|------------------------|----------------------|-------------|
|                        | Huynh-Feldt          | Lower-bound |
| method                 | .895                 | .333        |

Tests the null hypothesis that the error covariance matrix of the orthonormalized transformed dependent variables is proportional to an identity matrix.

a. Design: Intercept

Within Subjects Design: method

b. May be used to adjust the degrees of freedom for the averaged tests of significance. Corrected tests are displayed in the Tests of Within-Subjects Effects table.

### Tests of Within-Subjects Effects

Measure: rating

| Source        |                    | Type III Sum of Squares | df     | Mean Square | F     |
|---------------|--------------------|-------------------------|--------|-------------|-------|
| method        | Sphericity Assumed | 24.475                  | 3      | 8.158       | 4.381 |
|               | Greenhouse-Geisser | 24.475                  | 2.062  | 11.868      | 4.381 |
|               | Huynh-Feldt        | 24.475                  | 2.684  | 9.118       | 4.381 |
|               | Lower-bound        | 24.475                  | 1.000  | 24.475      | 4.381 |
| Error(method) | Sphericity Assumed | 50.275                  | 27     | 1.862       |       |
|               | Greenhouse-Geisser | 50.275                  | 18.560 | 2.709       |       |
|               | Huynh-Feldt        | 50.275                  | 24.157 | 2.081       |       |
|               | Lower-bound        | 50.275                  | 9.000  | 5.586       |       |

### Tests of Within-Subjects Effects

Measure: rating

| Source        |                    | Sig. |
|---------------|--------------------|------|
| method        | Sphericity Assumed | .012 |
|               | Greenhouse-Geisser | .027 |
|               | Huynh-Feldt        | .016 |
|               | Lower-bound        | .066 |
| Error(method) | Sphericity Assumed |      |
|               | Greenhouse-Geisser |      |
|               | Huynh-Feldt        |      |
|               | Lower-bound        |      |

### Tests of Within-Subjects Contrasts

Measure: rating

| Source        | method    | Type III Sum of Squares | df | Mean Square | F     | Sig. |
|---------------|-----------|-------------------------|----|-------------|-------|------|
| method        | Linear    | 10.125                  | 1  | 10.125      | 5.200 | .049 |
|               | Quadratic | 4.225                   | 1  | 4.225       | 6.311 | .033 |
|               | Cubic     | 10.125                  | 1  | 10.125      | 3.410 | .098 |
| Error(method) | Linear    | 17.525                  | 9  | 1.947       |       |      |
|               | Quadratic | 6.025                   | 9  | .669        |       |      |
|               | Cubic     | 26.725                  | 9  | 2.969       |       |      |

### Tests of Between-Subjects Effects

Measure: rating

Transformed Variable: Average

| Source    | Type III Sum of Squares | df | Mean Square | F       | Sig. |
|-----------|-------------------------|----|-------------|---------|------|
| Intercept | 1199.025                | 1  | 1199.025    | 961.356 | .000 |
| Error     | 11.225                  | 9  | 1.247       |         |      |

### Estimated Marginal Means

method

## Estimates

Measure: rating

| method | Mean  | Std. Error | 95% Confidence Interval |             |
|--------|-------|------------|-------------------------|-------------|
|        |       |            | Lower Bound             | Upper Bound |
| 1      | 4.900 | .504       | 3.759                   | 6.041       |
| 2      | 5.600 | .427       | 4.634                   | 6.566       |
| 3      | 4.700 | .473       | 3.631                   | 5.769       |
| 4      | 6.700 | .153       | 6.354                   | 7.046       |

## Pairwise Comparisons

Measure: rating

| (I) method | (J) method | Mean Difference (I-J) | Std. Error | Sig. <sup>b</sup> | 95% Confidence Interval for Difference <sup>b</sup> |             |
|------------|------------|-----------------------|------------|-------------------|-----------------------------------------------------|-------------|
|            |            |                       |            |                   | Lower Bound                                         | Upper Bound |
| 1          | 2          | -.700                 | .633       | .298              | -2.133                                              | .733        |
|            | 3          | .200                  | .663       | .770              | -1.301                                              | 1.701       |
|            | 4          | -1.800*               | .573       | .012              | -3.097                                              | -.503       |
| 2          | 1          | .700                  | .633       | .298              | -.733                                               | 2.133       |
|            | 3          | .900                  | .809       | .295              | -.930                                               | 2.730       |
|            | 4          | -1.100*               | .482       | .048              | -2.190                                              | -.010       |
| 3          | 1          | -.200                 | .663       | .770              | -1.701                                              | 1.301       |
|            | 2          | -.900                 | .809       | .295              | -2.730                                              | .930        |
|            | 4          | -2.000*               | .422       | .001              | -2.954                                              | -1.046      |
| 4          | 1          | 1.800*                | .573       | .012              | .503                                                | 3.097       |
|            | 2          | 1.100*                | .482       | .048              | .010                                                | 2.190       |
|            | 3          | 2.000*                | .422       | .001              | 1.046                                               | 2.954       |

Based on estimated marginal means

\*. The mean difference is significant at the .05 level.

b. Adjustment for multiple comparisons: Least Significant Difference (equivalent to no adjustments).



### Multivariate Tests

|                    | Value | F                   | Hypothesis df | Error df | Sig. |
|--------------------|-------|---------------------|---------------|----------|------|
| Pillai's trace     | .877  | 16.639 <sup>a</sup> | 3.000         | 7.000    | .001 |
| Wilks' lambda      | .123  | 16.639 <sup>a</sup> | 3.000         | 7.000    | .001 |
| Hotelling's trace  | 7.131 | 16.639 <sup>a</sup> | 3.000         | 7.000    | .001 |
| Roy's largest root | 7.131 | 16.639 <sup>a</sup> | 3.000         | 7.000    | .001 |

Each F tests the multivariate effect of method. These tests are based on the linearly independent pairwise comparisons among the estimated marginal means.

a. Exact statistic

### Profile Plots

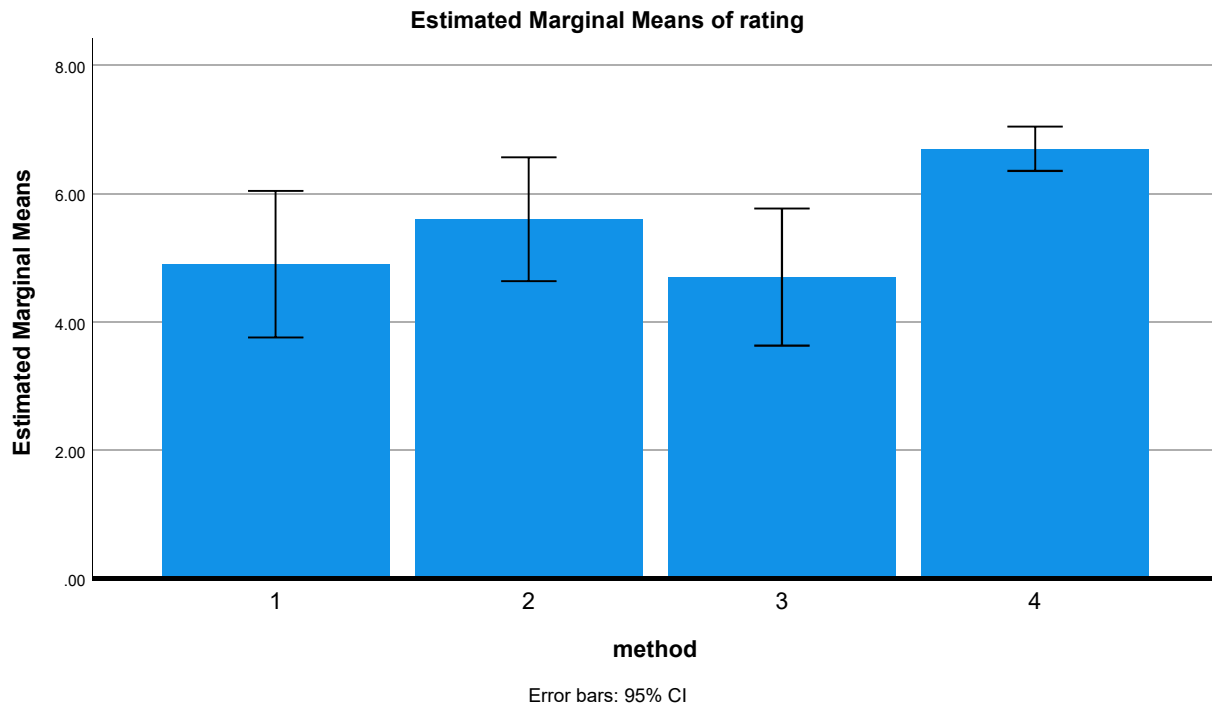

Supplement: Supplementary file 4 [file subjective.pdf]
