# Supplementary material for: Communicating Inferred Goals with Passive Augmented Reality and Active Haptic Feedback
Source: arXiv:2109.01747 source file (2021-09-03)

```

GLM A1 B1 C1 D1
  /WSFACTOR=method 4 Polynomial
  /MEASURE=teaching_efficiency
  /METHOD=SSTYPE(3)
  /PLOT=PROFILE(method) TYPE=BAR ERRORBAR=CI MEANREFERENCE=NO
  /EMMEANS=TABLES(method) COMPARE ADJ(LSD)
  /PRINT=DESCRIPTIVE
  /CRITERIA=ALPHA(.05)
  /WSDSIGN=method.

```

## General Linear Model

### Within-Subjects Factors

Measure: teaching\_efficiency

| method | Dependent<br>Variable |
|--------|-----------------------|
| 1      | A1                    |
| 2      | B1                    |
| 3      | C1                    |
| 4      | D1                    |

### Descriptive Statistics

|    | Mean  | Std. Deviation | N   |
|----|-------|----------------|-----|
| A1 | .0761 | .01974         | 380 |
| B1 | .0873 | .00752         | 380 |
| C1 | .0762 | .01823         | 380 |
| D1 | .0874 | .01321         | 380 |

### Multivariate Tests<sup>a</sup>

| Effect |                    | Value | F                    | Hypothesis df | Error df | Sig. |
|--------|--------------------|-------|----------------------|---------------|----------|------|
| method | Pillai's Trace     | .455  | 104.866 <sup>b</sup> | 3.000         | 377.000  | .000 |
|        | Wilks' Lambda      | .545  | 104.866 <sup>b</sup> | 3.000         | 377.000  | .000 |
|        | Hotelling's Trace  | .834  | 104.866 <sup>b</sup> | 3.000         | 377.000  | .000 |
|        | Roy's Largest Root | .834  | 104.866 <sup>b</sup> | 3.000         | 377.000  | .000 |

a. Design: Intercept  
Within Subjects Design: method

b. Exact statistic

### Mauchly's Test of Sphericity<sup>a</sup>

Measure: teaching\_efficiency

| Within Subjects Effect | Mauchly's W | Approx. Chi-Square | df | Sig. | Epsilon <sup>b</sup><br>Greenhouse-Geisser |
|------------------------|-------------|--------------------|----|------|--------------------------------------------|
| method                 | .547        | 227.623            | 5  | .000 | .761                                       |

### Mauchly's Test of Sphericity<sup>a</sup>

Measure: teaching\_efficiency

| Within Subjects Effect | Epsilon <sup>b</sup> |             |
|------------------------|----------------------|-------------|
|                        | Huynh-Feldt          | Lower-bound |
| method                 | .766                 | .333        |

Tests the null hypothesis that the error covariance matrix of the orthonormalized transformed dependent variables is proportional to an identity matrix.

a. Design: Intercept

Within Subjects Design: method

b. May be used to adjust the degrees of freedom for the averaged tests of significance. Corrected tests are displayed in the Tests of Within-Subjects Effects table.

### Tests of Within-Subjects Effects

Measure: teaching\_efficiency

| Source        |                    | Type III Sum of Squares | df      | Mean Square | F      |
|---------------|--------------------|-------------------------|---------|-------------|--------|
| method        | Sphericity Assumed | .048                    | 3       | .016        | 80.713 |
|               | Greenhouse-Geisser | .048                    | 2.283   | .021        | 80.713 |
|               | Huynh-Feldt        | .048                    | 2.297   | .021        | 80.713 |
|               | Lower-bound        | .048                    | 1.000   | .048        | 80.713 |
| Error(method) | Sphericity Assumed | .225                    | 1137    | .000        |        |
|               | Greenhouse-Geisser | .225                    | 865.117 | .000        |        |
|               | Huynh-Feldt        | .225                    | 870.643 | .000        |        |
|               | Lower-bound        | .225                    | 379.000 | .001        |        |

### Tests of Within-Subjects Effects

Measure: teaching\_efficiency

| Source        |                    | Sig. |
|---------------|--------------------|------|
| method        | Sphericity Assumed | .000 |
|               | Greenhouse-Geisser | .000 |
|               | Huynh-Feldt        | .000 |
|               | Lower-bound        | .000 |
| Error(method) | Sphericity Assumed |      |
|               | Greenhouse-Geisser |      |
|               | Huynh-Feldt        |      |
|               | Lower-bound        |      |

### Tests of Within-Subjects Contrasts

Measure: teaching\_efficiency

| Source        | method    | Type III Sum of Squares | df  | Mean Square | F       | Sig. |
|---------------|-----------|-------------------------|-----|-------------|---------|------|
| method        | Linear    | .010                    | 1   | .010        | 111.348 | .000 |
|               | Quadratic | 5.794E-7                | 1   | 5.794E-7    | .002    | .965 |
|               | Cubic     | .038                    | 1   | .038        | 182.203 | .000 |
| Error(method) | Linear    | .034                    | 379 | 8.950E-5    |         |      |
|               | Quadratic | .112                    | 379 | .000        |         |      |
|               | Cubic     | .079                    | 379 | .000        |         |      |

### Tests of Between-Subjects Effects

Measure: teaching\_efficiency

Transformed Variable: Average

| Source    | Type III Sum of Squares | df  | Mean Square | F         | Sig. |
|-----------|-------------------------|-----|-------------|-----------|------|
| Intercept | 10.154                  | 1   | 10.154      | 28198.946 | .000 |
| Error     | .136                    | 379 | .000        |           |      |

### Estimated Marginal Means

method

## Estimates

Measure: teaching\_efficiency

| method | Mean | Std. Error | 95% Confidence Interval |             |
|--------|------|------------|-------------------------|-------------|
|        |      |            | Lower Bound             | Upper Bound |
| 1      | .076 | .001       | .074                    | .078        |
| 2      | .087 | .000       | .087                    | .088        |
| 3      | .076 | .001       | .074                    | .078        |
| 4      | .087 | .001       | .086                    | .089        |

## Pairwise Comparisons

Measure: teaching\_efficiency

| (I) method | (J) method | Mean Difference (I-J) | Std. Error | Sig. <sup>b</sup> | 95% Confidence Interval for Difference <sup>b</sup> |             |
|------------|------------|-----------------------|------------|-------------------|-----------------------------------------------------|-------------|
|            |            |                       |            |                   | Lower Bound                                         | Upper Bound |
| 1          | 2          | -.011 <sup>*</sup>    | .001       | .000              | -.013                                               | -.009       |
|            | 3          | -7.549E-5             | .001       | .952              | -.003                                               | .002        |
|            | 4          | -.011 <sup>*</sup>    | .001       | .000              | -.013                                               | -.010       |
| 2          | 1          | .011 <sup>*</sup>     | .001       | .000              | .009                                                | .013        |
|            | 3          | .011 <sup>*</sup>     | .001       | .000              | .009                                                | .013        |
|            | 4          | .000                  | .001       | .847              | -.002                                               | .001        |
| 3          | 1          | 7.549E-5              | .001       | .952              | -.002                                               | .003        |
|            | 2          | -.011 <sup>*</sup>    | .001       | .000              | -.013                                               | -.009       |
|            | 4          | -.011 <sup>*</sup>    | .001       | .000              | -.014                                               | -.009       |
| 4          | 1          | .011 <sup>*</sup>     | .001       | .000              | .010                                                | .013        |
|            | 2          | .000                  | .001       | .847              | -.001                                               | .002        |
|            | 3          | .011 <sup>*</sup>     | .001       | .000              | .009                                                | .014        |

Based on estimated marginal means

\*. The mean difference is significant at the .05 level.

b. Adjustment for multiple comparisons: Least Significant Difference (equivalent to no adjustments).

### Multivariate Tests

|                    | Value | F                    | Hypothesis df | Error df | Sig. |
|--------------------|-------|----------------------|---------------|----------|------|
| Pillai's trace     | .455  | 104.866 <sup>a</sup> | 3.000         | 377.000  | .000 |
| Wilks' lambda      | .545  | 104.866 <sup>a</sup> | 3.000         | 377.000  | .000 |
| Hotelling's trace  | .834  | 104.866 <sup>a</sup> | 3.000         | 377.000  | .000 |
| Roy's largest root | .834  | 104.866 <sup>a</sup> | 3.000         | 377.000  | .000 |

Each F tests the multivariate effect of method. These tests are based on the linearly independent pairwise comparisons among the estimated marginal means.

a. Exact statistic

### Profile Plots

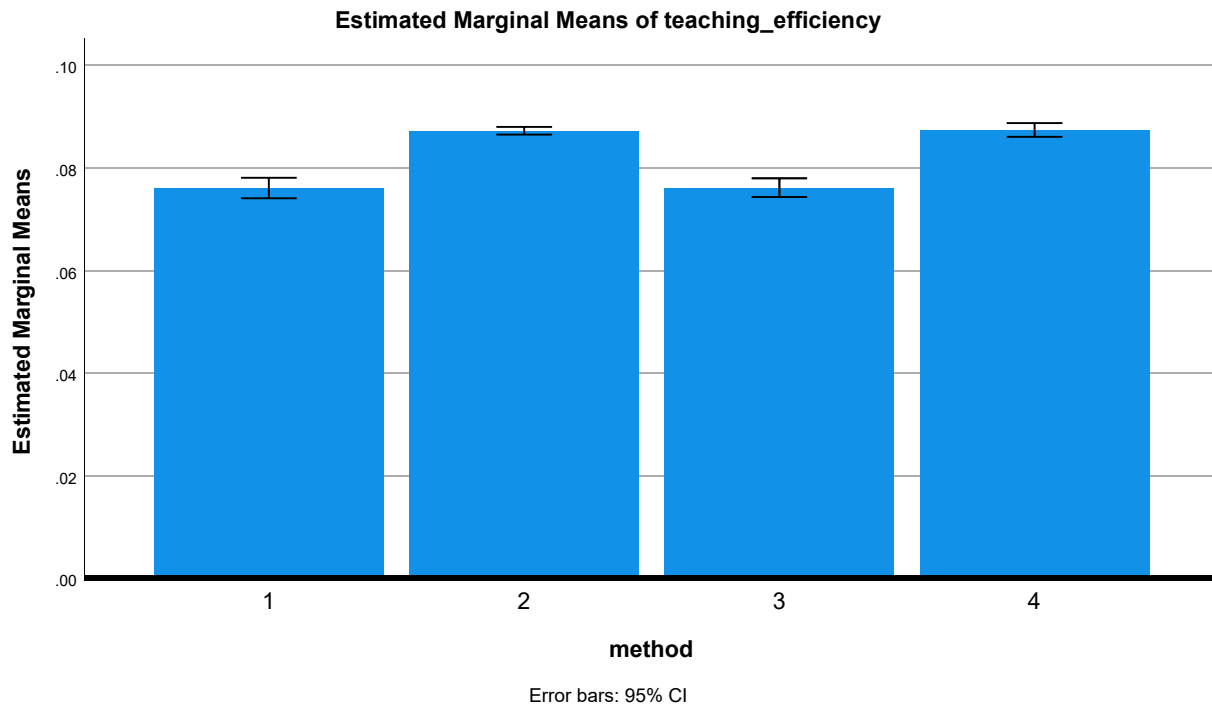

```
GLM A2 B2 C2 D2
  /WSFACTOR=method 4 Polynomial
  /MEASURE=teaching_efficiency
  /METHOD=SSTYPE(3)
  /PLOT=PROFILE(method) TYPE=BAR ERRORBAR=CI MEANREFERENCE=NO
  /EMMEANS=TABLES(method) COMPARE ADJ(LSD)
  /PRINT=DESCRIPTIVE
  /CRITERIA=ALPHA(.05)
  /WSDESIGN=method.
```

### General Linear Model

## Within-Subjects Factors

Measure: teaching\_efficiency

| method | Dependent<br>Variable |
|--------|-----------------------|
| 1      | A2                    |
| 2      | B2                    |
| 3      | C2                    |
| 4      | D2                    |

## Descriptive Statistics

|    | Mean  | Std. Deviation | N   |
|----|-------|----------------|-----|
| A2 | .2345 | .07025         | 380 |
| B2 | .2603 | .07313         | 380 |
| C2 | .3014 | .07901         | 380 |
| D2 | .3338 | .04332         | 380 |

## Multivariate Tests<sup>a</sup>

| Effect |                    | Value | F                    | Hypothesis df | Error df | Sig. |
|--------|--------------------|-------|----------------------|---------------|----------|------|
| method | Pillai's Trace     | .676  | 261.824 <sup>b</sup> | 3.000         | 377.000  | .000 |
|        | Wilks' Lambda      | .324  | 261.824 <sup>b</sup> | 3.000         | 377.000  | .000 |
|        | Hotelling's Trace  | 2.083 | 261.824 <sup>b</sup> | 3.000         | 377.000  | .000 |
|        | Roy's Largest Root | 2.083 | 261.824 <sup>b</sup> | 3.000         | 377.000  | .000 |

a. Design: Intercept  
Within Subjects Design: method

b. Exact statistic

### Mauchly's Test of Sphericity<sup>a</sup>

Measure: teaching\_efficiency

| Within Subjects Effect | Mauchly's W | Approx. Chi-Square | df | Sig. | Epsilon <sup>b</sup><br>Greenhouse-Geisser |
|------------------------|-------------|--------------------|----|------|--------------------------------------------|
| method                 | .275        | 487.904            | 5  | .000 | .643                                       |

### Mauchly's Test of Sphericity<sup>a</sup>

Measure: teaching\_efficiency

| Within Subjects Effect | Huynh-Feldt | Epsilon <sup>b</sup><br>Lower-bound |
|------------------------|-------------|-------------------------------------|
| method                 | .646        | .333                                |

Tests the null hypothesis that the error covariance matrix of the orthonormalized transformed dependent variables is proportional to an identity matrix.

a. Design: Intercept

Within Subjects Design: method

b. May be used to adjust the degrees of freedom for the averaged tests of significance. Corrected tests are displayed in the Tests of Within-Subjects Effects table.

### Tests of Within-Subjects Effects

Measure: teaching\_efficiency

| Source        |                    | Type III Sum of Squares | df      | Mean Square | F       |
|---------------|--------------------|-------------------------|---------|-------------|---------|
| method        | Sphericity Assumed | 2.201                   | 3       | .734        | 177.123 |
|               | Greenhouse-Geisser | 2.201                   | 1.929   | 1.141       | 177.123 |
|               | Huynh-Feldt        | 2.201                   | 1.938   | 1.135       | 177.123 |
|               | Lower-bound        | 2.201                   | 1.000   | 2.201       | 177.123 |
| Error(method) | Sphericity Assumed | 4.709                   | 1137    | .004        |         |
|               | Greenhouse-Geisser | 4.709                   | 730.994 | .006        |         |
|               | Huynh-Feldt        | 4.709                   | 734.661 | .006        |         |
|               | Lower-bound        | 4.709                   | 379.000 | .012        |         |

### Tests of Within-Subjects Effects

Measure: teaching\_efficiency

| Source        |                    | Sig. |
|---------------|--------------------|------|
| method        | Sphericity Assumed | .000 |
|               | Greenhouse-Geisser | .000 |
|               | Huynh-Feldt        | .000 |
|               | Lower-bound        | .000 |
| Error(method) | Sphericity Assumed |      |
|               | Greenhouse-Geisser |      |
|               | Huynh-Feldt        |      |
|               | Lower-bound        |      |

### Tests of Within-Subjects Contrasts

Measure: teaching\_efficiency

| Source        | method    | Type III Sum of Squares | df  | Mean Square | F       | Sig. |
|---------------|-----------|-------------------------|-----|-------------|---------|------|
| method        | Linear    | 2.186                   | 1   | 2.186       | 574.355 | .000 |
|               | Quadratic | .004                    | 1   | .004        | 4.692   | .031 |
|               | Cubic     | .011                    | 1   | .011        | 1.422   | .234 |
| Error(method) | Linear    | 1.442                   | 379 | .004        |         |      |
|               | Quadratic | .335                    | 379 | .001        |         |      |
|               | Cubic     | 2.932                   | 379 | .008        |         |      |

### Tests of Between-Subjects Effects

Measure: teaching\_efficiency

Transformed Variable: Average

| Source    | Type III Sum of Squares | df  | Mean Square | F         | Sig. |
|-----------|-------------------------|-----|-------------|-----------|------|
| Intercept | 121.305                 | 1   | 121.305     | 20296.262 | .000 |
| Error     | 2.265                   | 379 | .006        |           |      |

### Estimated Marginal Means

method



### Estimates

Measure: teaching\_efficiency

| method | Mean | Std. Error | 95% Confidence Interval |             |
|--------|------|------------|-------------------------|-------------|
|        |      |            | Lower Bound             | Upper Bound |
| 1      | .234 | .004       | .227                    | .242        |
| 2      | .260 | .004       | .253                    | .268        |
| 3      | .301 | .004       | .293                    | .309        |
| 4      | .334 | .002       | .329                    | .338        |

### Pairwise Comparisons

Measure: teaching\_efficiency

| (I) method | (J) method | Mean Difference (I-J) | Std. Error | Sig. <sup>b</sup> | 95% Confidence Interval for Difference <sup>b</sup> |             |
|------------|------------|-----------------------|------------|-------------------|-----------------------------------------------------|-------------|
|            |            |                       |            |                   | Lower Bound                                         | Upper Bound |
| 1          | 2          | -.026 <sup>*</sup>    | .005       | .000              | -.035                                               | -.017       |
|            | 3          | -.067 <sup>*</sup>    | .004       | .000              | -.076                                               | -.058       |
|            | 4          | -.099 <sup>*</sup>    | .004       | .000              | -.108                                               | -.091       |
| 2          | 1          | .026 <sup>*</sup>     | .005       | .000              | .017                                                | .035        |
|            | 3          | -.041 <sup>*</sup>    | .007       | .000              | -.054                                               | -.028       |
|            | 4          | -.074 <sup>*</sup>    | .004       | .000              | -.081                                               | -.066       |
| 3          | 1          | .067 <sup>*</sup>     | .004       | .000              | .058                                                | .076        |
|            | 2          | .041 <sup>*</sup>     | .007       | .000              | .028                                                | .054        |
|            | 4          | -.032 <sup>*</sup>    | .004       | .000              | -.040                                               | -.025       |
| 4          | 1          | .099 <sup>*</sup>     | .004       | .000              | .091                                                | .108        |
|            | 2          | .074 <sup>*</sup>     | .004       | .000              | .066                                                | .081        |
|            | 3          | .032 <sup>*</sup>     | .004       | .000              | .025                                                | .040        |

Based on estimated marginal means

\*. The mean difference is significant at the .05 level.

b. Adjustment for multiple comparisons: Least Significant Difference (equivalent to no adjustments).

### Multivariate Tests

|                    | Value | F                    | Hypothesis df | Error df | Sig. |
|--------------------|-------|----------------------|---------------|----------|------|
| Pillai's trace     | .676  | 261.824 <sup>a</sup> | 3.000         | 377.000  | .000 |
| Wilks' lambda      | .324  | 261.824 <sup>a</sup> | 3.000         | 377.000  | .000 |
| Hotelling's trace  | 2.083 | 261.824 <sup>a</sup> | 3.000         | 377.000  | .000 |
| Roy's largest root | 2.083 | 261.824 <sup>a</sup> | 3.000         | 377.000  | .000 |

Each F tests the multivariate effect of method. These tests are based on the linearly independent pairwise comparisons among the estimated marginal means.

a. Exact statistic

### Profile Plots

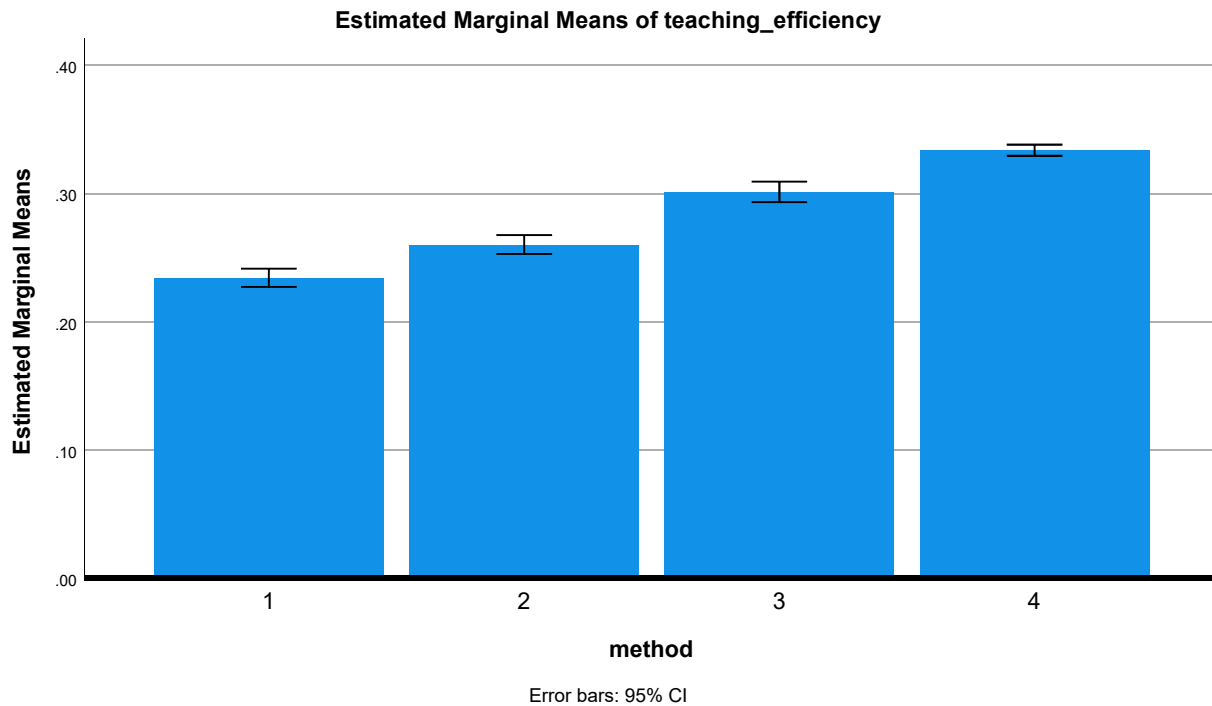

```
GLM A3 B3 C3 D3
  /WSFACTOR=method 4 Polynomial
  /MEASURE=teaching_efficiency
  /METHOD=SSTYPE(3)
  /PLOT=PROFILE(method) TYPE=BAR ERRORBAR=CI MEANREFERENCE=NO
  /EMMEANS=TABLES(method) COMPARE ADJ(LSD)
  /PRINT=DESCRIPTIVE
  /CRITERIA=ALPHA(.05)
  /WSDESIGN=method.
```

### General Linear Model

## Within-Subjects Factors

Measure: teaching\_efficiency

| method | Dependent<br>Variable |
|--------|-----------------------|
| 1      | A3                    |
| 2      | B3                    |
| 3      | C3                    |
| 4      | D3                    |

## Descriptive Statistics

|    | Mean  | Std. Deviation | N   |
|----|-------|----------------|-----|
| A3 | .4215 | .12982         | 380 |
| B3 | .3685 | .15784         | 380 |
| C3 | .4249 | .18035         | 380 |
| D3 | .6127 | .24809         | 380 |

## Multivariate Tests<sup>a</sup>

| Effect |                    | Value | F                    | Hypothesis df | Error df | Sig. |
|--------|--------------------|-------|----------------------|---------------|----------|------|
| method | Pillai's Trace     | .491  | 121.369 <sup>b</sup> | 3.000         | 377.000  | .000 |
|        | Wilks' Lambda      | .509  | 121.369 <sup>b</sup> | 3.000         | 377.000  | .000 |
|        | Hotelling's Trace  | .966  | 121.369 <sup>b</sup> | 3.000         | 377.000  | .000 |
|        | Roy's Largest Root | .966  | 121.369 <sup>b</sup> | 3.000         | 377.000  | .000 |

a. Design: Intercept  
Within Subjects Design: method

b. Exact statistic

### Mauchly's Test of Sphericity<sup>a</sup>

Measure: teaching\_efficiency

| Within Subjects Effect | Mauchly's W | Approx. Chi-Square | df | Sig. | Epsilon <sup>b</sup><br>Greenhouse-Geisser |
|------------------------|-------------|--------------------|----|------|--------------------------------------------|
| method                 | .291        | 466.433            | 5  | .000 | .625                                       |

### Mauchly's Test of Sphericity<sup>a</sup>

Measure: teaching\_efficiency

| Within Subjects Effect | Huynh-Feldt | Epsilon <sup>b</sup><br>Lower-bound |
|------------------------|-------------|-------------------------------------|
| method                 | .628        | .333                                |

Tests the null hypothesis that the error covariance matrix of the orthonormalized transformed dependent variables is proportional to an identity matrix.

a. Design: Intercept

Within Subjects Design: method

b. May be used to adjust the degrees of freedom for the averaged tests of significance. Corrected tests are displayed in the Tests of Within-Subjects Effects table.

### Tests of Within-Subjects Effects

Measure: teaching\_efficiency

| Source        |                    | Type III Sum of Squares | df      | Mean Square | F       |
|---------------|--------------------|-------------------------|---------|-------------|---------|
| method        | Sphericity Assumed | 13.063                  | 3       | 4.354       | 146.218 |
|               | Greenhouse-Geisser | 13.063                  | 1.876   | 6.965       | 146.218 |
|               | Huynh-Feldt        | 13.063                  | 1.885   | 6.931       | 146.218 |
|               | Lower-bound        | 13.063                  | 1.000   | 13.063      | 146.218 |
| Error(method) | Sphericity Assumed | 33.859                  | 1137    | .030        |         |
|               | Greenhouse-Geisser | 33.859                  | 710.855 | .048        |         |
|               | Huynh-Feldt        | 33.859                  | 714.265 | .047        |         |
|               | Lower-bound        | 33.859                  | 379.000 | .089        |         |

### Tests of Within-Subjects Effects

Measure: teaching\_efficiency

| Source        |                    | Sig. |
|---------------|--------------------|------|
| method        | Sphericity Assumed | .000 |
|               | Greenhouse-Geisser | .000 |
|               | Huynh-Feldt        | .000 |
|               | Lower-bound        | .000 |
| Error(method) | Sphericity Assumed |      |
|               | Greenhouse-Geisser |      |
|               | Huynh-Feldt        |      |
|               | Lower-bound        |      |

### Tests of Within-Subjects Contrasts

Measure: teaching\_efficiency

| Source        | method    | Type III Sum of Squares | df  | Mean Square | F       | Sig. |
|---------------|-----------|-------------------------|-----|-------------|---------|------|
| method        | Linear    | 7.546                   | 1   | 7.546       | 156.846 | .000 |
|               | Quadratic | 5.508                   | 1   | 5.508       | 298.572 | .000 |
|               | Cubic     | .009                    | 1   | .009        | .400    | .527 |
| Error(method) | Linear    | 18.234                  | 379 | .048        |         |      |
|               | Quadratic | 6.992                   | 379 | .018        |         |      |
|               | Cubic     | 8.634                   | 379 | .023        |         |      |

### Tests of Between-Subjects Effects

Measure: teaching\_efficiency

Transformed Variable: Average

| Source    | Type III Sum of Squares | df  | Mean Square | F        | Sig. |
|-----------|-------------------------|-----|-------------|----------|------|
| Intercept | 317.321                 | 1   | 317.321     | 6823.236 | .000 |
| Error     | 17.626                  | 379 | .047        |          |      |

### Estimated Marginal Means

method

## Estimates

Measure: teaching\_efficiency

| method | Mean | Std. Error | 95% Confidence Interval |             |
|--------|------|------------|-------------------------|-------------|
|        |      |            | Lower Bound             | Upper Bound |
| 1      | .421 | .007       | .408                    | .435        |
| 2      | .368 | .008       | .353                    | .384        |
| 3      | .425 | .009       | .407                    | .443        |
| 4      | .613 | .013       | .588                    | .638        |

## Pairwise Comparisons

Measure: teaching\_efficiency

| (I) method | (J) method | Mean Difference (I-J) | Std. Error | Sig. <sup>b</sup> | 95% Confidence Interval for Difference <sup>b</sup> |             |
|------------|------------|-----------------------|------------|-------------------|-----------------------------------------------------|-------------|
|            |            |                       |            |                   | Lower Bound                                         | Upper Bound |
| 1          | 2          | .053 <sup>*</sup>     | .006       | .000              | .041                                                | .065        |
|            | 3          | -.003                 | .013       | .791              | -.029                                               | .022        |
|            | 4          | -.191 <sup>*</sup>    | .013       | .000              | -.217                                               | -.165       |
| 2          | 1          | -.053 <sup>*</sup>    | .006       | .000              | -.065                                               | -.041       |
|            | 3          | -.056 <sup>*</sup>    | .014       | .000              | -.084                                               | -.029       |
|            | 4          | -.244 <sup>*</sup>    | .016       | .000              | -.275                                               | -.214       |
| 3          | 1          | .003                  | .013       | .791              | -.022                                               | .029        |
|            | 2          | .056 <sup>*</sup>     | .014       | .000              | .029                                                | .084        |
|            | 4          | -.188 <sup>*</sup>    | .011       | .000              | -.209                                               | -.166       |
| 4          | 1          | .191 <sup>*</sup>     | .013       | .000              | .165                                                | .217        |
|            | 2          | .244 <sup>*</sup>     | .016       | .000              | .214                                                | .275        |
|            | 3          | .188 <sup>*</sup>     | .011       | .000              | .166                                                | .209        |

Based on estimated marginal means

\*. The mean difference is significant at the .05 level.

b. Adjustment for multiple comparisons: Least Significant Difference (equivalent to no adjustments).

### Multivariate Tests

|                    | Value | F                    | Hypothesis df | Error df | Sig. |
|--------------------|-------|----------------------|---------------|----------|------|
| Pillai's trace     | .491  | 121.369 <sup>a</sup> | 3.000         | 377.000  | .000 |
| Wilks' lambda      | .509  | 121.369 <sup>a</sup> | 3.000         | 377.000  | .000 |
| Hotelling's trace  | .966  | 121.369 <sup>a</sup> | 3.000         | 377.000  | .000 |
| Roy's largest root | .966  | 121.369 <sup>a</sup> | 3.000         | 377.000  | .000 |

Each F tests the multivariate effect of method. These tests are based on the linearly independent pairwise comparisons among the estimated marginal means.

a. Exact statistic

### Profile Plots

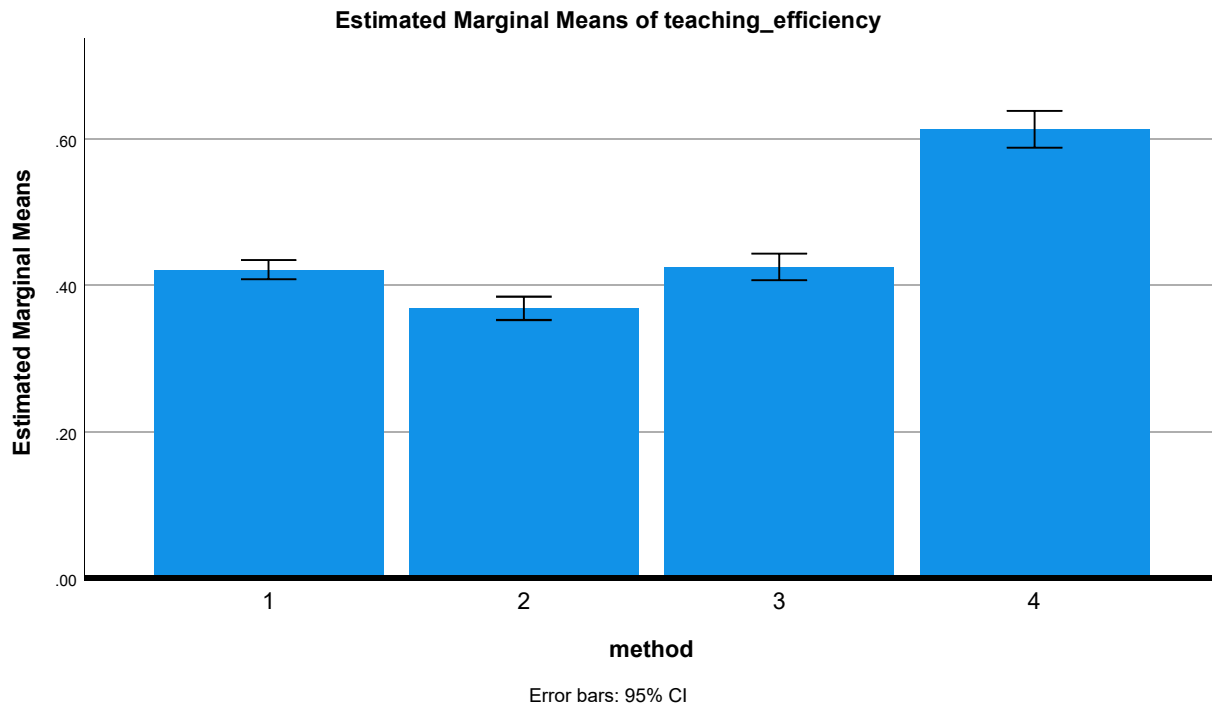

```
GLM A4 B4 C4 D4
  /WSFACTOR=method 4 Polynomial
  /MEASURE=teaching_efficiency
  /METHOD=SSTYPE(3)
  /PLOT=PROFILE(method) TYPE=BAR ERRORBAR=CI MEANREFERENCE=NO
  /EMMEANS=TABLES(method) COMPARE ADJ(LSD)
  /PRINT=DESCRIPTIVE
  /CRITERIA=ALPHA(.05)
  /WSDESIGN=method.
```

### General Linear Model

## Within-Subjects Factors

Measure: teaching\_efficiency

| method | Dependent<br>Variable |
|--------|-----------------------|
| 1      | A4                    |
| 2      | B4                    |
| 3      | C4                    |
| 4      | D4                    |

## Descriptive Statistics

|    | Mean  | Std. Deviation | N   |
|----|-------|----------------|-----|
| A4 | .3758 | .17308         | 380 |
| B4 | .2697 | .06078         | 380 |
| C4 | .3317 | .06381         | 380 |
| D4 | .3165 | .07666         | 380 |

## Multivariate Tests<sup>a</sup>

| Effect |                    | Value | F                    | Hypothesis df | Error df | Sig. |
|--------|--------------------|-------|----------------------|---------------|----------|------|
| method | Pillai's Trace     | .830  | 614.344 <sup>b</sup> | 3.000         | 377.000  | .000 |
|        | Wilks' Lambda      | .170  | 614.344 <sup>b</sup> | 3.000         | 377.000  | .000 |
|        | Hotelling's Trace  | 4.889 | 614.344 <sup>b</sup> | 3.000         | 377.000  | .000 |
|        | Roy's Largest Root | 4.889 | 614.344 <sup>b</sup> | 3.000         | 377.000  | .000 |

a. Design: Intercept  
Within Subjects Design: method

b. Exact statistic



### Mauchly's Test of Sphericity<sup>a</sup>

Measure: teaching\_efficiency

| Within Subjects Effect | Mauchly's W | Approx. Chi-Square | df | Sig. | Epsilon <sup>b</sup><br>Greenhouse-Geisser |
|------------------------|-------------|--------------------|----|------|--------------------------------------------|
| method                 | .031        | 1315.182           | 5  | .000 | .392                                       |

### Mauchly's Test of Sphericity<sup>a</sup>

Measure: teaching\_efficiency

| Within Subjects Effect | Epsilon <sup>b</sup> |             |
|------------------------|----------------------|-------------|
|                        | Huynh-Feldt          | Lower-bound |
| method                 | .392                 | .333        |

Tests the null hypothesis that the error covariance matrix of the orthonormalized transformed dependent variables is proportional to an identity matrix.

a. Design: Intercept

Within Subjects Design: method

b. May be used to adjust the degrees of freedom for the averaged tests of significance. Corrected tests are displayed in the Tests of Within-Subjects Effects table.

### Tests of Within-Subjects Effects

Measure: teaching\_efficiency

| Source        |                    | Type III Sum of Squares | df      | Mean Square | F       |
|---------------|--------------------|-------------------------|---------|-------------|---------|
| method        | Sphericity Assumed | 2.186                   | 3       | .729        | 118.650 |
|               | Greenhouse-Geisser | 2.186                   | 1.175   | 1.861       | 118.650 |
|               | Huynh-Feldt        | 2.186                   | 1.176   | 1.858       | 118.650 |
|               | Lower-bound        | 2.186                   | 1.000   | 2.186       | 118.650 |
| Error(method) | Sphericity Assumed | 6.982                   | 1137    | .006        |         |
|               | Greenhouse-Geisser | 6.982                   | 445.249 | .016        |         |
|               | Huynh-Feldt        | 6.982                   | 445.806 | .016        |         |
|               | Lower-bound        | 6.982                   | 379.000 | .018        |         |

### Tests of Within-Subjects Effects

Measure: teaching\_efficiency

| Source        |                    | Sig. |
|---------------|--------------------|------|
| method        | Sphericity Assumed | .000 |
|               | Greenhouse-Geisser | .000 |
|               | Huynh-Feldt        | .000 |
|               | Lower-bound        | .000 |
| Error(method) | Sphericity Assumed |      |
|               | Greenhouse-Geisser |      |
|               | Huynh-Feldt        |      |
|               | Lower-bound        |      |

### Tests of Within-Subjects Contrasts

Measure: teaching\_efficiency

| Source        | method    | Type III Sum of Squares | df  | Mean Square | F        | Sig. |
|---------------|-----------|-------------------------|-----|-------------|----------|------|
| method        | Linear    | .255                    | 1   | .255        | 25.974   | .000 |
|               | Quadratic | .788                    | 1   | .788        | 101.347  | .000 |
|               | Cubic     | 1.143                   | 1   | 1.143       | 1371.014 | .000 |
| Error(method) | Linear    | 3.721                   | 379 | .010        |          |      |
|               | Quadratic | 2.945                   | 379 | .008        |          |      |
|               | Cubic     | .316                    | 379 | .001        |          |      |

### Tests of Between-Subjects Effects

Measure: teaching\_efficiency

Transformed Variable: Average

| Source    | Type III Sum of Squares | df  | Mean Square | F        | Sig. |
|-----------|-------------------------|-----|-------------|----------|------|
| Intercept | 158.988                 | 1   | 158.988     | 6314.703 | .000 |
| Error     | 9.542                   | 379 | .025        |          |      |

### Estimated Marginal Means

method

## Estimates

Measure: teaching\_efficiency

| method | Mean | Std. Error | 95% Confidence Interval |             |
|--------|------|------------|-------------------------|-------------|
|        |      |            | Lower Bound             | Upper Bound |
| 1      | .376 | .009       | .358                    | .393        |
| 2      | .270 | .003       | .264                    | .276        |
| 3      | .332 | .003       | .325                    | .338        |
| 4      | .317 | .004       | .309                    | .324        |

## Pairwise Comparisons

Measure: teaching\_efficiency

| (I) method | (J) method | Mean Difference (I-J) | Std. Error | Sig. <sup>b</sup> | 95% Confidence Interval for Difference <sup>b</sup> |             |
|------------|------------|-----------------------|------------|-------------------|-----------------------------------------------------|-------------|
|            |            |                       |            |                   | Lower Bound                                         | Upper Bound |
| 1          | 2          | .106 <sup>*</sup>     | .008       | .000              | .091                                                | .121        |
|            | 3          | .044 <sup>*</sup>     | .008       | .000              | .028                                                | .061        |
|            | 4          | .059 <sup>*</sup>     | .007       | .000              | .045                                                | .073        |
| 2          | 1          | -.106 <sup>*</sup>    | .008       | .000              | -.121                                               | -.091       |
|            | 3          | -.062 <sup>*</sup>    | .002       | .000              | -.066                                               | -.058       |
|            | 4          | -.047 <sup>*</sup>    | .002       | .000              | -.052                                               | -.042       |
| 3          | 1          | -.044 <sup>*</sup>    | .008       | .000              | -.061                                               | -.028       |
|            | 2          | .062 <sup>*</sup>     | .002       | .000              | .058                                                | .066        |
|            | 4          | .015 <sup>*</sup>     | .002       | .000              | .011                                                | .019        |
| 4          | 1          | -.059 <sup>*</sup>    | .007       | .000              | -.073                                               | -.045       |
|            | 2          | .047 <sup>*</sup>     | .002       | .000              | .042                                                | .052        |
|            | 3          | -.015 <sup>*</sup>    | .002       | .000              | -.019                                               | -.011       |

Based on estimated marginal means

\*. The mean difference is significant at the .05 level.

b. Adjustment for multiple comparisons: Least Significant Difference (equivalent to no adjustments).

### Multivariate Tests

|                    | Value | F                    | Hypothesis df | Error df | Sig. |
|--------------------|-------|----------------------|---------------|----------|------|
| Pillai's trace     | .830  | 614.344 <sup>a</sup> | 3.000         | 377.000  | .000 |
| Wilks' lambda      | .170  | 614.344 <sup>a</sup> | 3.000         | 377.000  | .000 |
| Hotelling's trace  | 4.889 | 614.344 <sup>a</sup> | 3.000         | 377.000  | .000 |
| Roy's largest root | 4.889 | 614.344 <sup>a</sup> | 3.000         | 377.000  | .000 |

Each F tests the multivariate effect of method. These tests are based on the linearly independent pairwise comparisons among the estimated marginal means.

a. Exact statistic

### Profile Plots

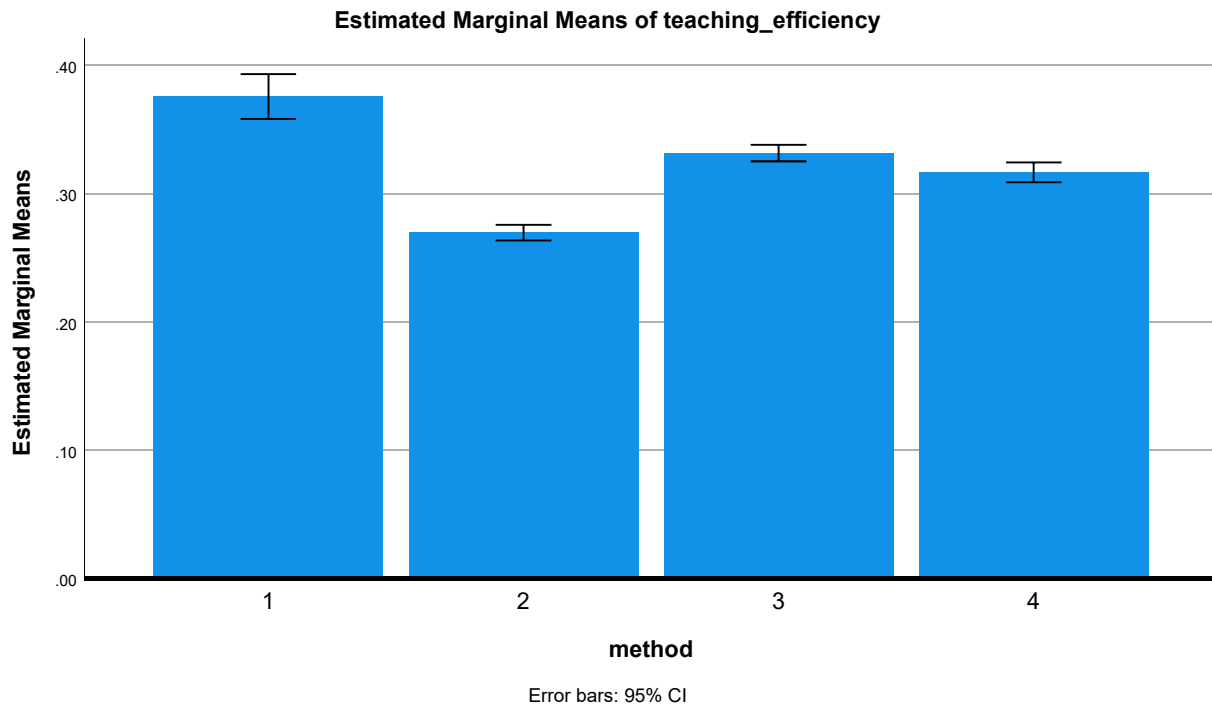

```
GLM A5 B5 C5 D5
  /WSFACTOR=method 4 Polynomial
  /MEASURE=teaching_efficiency
  /METHOD=SSTYPE(3)
  /PLOT=PROFILE(method) TYPE=BAR ERRORBAR=CI MEANREFERENCE=NO
  /EMMEANS=TABLES(method) COMPARE ADJ(LSD)
  /PRINT=DESCRIPTIVE
  /CRITERIA=ALPHA(.05)
  /WSDESIGN=method.
```

### General Linear Model

## Within-Subjects Factors

Measure: teaching\_efficiency

| method | Dependent<br>Variable |
|--------|-----------------------|
| 1      | A5                    |
| 2      | B5                    |
| 3      | C5                    |
| 4      | D5                    |

## Descriptive Statistics

|    | Mean  | Std. Deviation | N   |
|----|-------|----------------|-----|
| A5 | .1684 | .04293         | 380 |
| B5 | .1840 | .04288         | 380 |
| C5 | .1644 | .07566         | 380 |
| D5 | .2643 | .04270         | 380 |

## Multivariate Tests<sup>a</sup>

| Effect |                    | Value | F                    | Hypothesis df | Error df | Sig. |
|--------|--------------------|-------|----------------------|---------------|----------|------|
| method | Pillai's Trace     | .807  | 526.359 <sup>b</sup> | 3.000         | 377.000  | .000 |
|        | Wilks' Lambda      | .193  | 526.359 <sup>b</sup> | 3.000         | 377.000  | .000 |
|        | Hotelling's Trace  | 4.189 | 526.359 <sup>b</sup> | 3.000         | 377.000  | .000 |
|        | Roy's Largest Root | 4.189 | 526.359 <sup>b</sup> | 3.000         | 377.000  | .000 |

a. Design: Intercept  
Within Subjects Design: method

b. Exact statistic

### Mauchly's Test of Sphericity<sup>a</sup>

Measure: teaching\_efficiency

| Within Subjects Effect | Mauchly's W | Approx. Chi-Square | df | Sig. | Epsilon <sup>b</sup><br>Greenhouse-Geisser |
|------------------------|-------------|--------------------|----|------|--------------------------------------------|
| method                 | .194        | 619.793            | 5  | .000 | .504                                       |

### Mauchly's Test of Sphericity<sup>a</sup>

Measure: teaching\_efficiency

| Within Subjects Effect | Epsilon <sup>b</sup> |             |
|------------------------|----------------------|-------------|
|                        | Huynh-Feldt          | Lower-bound |
| method                 | .506                 | .333        |

Tests the null hypothesis that the error covariance matrix of the orthonormalized transformed dependent variables is proportional to an identity matrix.

a. Design: Intercept

Within Subjects Design: method

b. May be used to adjust the degrees of freedom for the averaged tests of significance. Corrected tests are displayed in the Tests of Within-Subjects Effects table.

### Tests of Within-Subjects Effects

Measure: teaching\_efficiency

| Source        |                    | Type III Sum of Squares | df      | Mean Square | F       |
|---------------|--------------------|-------------------------|---------|-------------|---------|
| method        | Sphericity Assumed | 2.498                   | 3       | .833        | 251.043 |
|               | Greenhouse-Geisser | 2.498                   | 1.513   | 1.651       | 251.043 |
|               | Huynh-Feldt        | 2.498                   | 1.518   | 1.645       | 251.043 |
|               | Lower-bound        | 2.498                   | 1.000   | 2.498       | 251.043 |
| Error(method) | Sphericity Assumed | 3.771                   | 1137    | .003        |         |
|               | Greenhouse-Geisser | 3.771                   | 573.476 | .007        |         |
|               | Huynh-Feldt        | 3.771                   | 575.286 | .007        |         |
|               | Lower-bound        | 3.771                   | 379.000 | .010        |         |

### Tests of Within-Subjects Effects

Measure: teaching\_efficiency

| Source        |                    | Sig. |
|---------------|--------------------|------|
| method        | Sphericity Assumed | .000 |
|               | Greenhouse-Geisser | .000 |
|               | Huynh-Feldt        | .000 |
|               | Lower-bound        | .000 |
| Error(method) | Sphericity Assumed |      |
|               | Greenhouse-Geisser |      |
|               | Huynh-Feldt        |      |
|               | Lower-bound        |      |

### Tests of Within-Subjects Contrasts

Measure: teaching\_efficiency

| Source        | method    | Type III Sum of Squares | df  | Mean Square | F       | Sig. |
|---------------|-----------|-------------------------|-----|-------------|---------|------|
| method        | Linear    | 1.366                   | 1   | 1.366       | 766.237 | .000 |
|               | Quadratic | .677                    | 1   | .677        | 212.853 | .000 |
|               | Cubic     | .455                    | 1   | .455        | 91.267  | .000 |
| Error(method) | Linear    | .676                    | 379 | .002        |         |      |
|               | Quadratic | 1.205                   | 379 | .003        |         |      |
|               | Cubic     | 1.890                   | 379 | .005        |         |      |

### Tests of Between-Subjects Effects

Measure: teaching\_efficiency

Transformed Variable: Average

| Source    | Type III Sum of Squares | df  | Mean Square | F         | Sig. |
|-----------|-------------------------|-----|-------------|-----------|------|
| Intercept | 57.973                  | 1   | 57.973      | 45312.098 | .000 |
| Error     | .485                    | 379 | .001        |           |      |

### Estimated Marginal Means

method

## Estimates

Measure: teaching\_efficiency

| method | Mean | Std. Error | 95% Confidence Interval |             |
|--------|------|------------|-------------------------|-------------|
|        |      |            | Lower Bound             | Upper Bound |
| 1      | .168 | .002       | .164                    | .173        |
| 2      | .184 | .002       | .180                    | .188        |
| 3      | .164 | .004       | .157                    | .172        |
| 4      | .264 | .002       | .260                    | .269        |

## Pairwise Comparisons

Measure: teaching\_efficiency

| (I) method | (J) method | Mean Difference (I-J) | Std. Error | Sig. <sup>b</sup> | 95% Confidence Interval for Difference <sup>b</sup> |             |
|------------|------------|-----------------------|------------|-------------------|-----------------------------------------------------|-------------|
|            |            |                       |            |                   | Lower Bound                                         | Upper Bound |
| 1          | 2          | -.016 <sup>*</sup>    | .002       | .000              | -.019                                               | -.012       |
|            | 3          | .004                  | .005       | .459              | -.007                                               | .015        |
|            | 4          | -.096 <sup>*</sup>    | .003       | .000              | -.101                                               | -.091       |
| 2          | 1          | .016 <sup>*</sup>     | .002       | .000              | .012                                                | .019        |
|            | 3          | .020 <sup>*</sup>     | .005       | .000              | .009                                                | .030        |
|            | 4          | -.080 <sup>*</sup>    | .002       | .000              | -.085                                               | -.076       |
| 3          | 1          | -.004                 | .005       | .459              | -.015                                               | .007        |
|            | 2          | -.020 <sup>*</sup>    | .005       | .000              | -.030                                               | -.009       |
|            | 4          | -.100 <sup>*</sup>    | .005       | .000              | -.111                                               | -.089       |
| 4          | 1          | .096 <sup>*</sup>     | .003       | .000              | .091                                                | .101        |
|            | 2          | .080 <sup>*</sup>     | .002       | .000              | .076                                                | .085        |
|            | 3          | .100 <sup>*</sup>     | .005       | .000              | .089                                                | .111        |

Based on estimated marginal means

\*. The mean difference is significant at the .05 level.

b. Adjustment for multiple comparisons: Least Significant Difference (equivalent to no adjustments).



### Multivariate Tests

|                    | Value | F                    | Hypothesis df | Error df | Sig. |
|--------------------|-------|----------------------|---------------|----------|------|
| Pillai's trace     | .807  | 526.359 <sup>a</sup> | 3.000         | 377.000  | .000 |
| Wilks' lambda      | .193  | 526.359 <sup>a</sup> | 3.000         | 377.000  | .000 |
| Hotelling's trace  | 4.189 | 526.359 <sup>a</sup> | 3.000         | 377.000  | .000 |
| Roy's largest root | 4.189 | 526.359 <sup>a</sup> | 3.000         | 377.000  | .000 |

Each F tests the multivariate effect of method. These tests are based on the linearly independent pairwise comparisons among the estimated marginal means.

a. Exact statistic

### Profile Plots

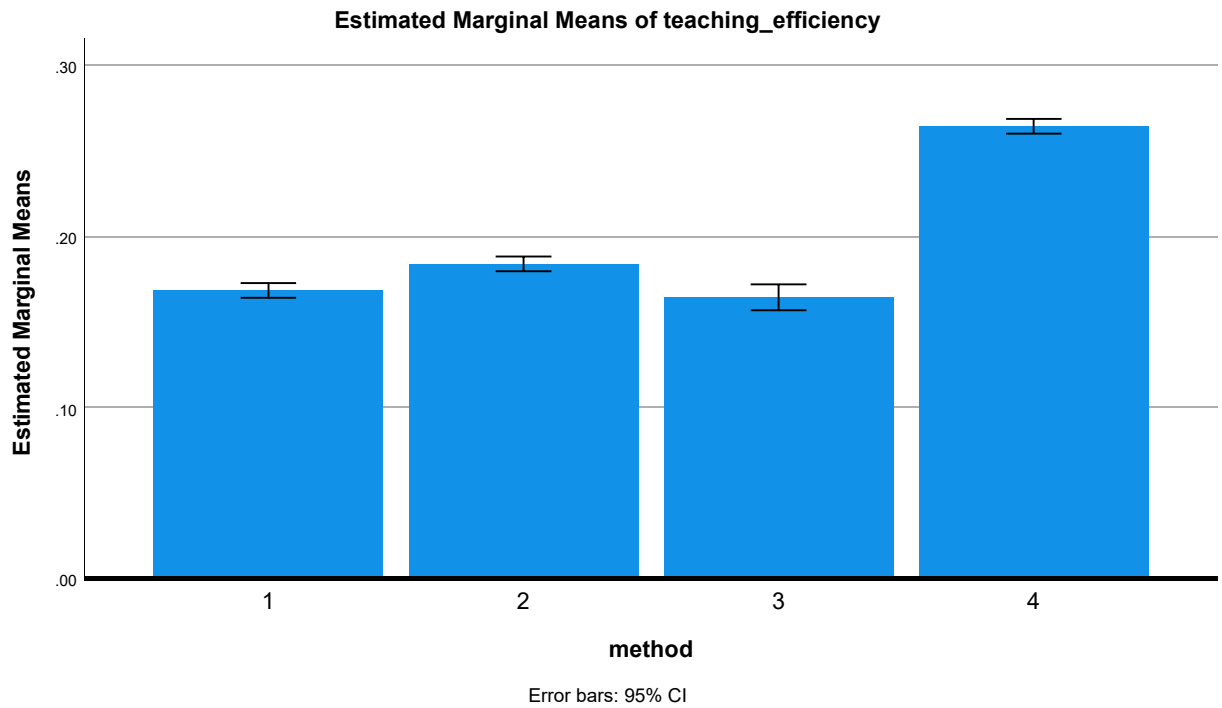

Supplement: Supplementary file 5 [file teaching_efficiency.pdf]
